# Supplementary material for: Invariant-mass and fractional-energy dependence of inclusive production of di-hadrons in $e^+e^-$ annihilation at $\sqrt{s}=$ 10.58 GeV
Source: arXiv:1706.08348 source file (2017-08-08)
Supplement: Supplementary file 1 [file supplement.tex]

%
%    Template for Belle journal submissions
%
%
% TeX'ing this file requires that you have AMS-LaTeX 2.0 installed
% as well as the rest of the prerequisites for REVTeX 4.0
%
% See the REVTeX 4 README file
% It also requires running BibTeX. The commands are as follows:
%
%  1)  latex apssamp.tex
%  2)  bibtex apssamp
%  3)  latex apssamp.tex
%  4)  latex apssamp.tex
%
%%% Use this for e-print submission 
%%% You also need to do the following:
%%%   * Comment out widetext, use eqnarray and \nonumber 
%%%     (for the first line) for eq:likelihood
%%%   * Change the figure size to 0.6
%%%   * Put preprint numbers and the Belle logo
%\documentclass[aps,prl,preprint,tightenlines,superscriptaddress,showpacs,byrevtex]{revtex4}
%
%%% Use this for PRL submission 
%%% You also need to do the following:
%%%   * Comment out widetext, use eqnarray and \nonumber 
%%%     (for the first line) for eq:likelihood
%%%   * Change the figure size to 0.6
%%%   * Comment out preprint numbers and the Belle logo
%\documentclass[aps,prl,preprint,superscriptaddress,showpacs,byrevtex]{revtex4}%
%%% Double-column style
%%% You also need to do the following:
%%%   * Use widetext for eq:likelihood, comment out \nonumber
%%%   * Change the figure size appropriately (should be less than 0.5)
%%%   * Comment out preprint numbers and the Belle logo
\RequirePackage{lineno} \setlength{\linenumbersep}{4pt}
\documentclass[aps,prd,twocolumn,superscriptaddress,preprintnumbers,amsmath,amssymb,tightenlines,floatfix]{revtex4-1}
%

% Some other (several out of many) possibilities
%\documentclass[preprint,aps]{revtex4}
%\documentclass[preprint,aps,draft]{revtex4}
\usepackage{graphicx} % Include figure files
\usepackage{dcolumn}  % Align table columns on decimal point
\usepackage{rotating}
\usepackage{epstopdf}
\usepackage{hyperref}
\graphicspath{{ps}}

%\renewcommand{\arraystretch}{1.1}

% Belle authors Checklist:
% 1) Title; use \\ to break title over several lines.
% 2) Author list
% 3) Abstract
% 4) pacs numbers, for PRL, PRD
% 5) Body

\begin{document}

%\vspace*{-3\baselineskip}
%\resizebox{!}{3cm}{\includegraphics{belle.eps}}

\preprint{\vbox{% \hbox{Version 1.9 }
    \hbox{Belle DRAFT {\it 2017-13}}
    \hbox{KEK DRAFT {\it 2017-09}}
       %                 \hbox{Intended for {\it PRD}}
       %                 \hbox{Author: R.Seidl}
       %                 \hbox{Committee: W. Jacobs(chair),}
       %                 \hbox{G. Schnell, M. Niiyama, }
  %		               \hbox{BN 1425}
}}

\title{ \quad\\[1.0cm]Supplemental figures to the publication: Invariant-mass and fractional-energy dependence of inclusive production of di-hadrons in $e^+e^-$ annihilation at $\sqrt{s}=$ 10.58~GeV }
\include{pub490}
%\collaboration{The Belle Collaboration}
%\author{Author}\affiliation{affiliation}
%\collaboration{The Belle Collaboration}
\noaffiliation
%% end author list
%\linenumbers
\begin{abstract}
This file collects various supplemental figures that would have made the main publication too unwieldy. In particular, the corresponding PID, acceptance and systematic uncertainty figures for the same-sign pion, pion-kaon and kaon pair cross sections are shown here. Also, the figures comparing those hadron combinations to various MC tunes and identifying the sources of some of the observed peaks are presented.
\end{abstract}

%\pacs{13.66.Bc,13.87.Fh,13.88.+e,14.20.Dh}

\maketitle

%%%% >>>> keep the final version single-spaced
%\tighten
%\tightenline
{\renewcommand{\thefootnote}{\fnsymbol{footnote}}}
\setcounter{footnote}{0}

\subsection{PID correction}
Figures \ref{fig:beforeafterpid2} to \ref{fig:beforeafterpid8192} display the effects of the PID correction for the same-sign hadron pairs as well as the opposite-sign pion-kaon and kaon pairs.
\begin{figure*}[th]
\begin{center}
\includegraphics[width=0.8\textwidth]{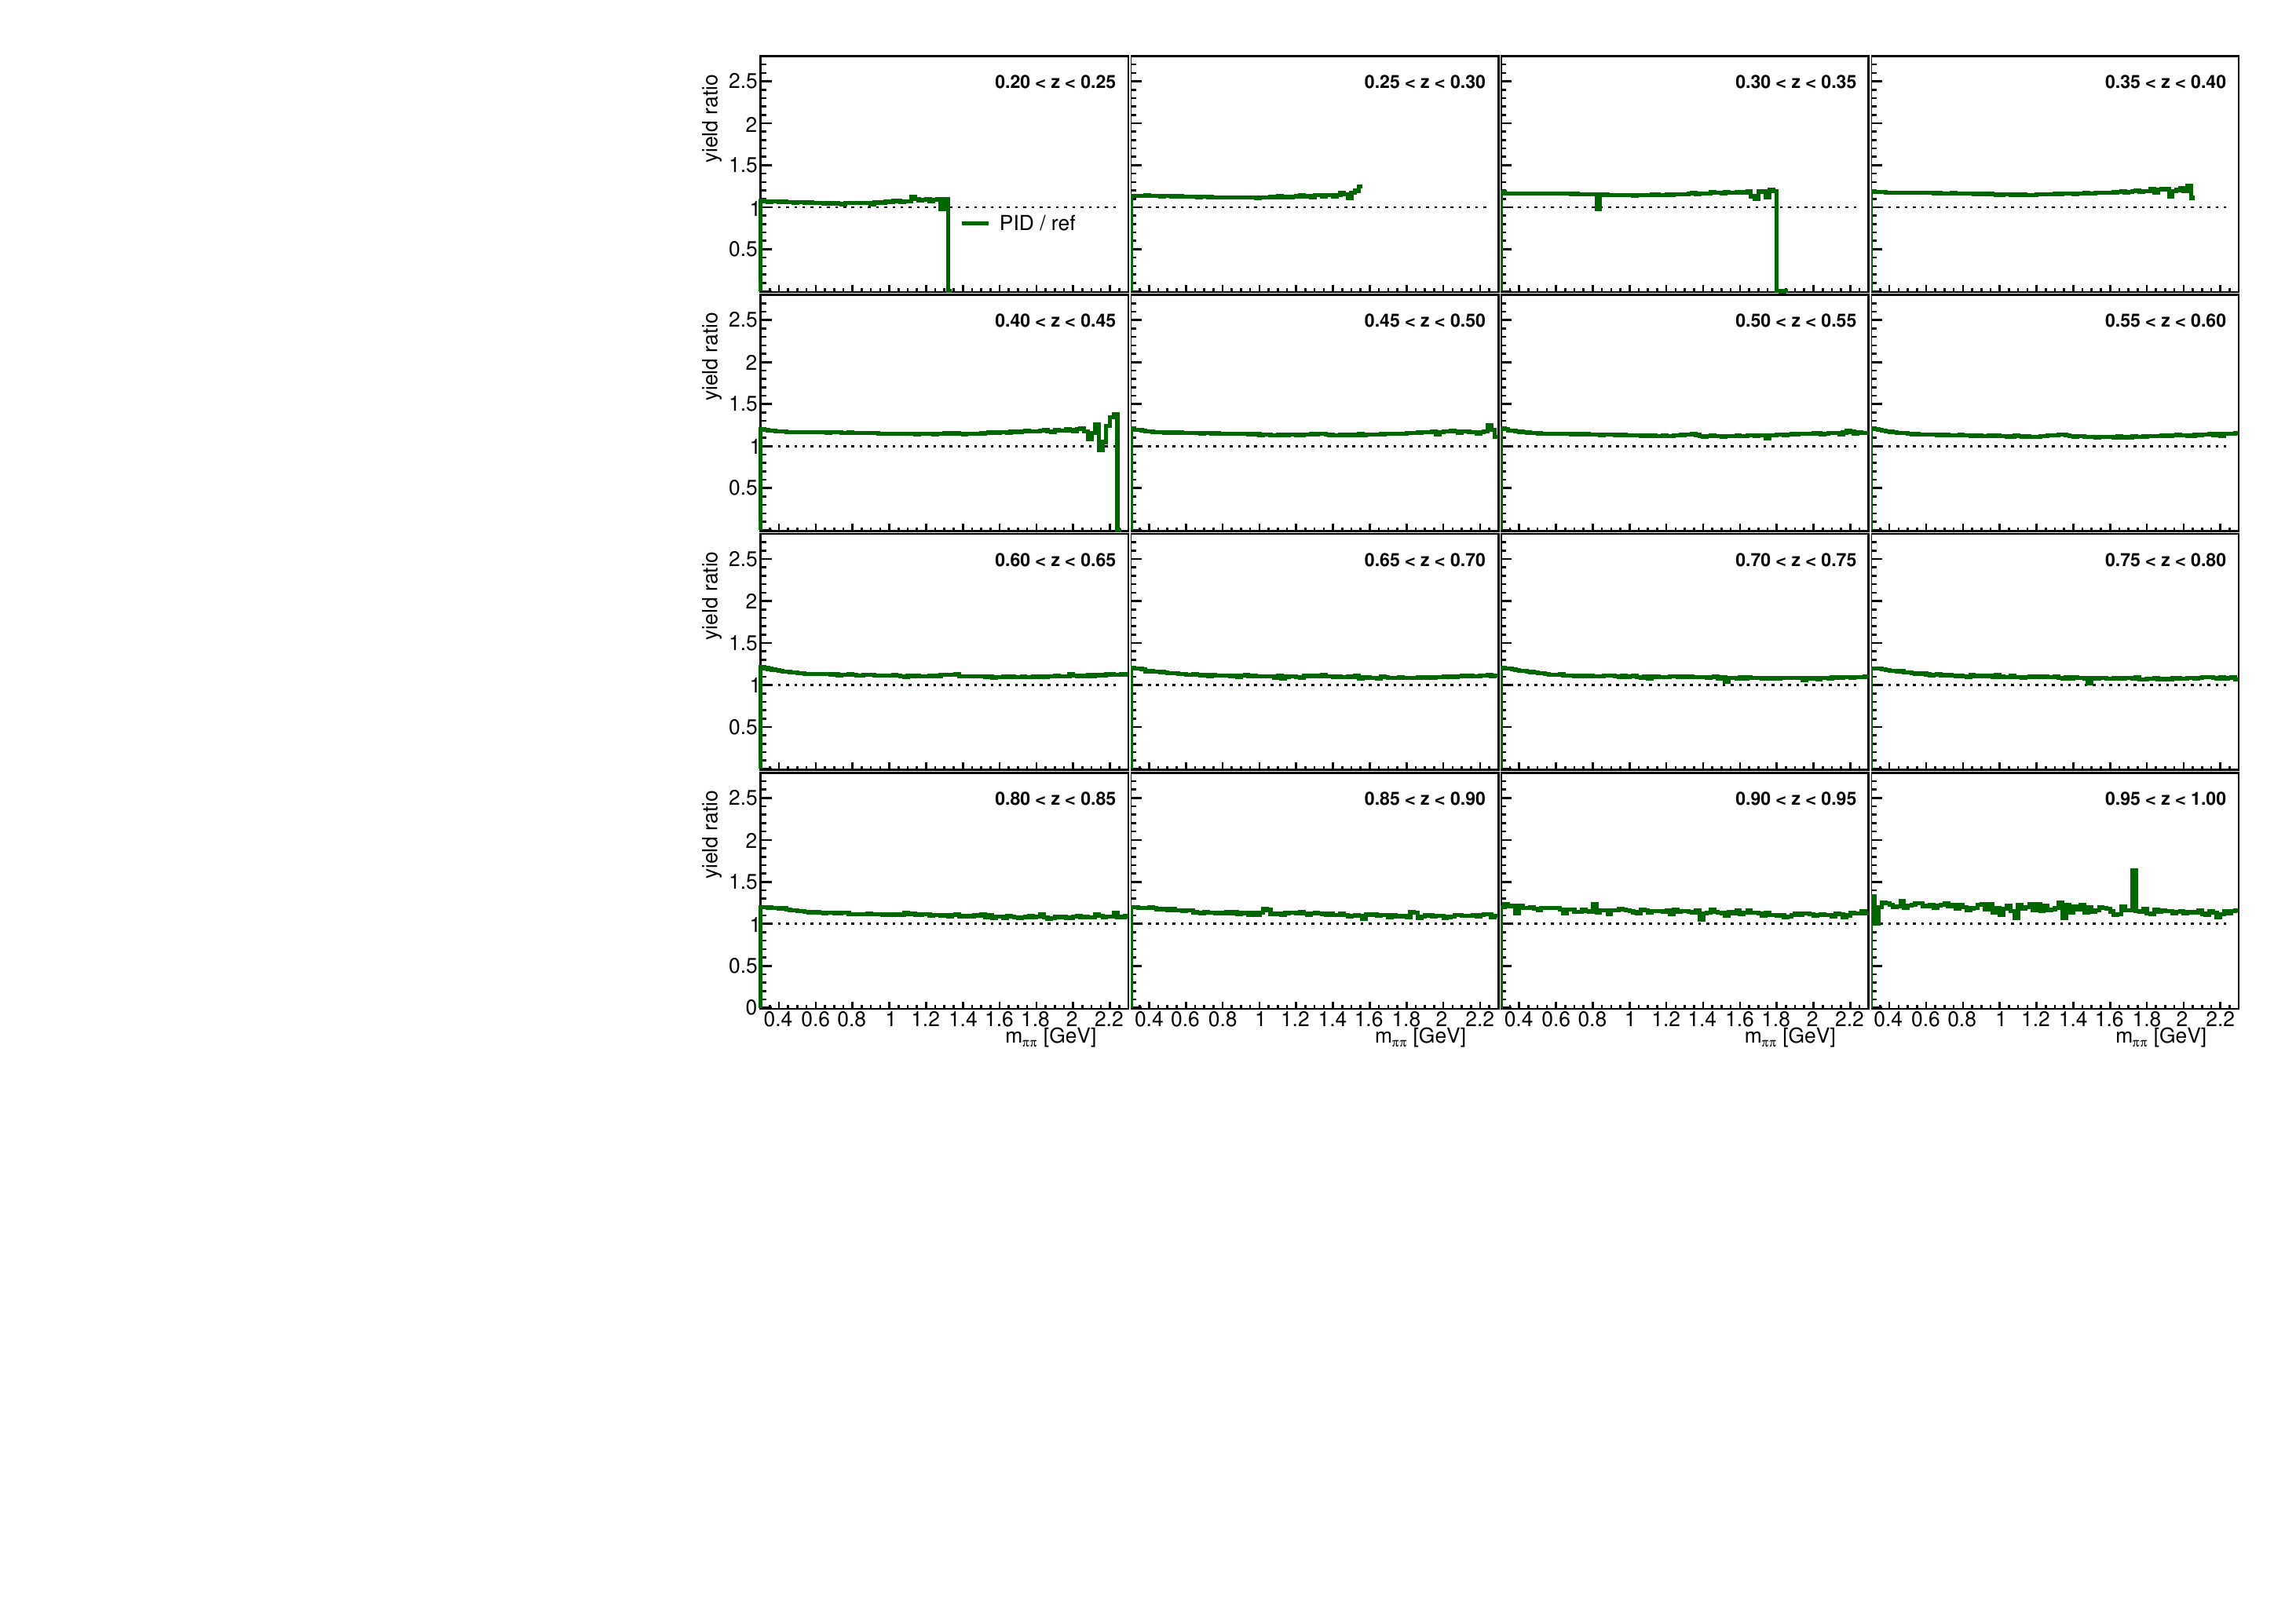} 
\caption{\label{fig:beforeafterpid2}Ratio of yields after to before applying the PID correction for $\pi^+\pi^+$ pairs as a function of $m_{\pi\pi}$ in bins of $z$. Structures are observed due to sharp resonances; at low $z$, the kinematical limits are evident.}
\end{center}
\end{figure*}
\begin{figure*}[th]
\begin{center}
\includegraphics[width=0.8\textwidth]{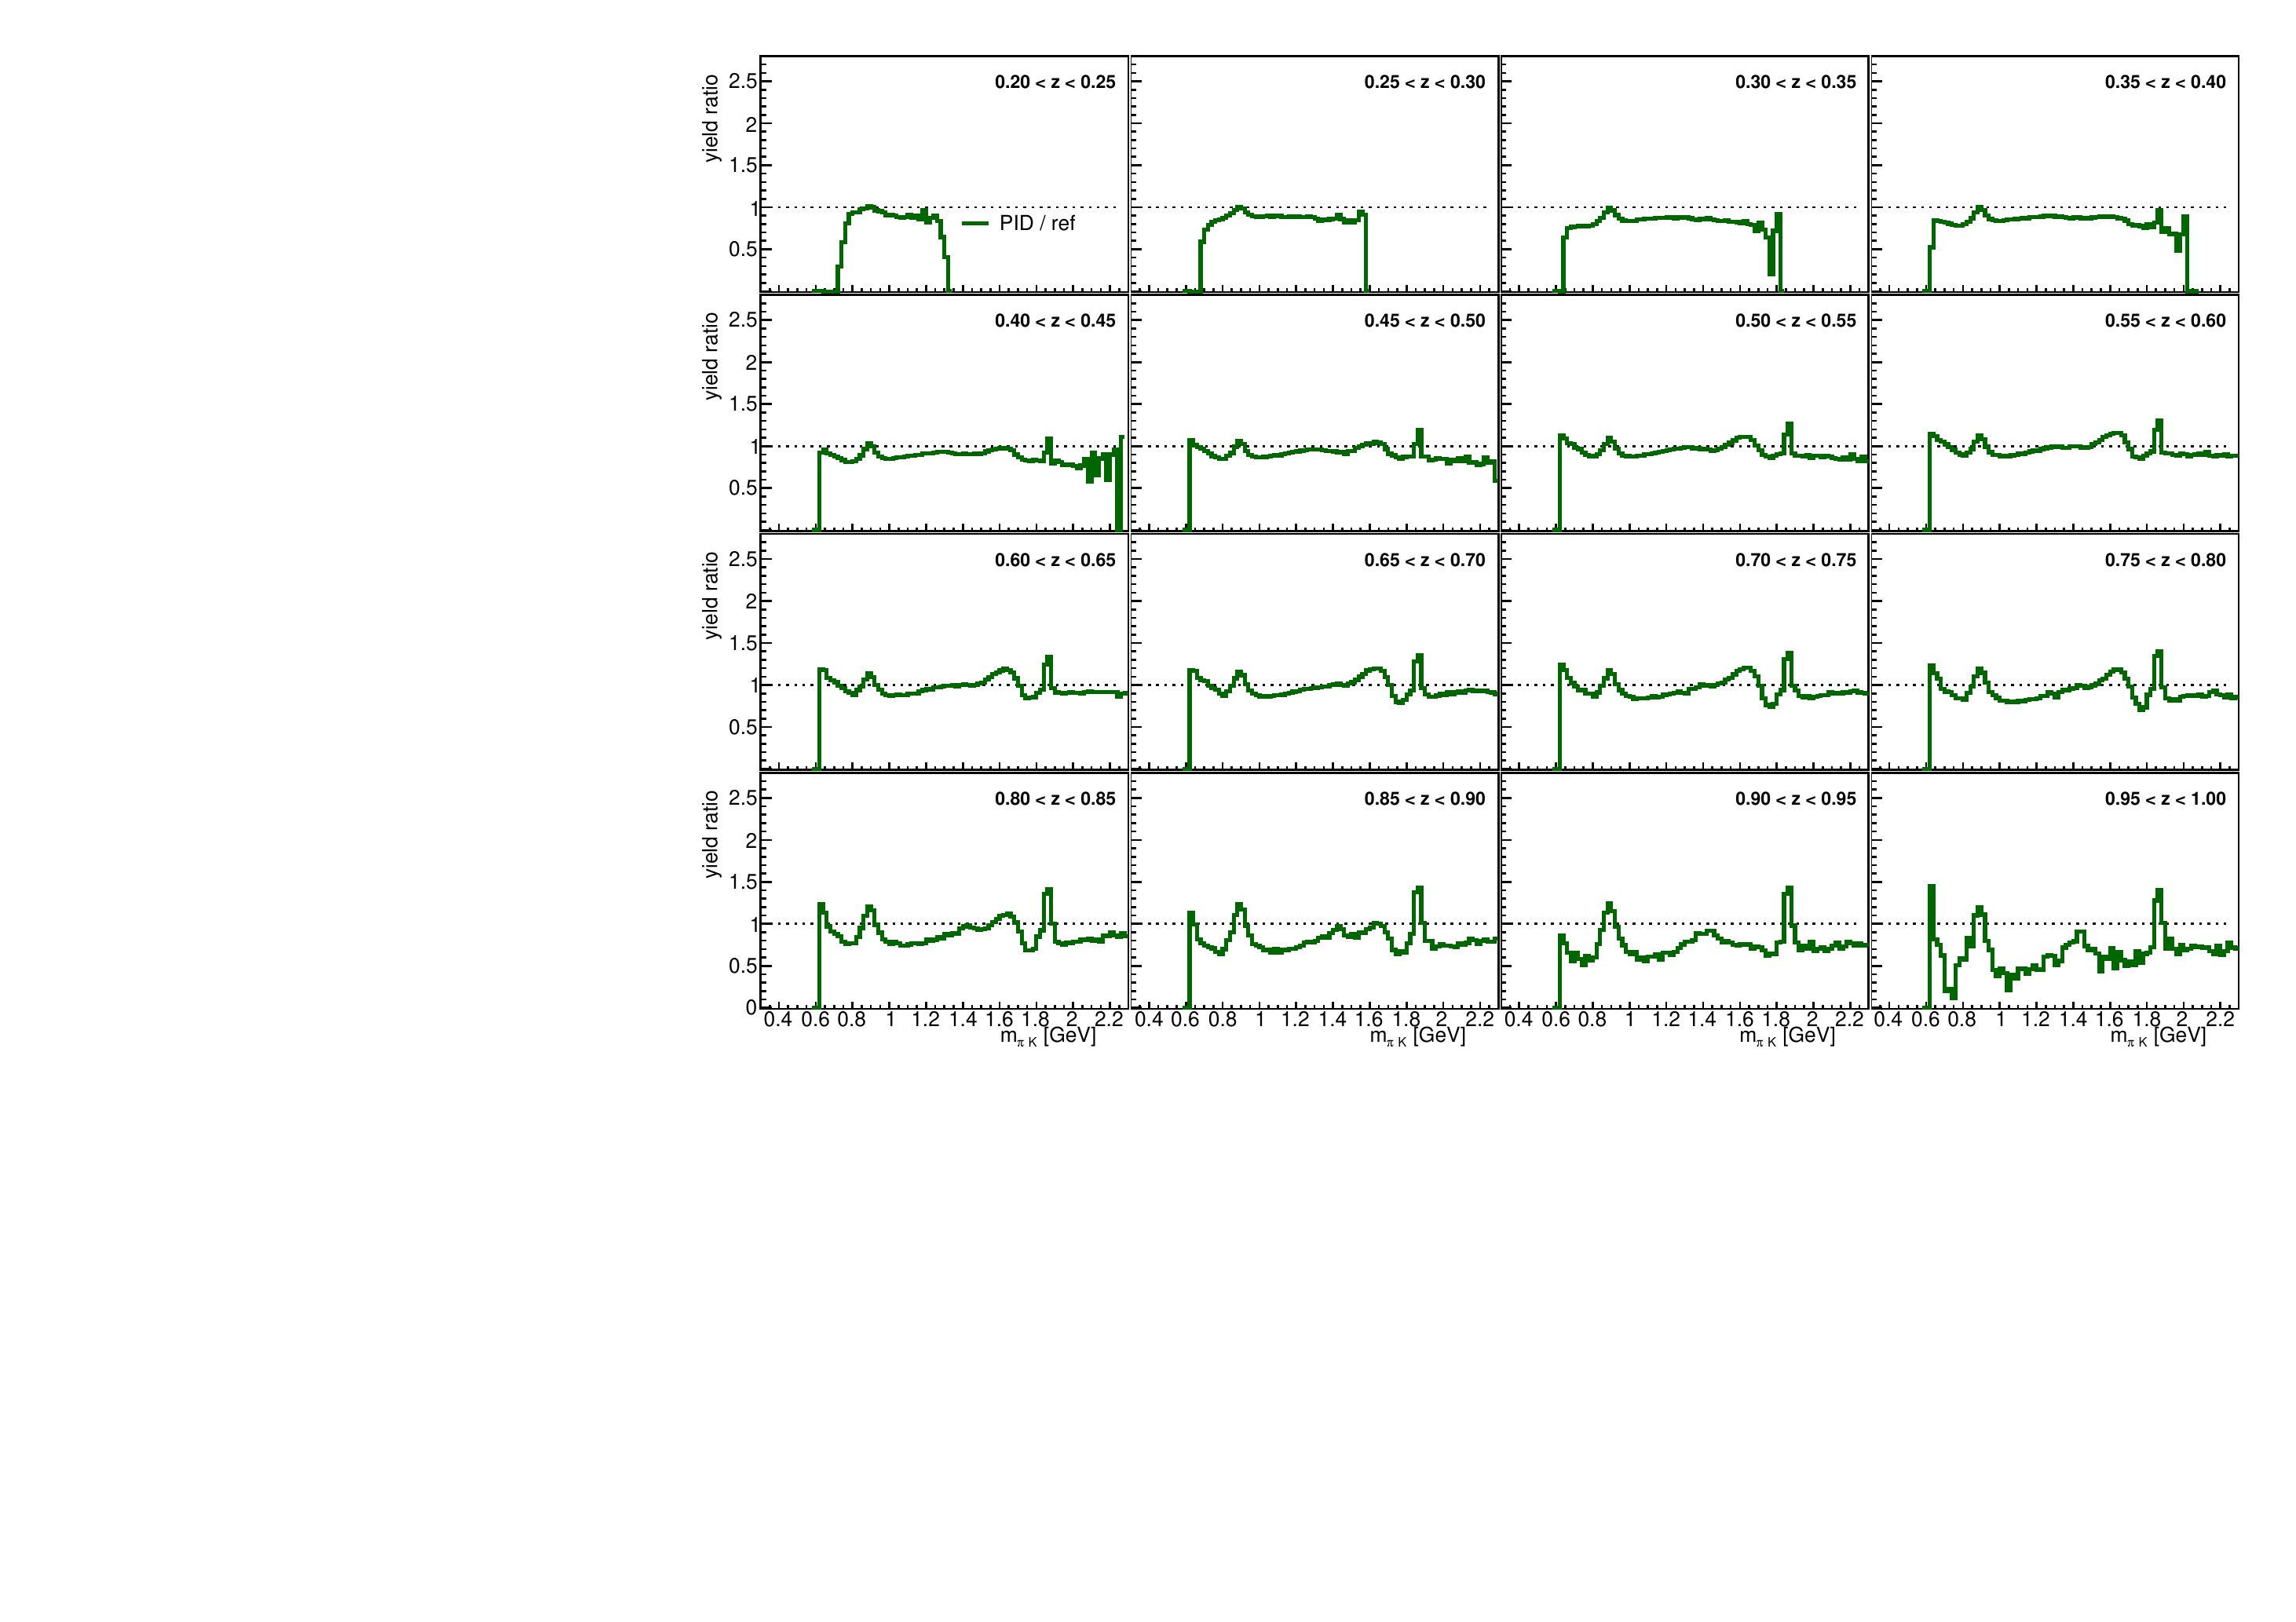} 
\caption{\label{fig:beforeafterpid16}Ratio of yields after to before applying the PID correction for  $\pi^+K^-$ pairs as a function of $m_{\pi K}$ in bins of $z$. Structures are observed due to sharp resonances; at low $z$, the kinematical limits are evident.}
\end{center}
\end{figure*}
\begin{figure*}[th]
\begin{center}
\includegraphics[width=0.8\textwidth]{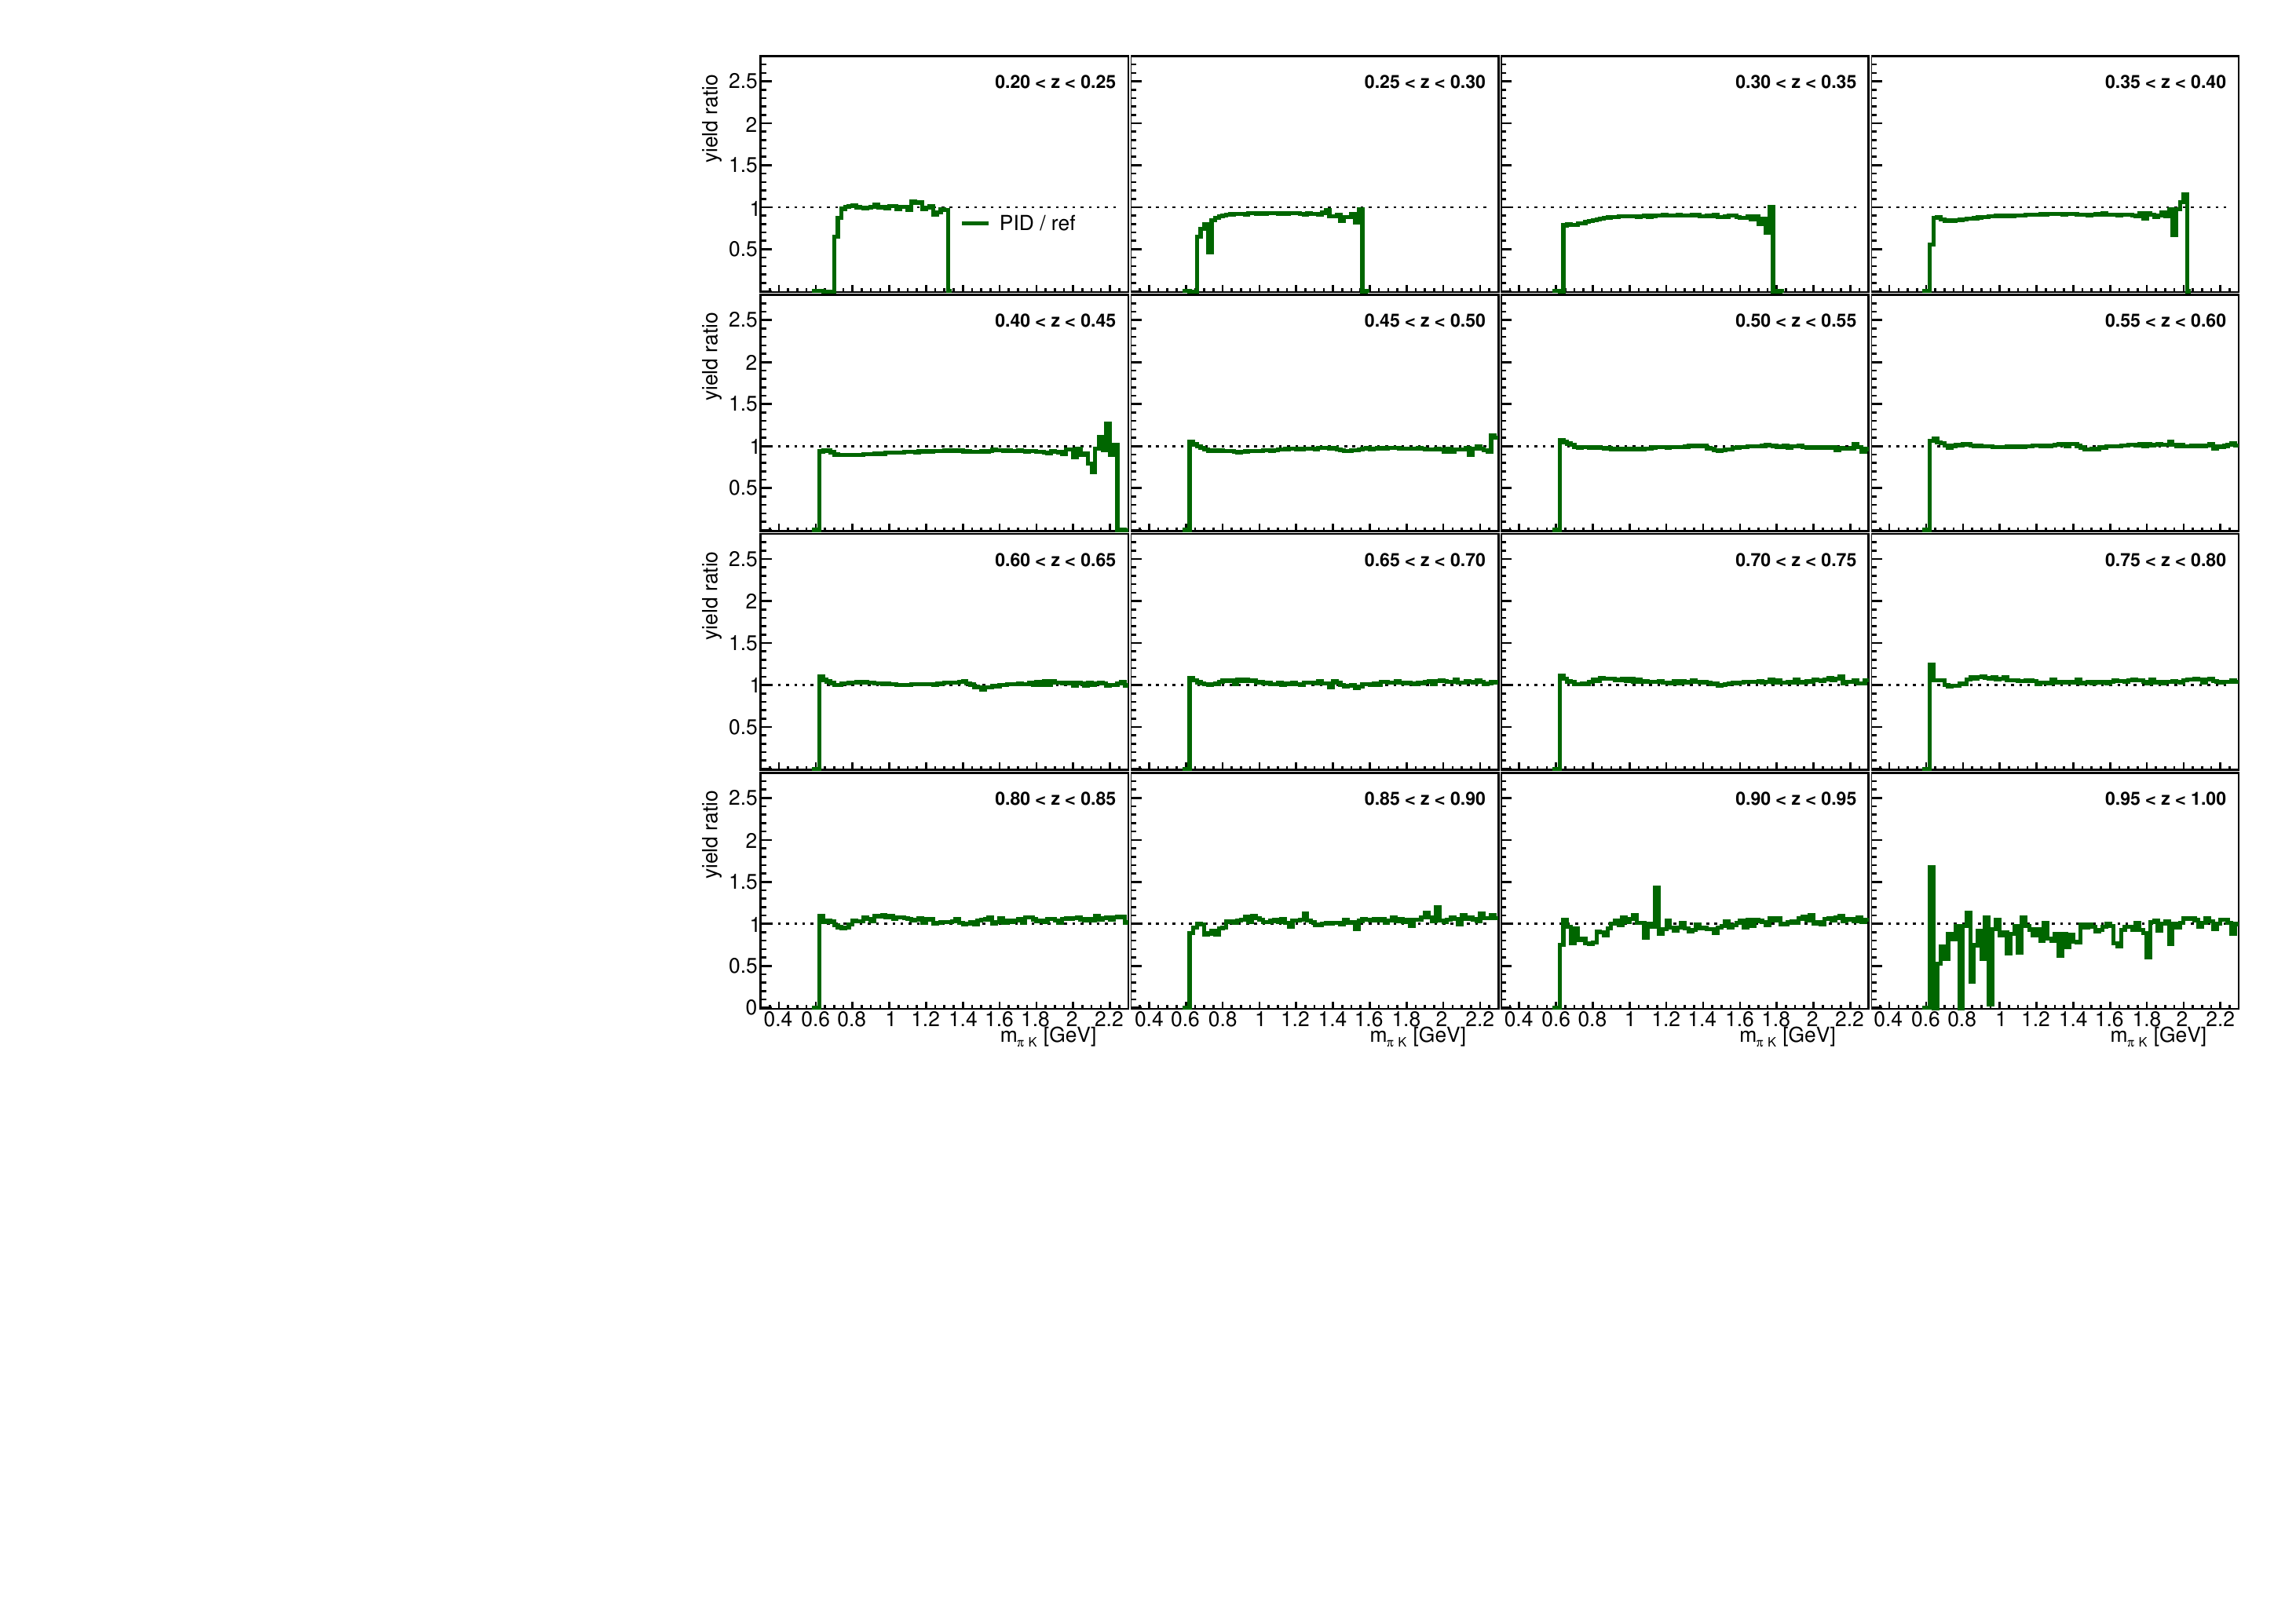} 
\caption{\label{fig:beforeafterpid32}Ratio of yields after to before applying the PID correction for  $\pi^+K^+$ pairs as a function of $m_{\pi K}$ in bins of $z$. Structures are observed due to sharp resonances; at low $z$, the kinematical limits are evident.}
\end{center}
\end{figure*}

\begin{figure*}[th]
\begin{center}
\includegraphics[width=0.8\textwidth]{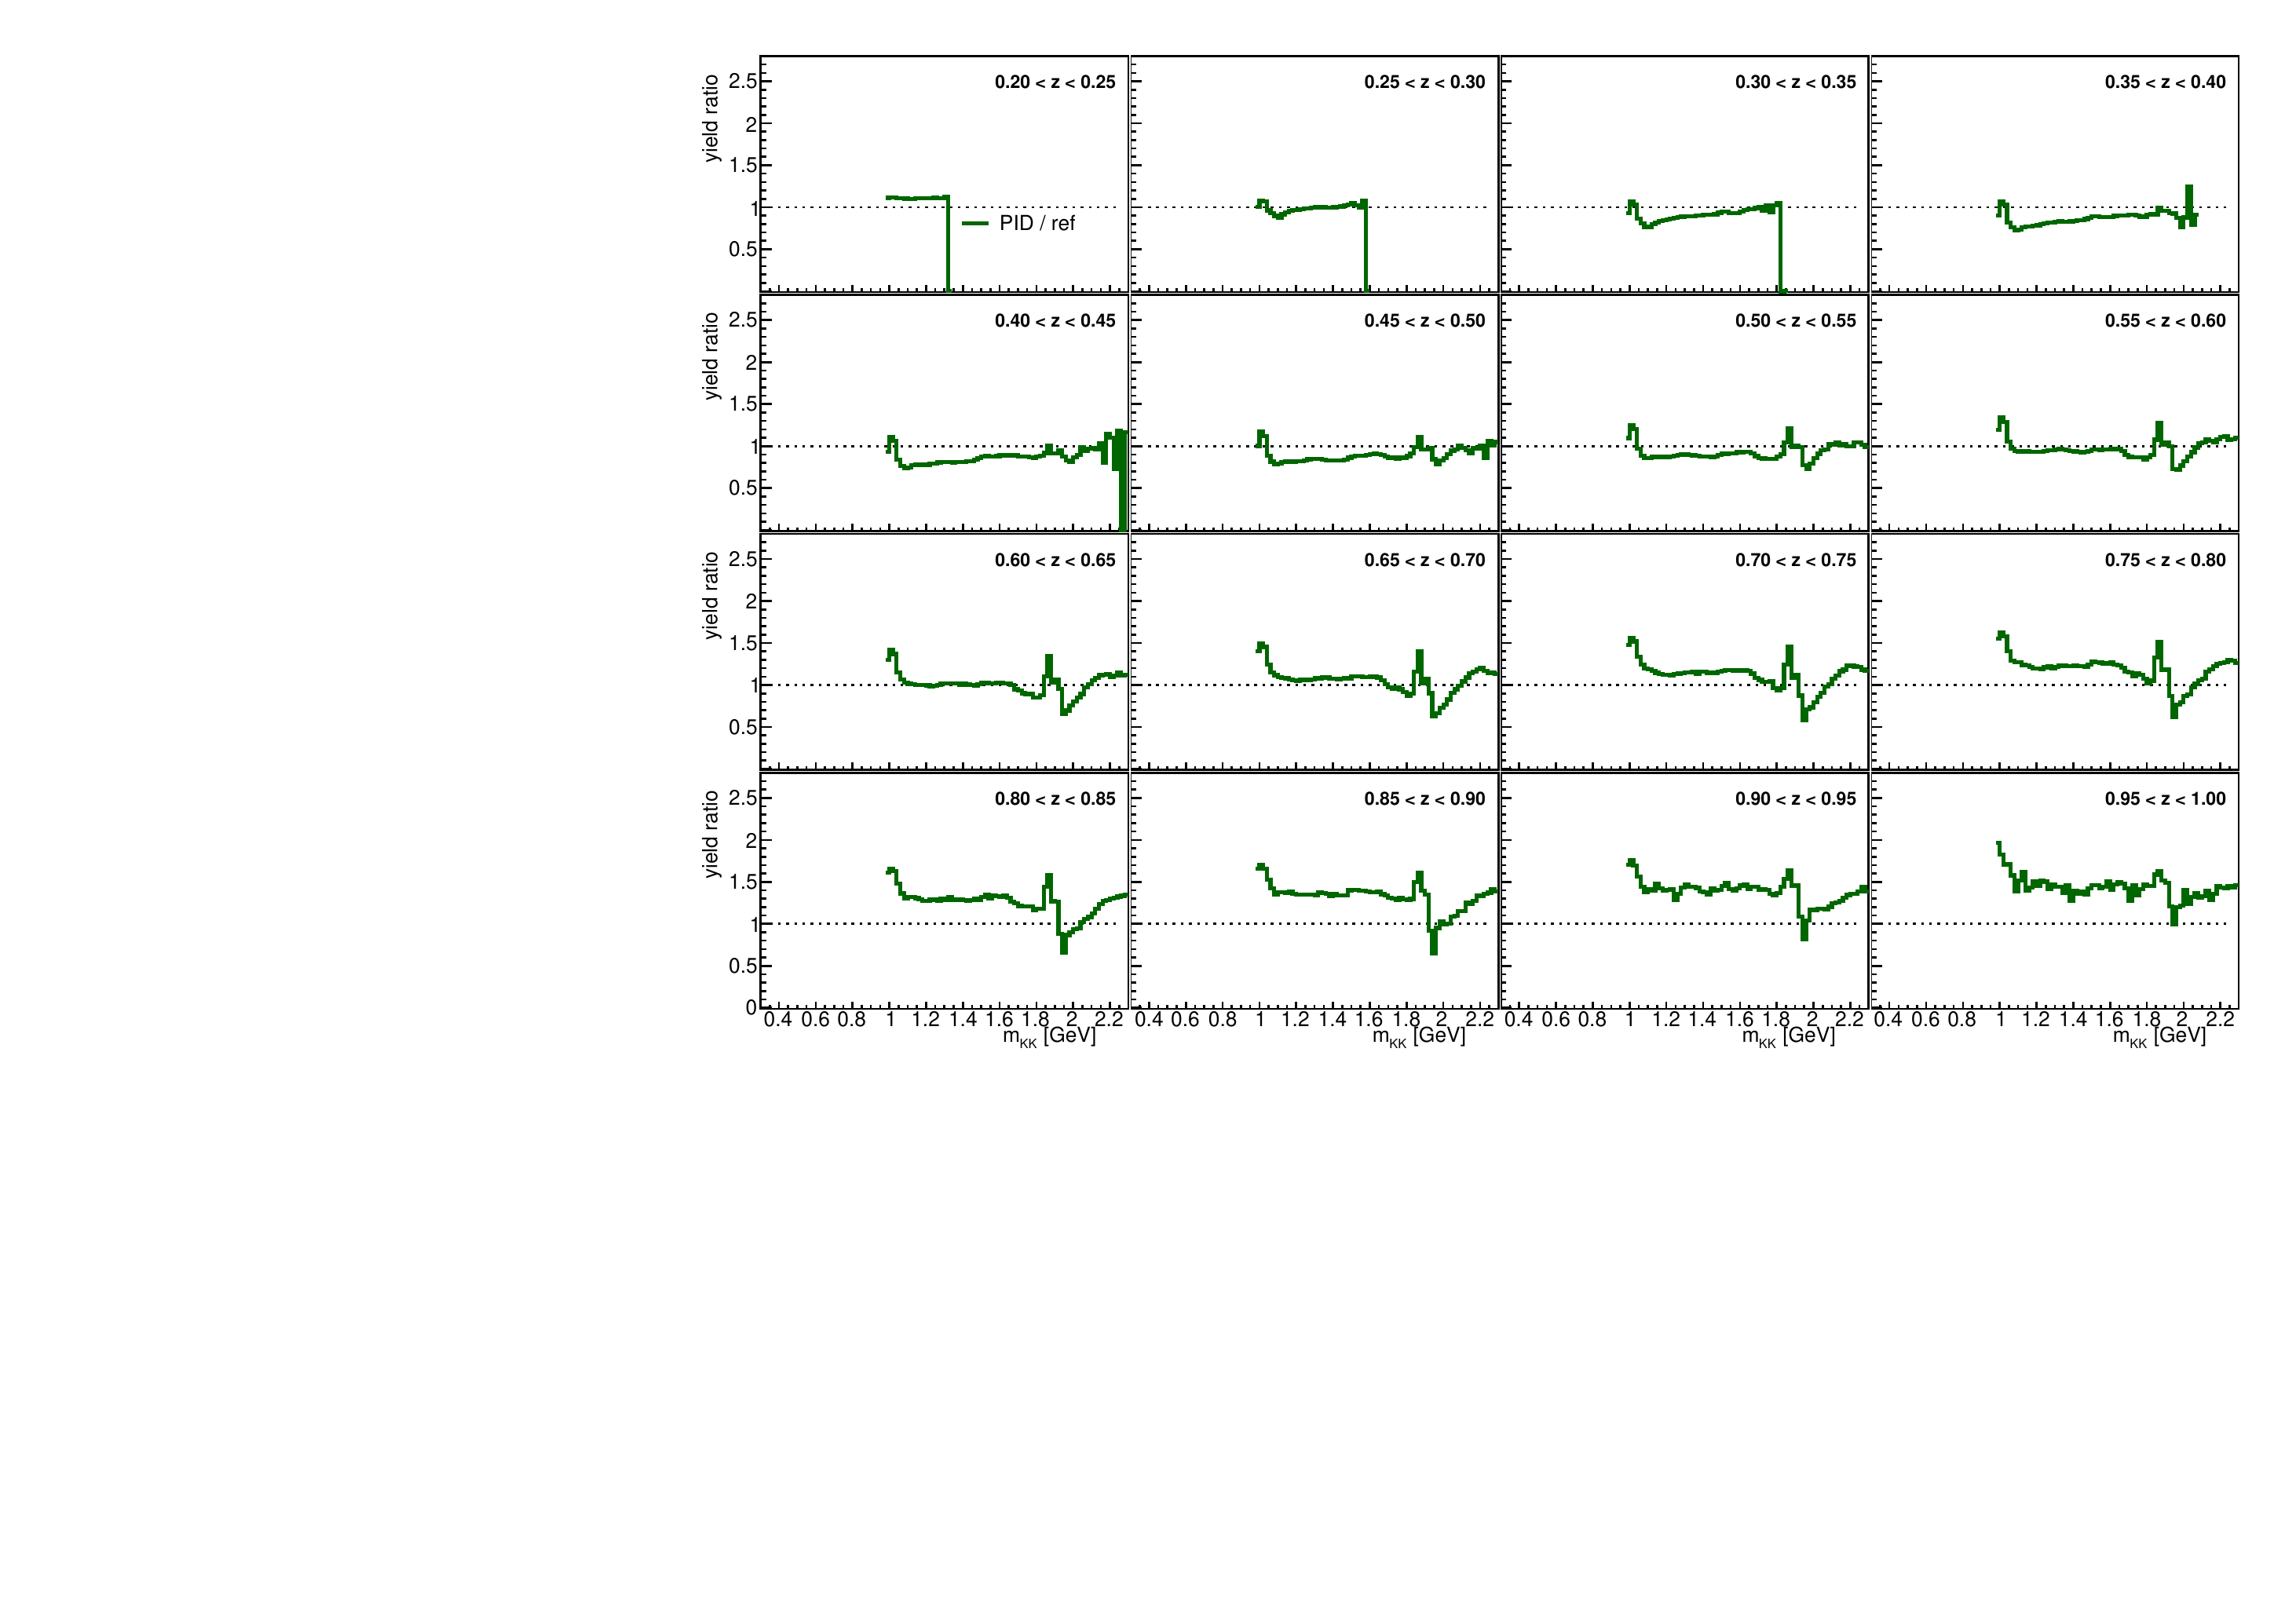} 
\caption{\label{fig:beforeafterpid4096}Ratio of yields after to before applying the PID correction for  $K^+K^-$ pairs as a function of $m_{KK}$ in bins of $z$. Structures are observed due to sharp resonances; at low $z$, the kinematical limits are evident. }
\end{center}
\end{figure*}
\begin{figure*}[th]
\begin{center}
\includegraphics[width=0.8\textwidth]{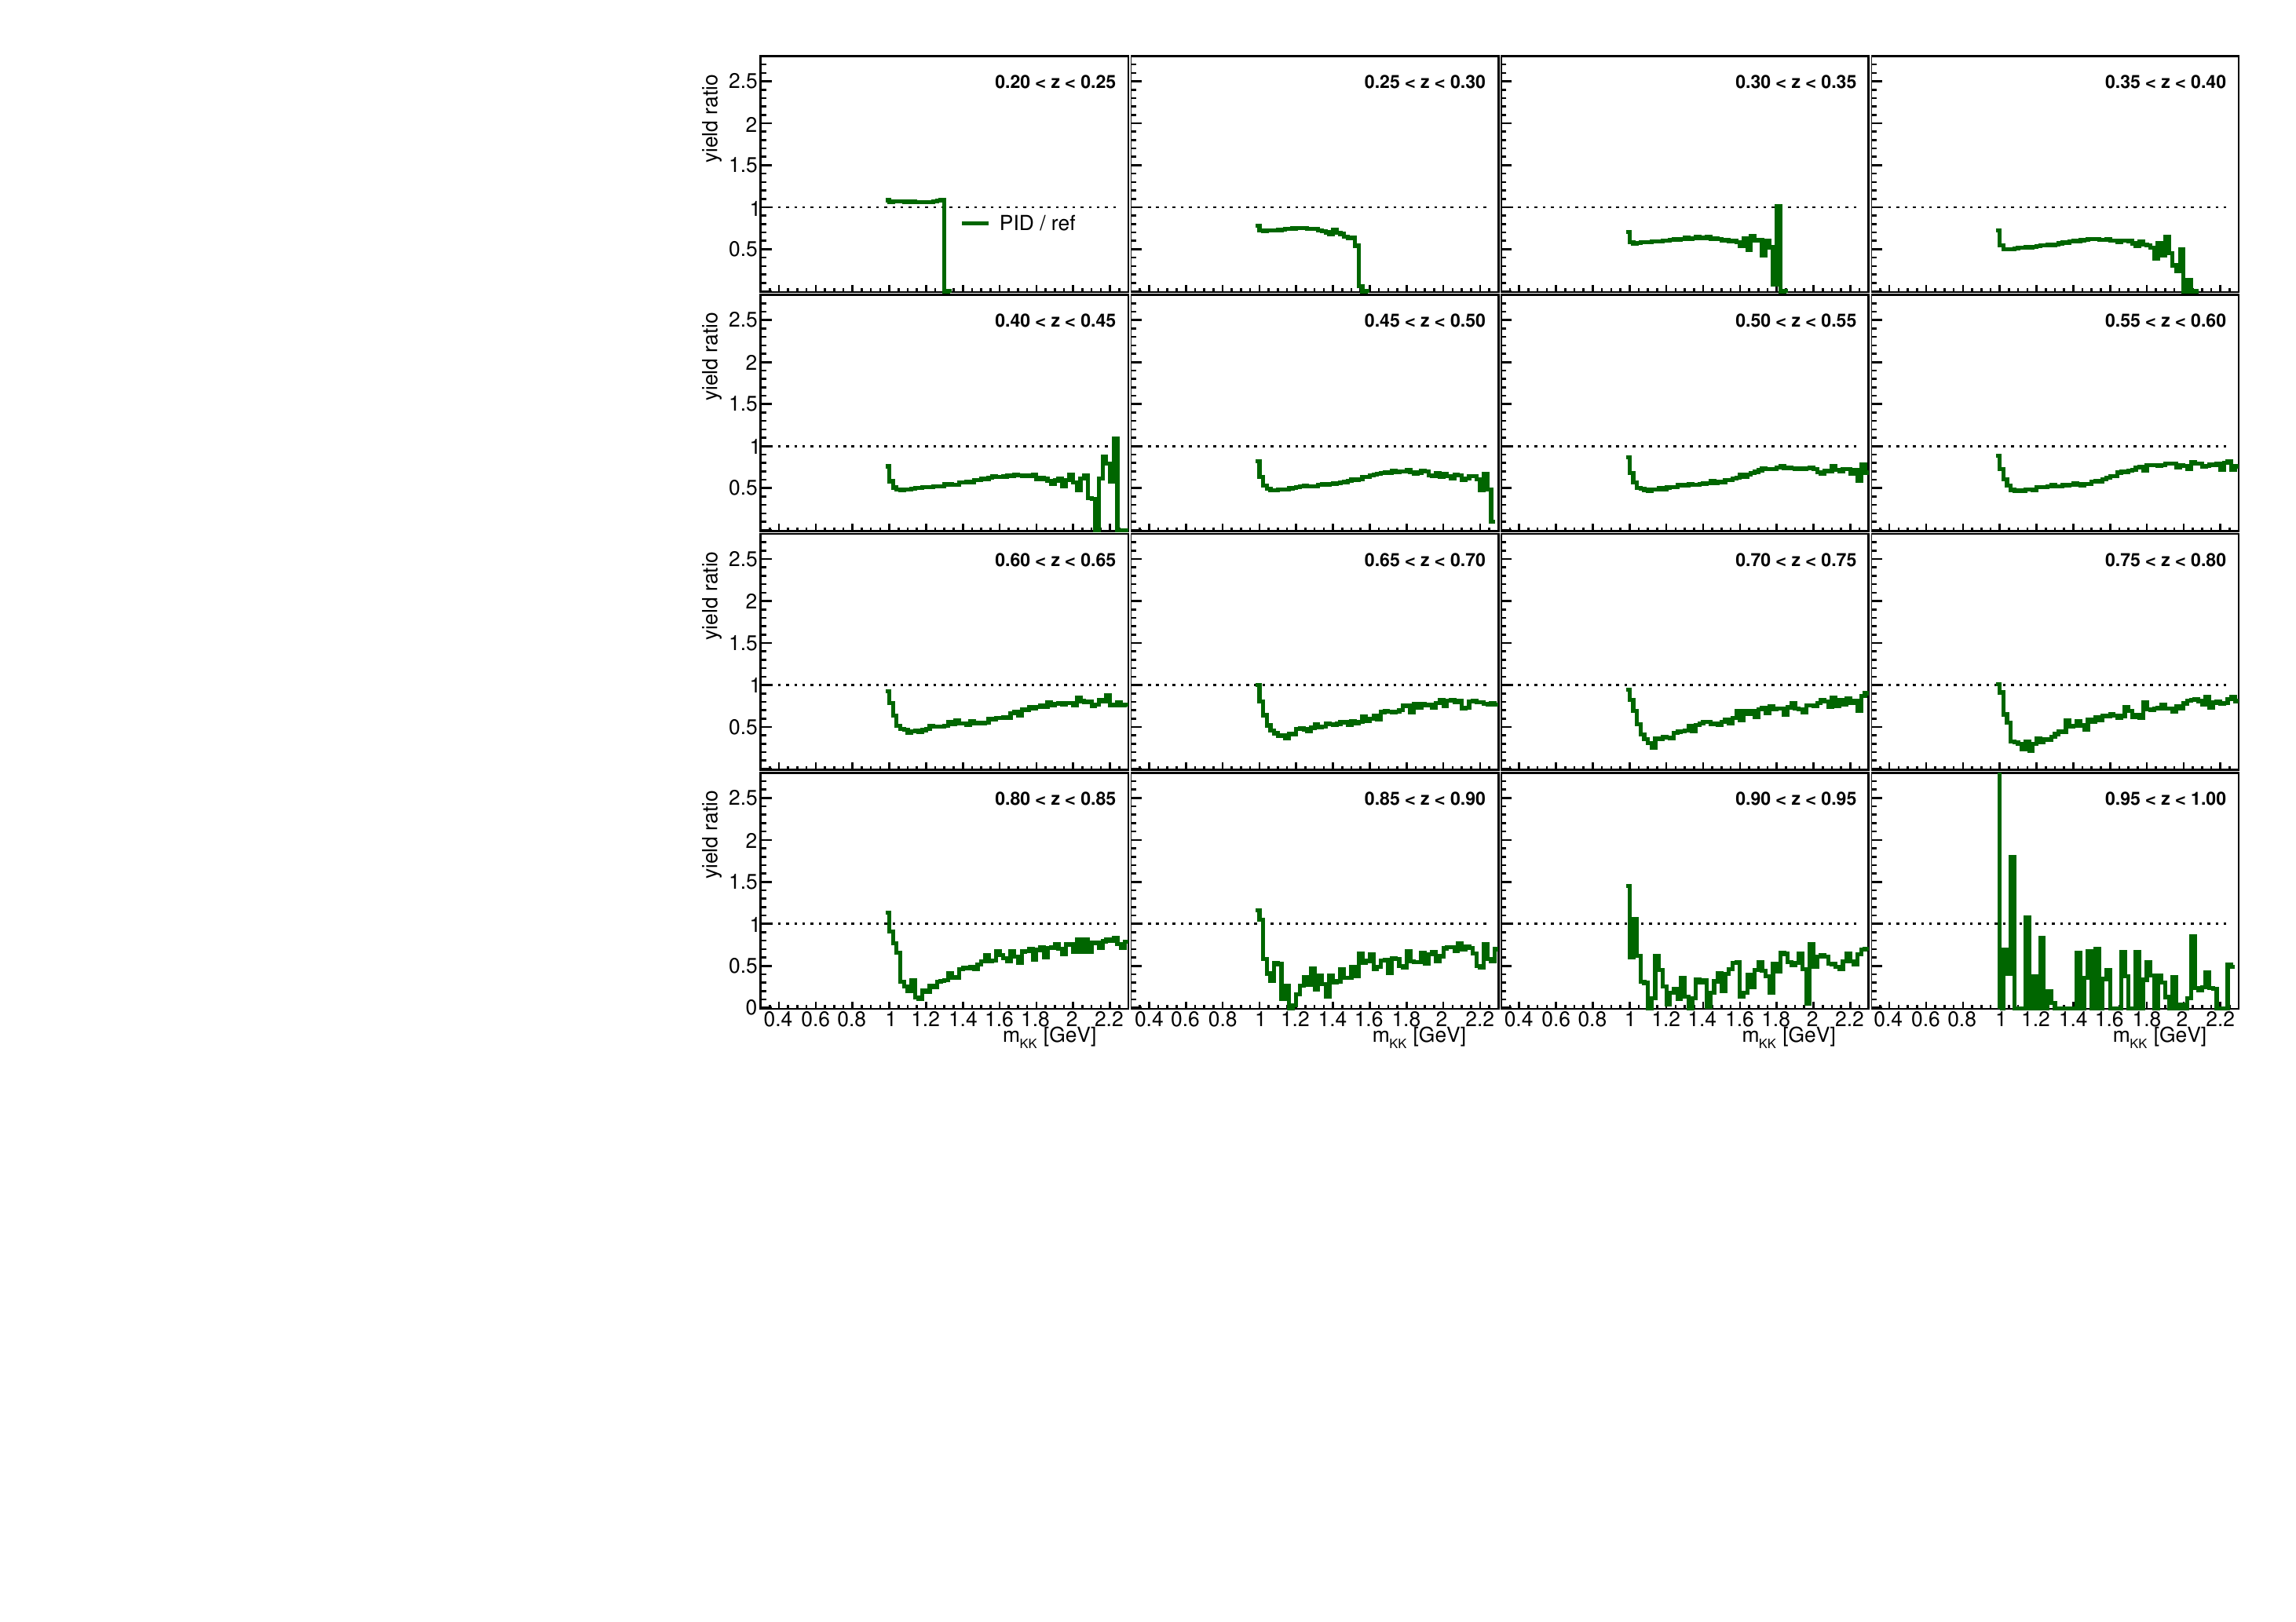} 
\caption{\label{fig:beforeafterpid8192}Ratio of yields after to before applying the PID correction for  $K^+K^+$ pairs as a function of $m_{KK}$ in bins of $z$. Structures are observed due to sharp resonances; at low $z$, the kinematical limits are evident. }
\end{center}
\end{figure*}

 \clearpage

\subsection{Preselection and acceptance correction}
Figures \ref{fig:acceptance2} to \ref{fig:acceptance8192} display the effects of the preselection and acceptance corrections for the same-sign hadron pairs as well as the opposite-sign pion-kaon and kaon pairs.
\begin{figure*}[ht]
\begin{center}
\includegraphics[width=0.8\textwidth]{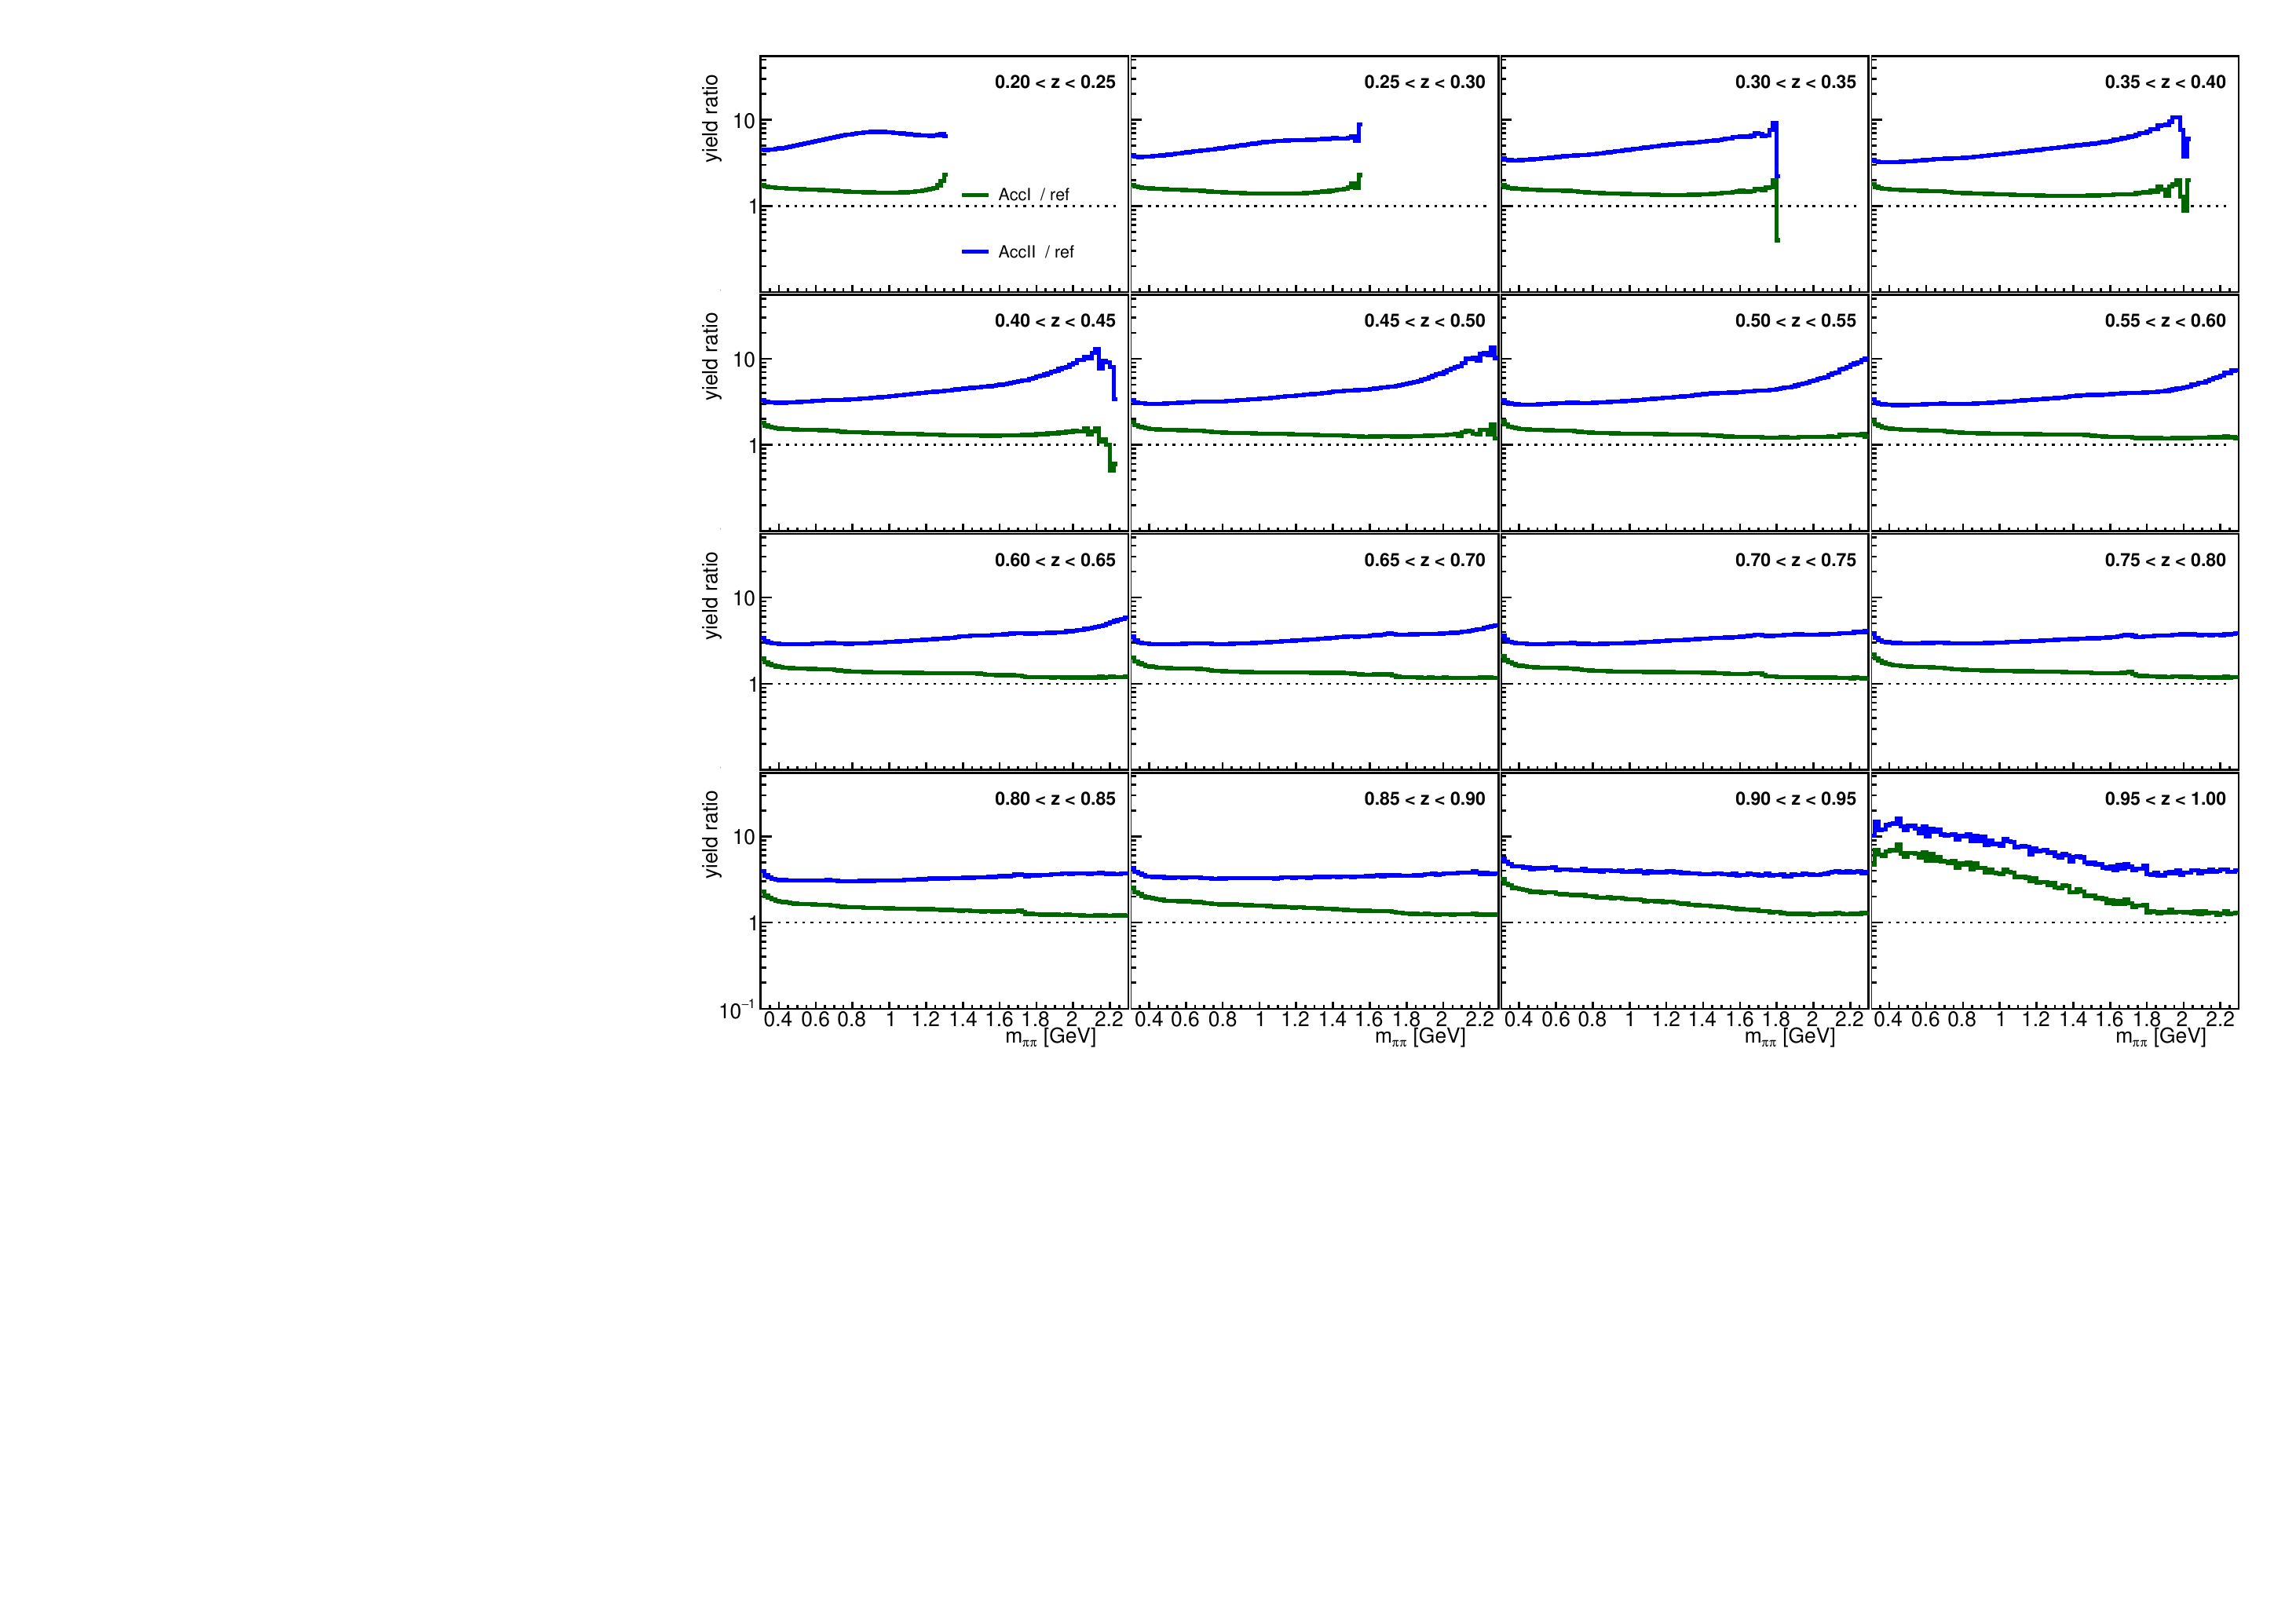} 
\caption{\label{fig:acceptance2}Yield ratios after successively applying all acceptance and efficiency corrections (labeled AccI and AccII as the two acceptance corrections discussed in the paper text) relative to the reference yields after non-$q\bar{q}$ removal for  $\pi^+\pi^+$ pairs as a function of $m_{\pi\pi}$ in bins of $z$.}
\end{center}
\end{figure*}
\begin{figure*}[ht]
\begin{center}
\includegraphics[width=0.8\textwidth]{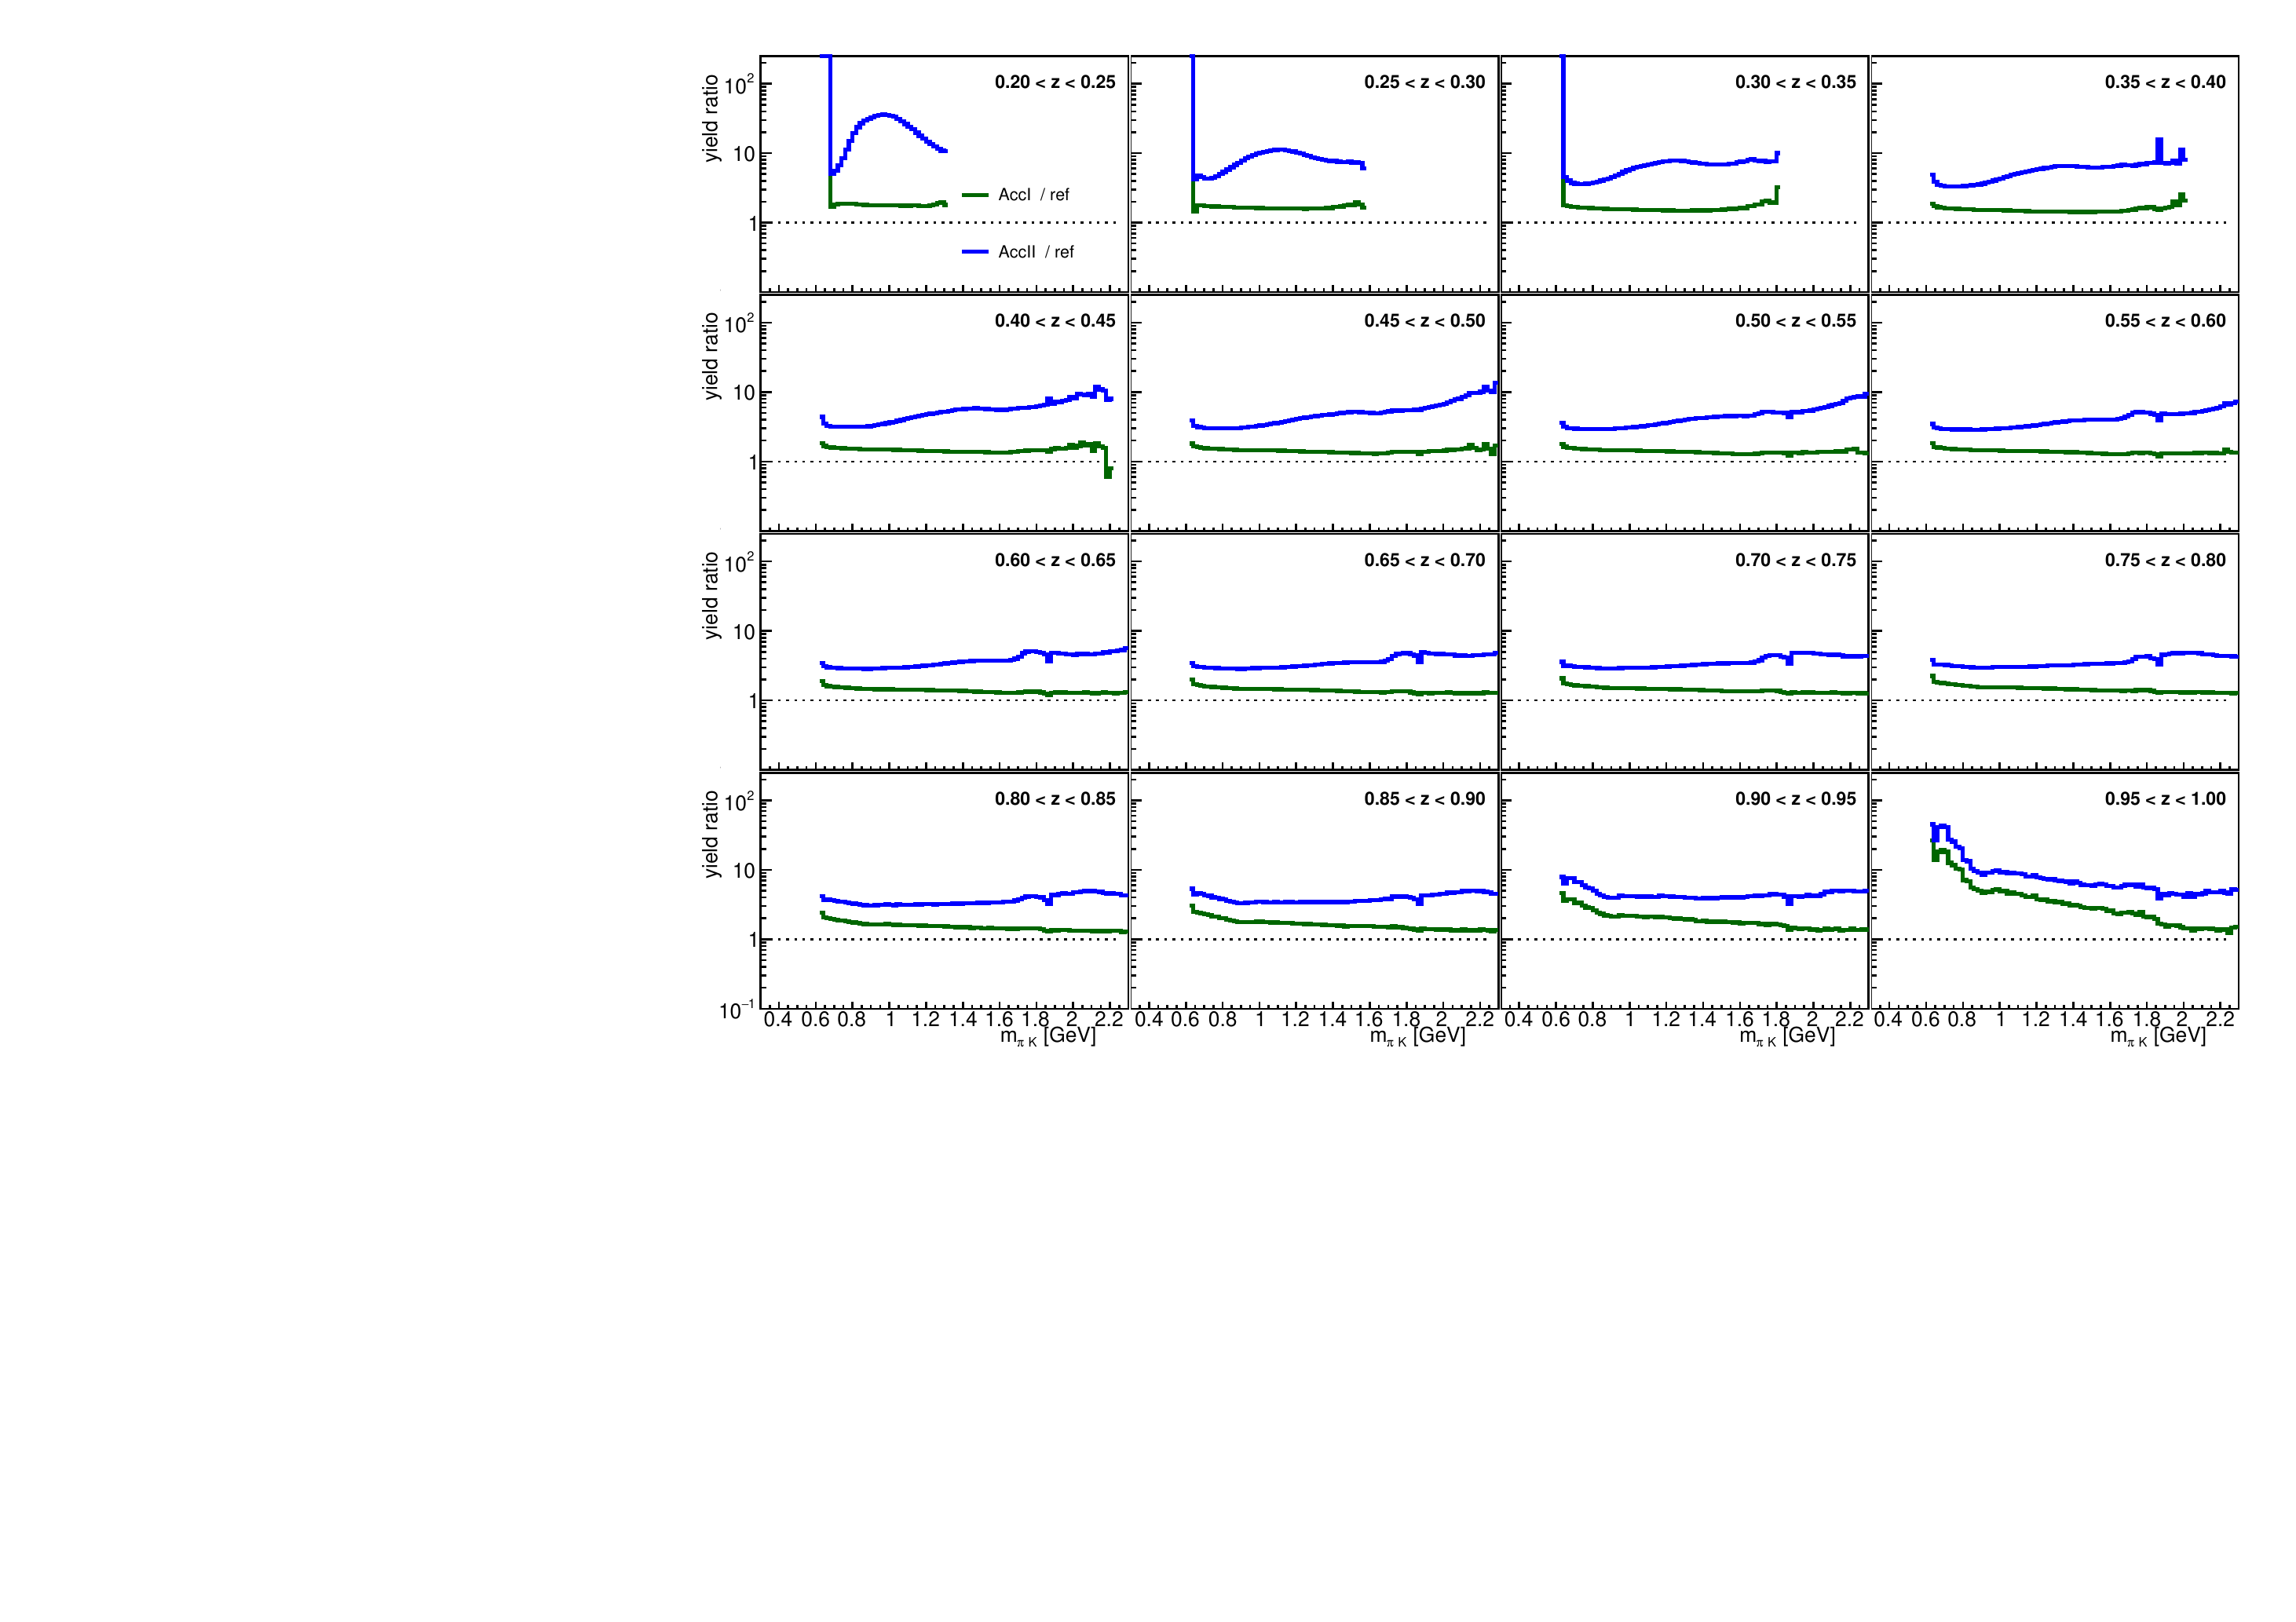} 
\caption{\label{fig:acceptance16}Yield ratios after successively applying all acceptance and efficiency corrections (labeled AccI and AccII as the two acceptance corrections discussed in the paper text) relative to the reference yields after non-$q\bar{q}$ removal for  $\pi^+K^-$ pairs as a function of $m_{K\pi}$ in bins of $z$.}
\end{center}
\end{figure*}

\begin{figure*}[ht]
\begin{center}
\includegraphics[width=0.8\textwidth]{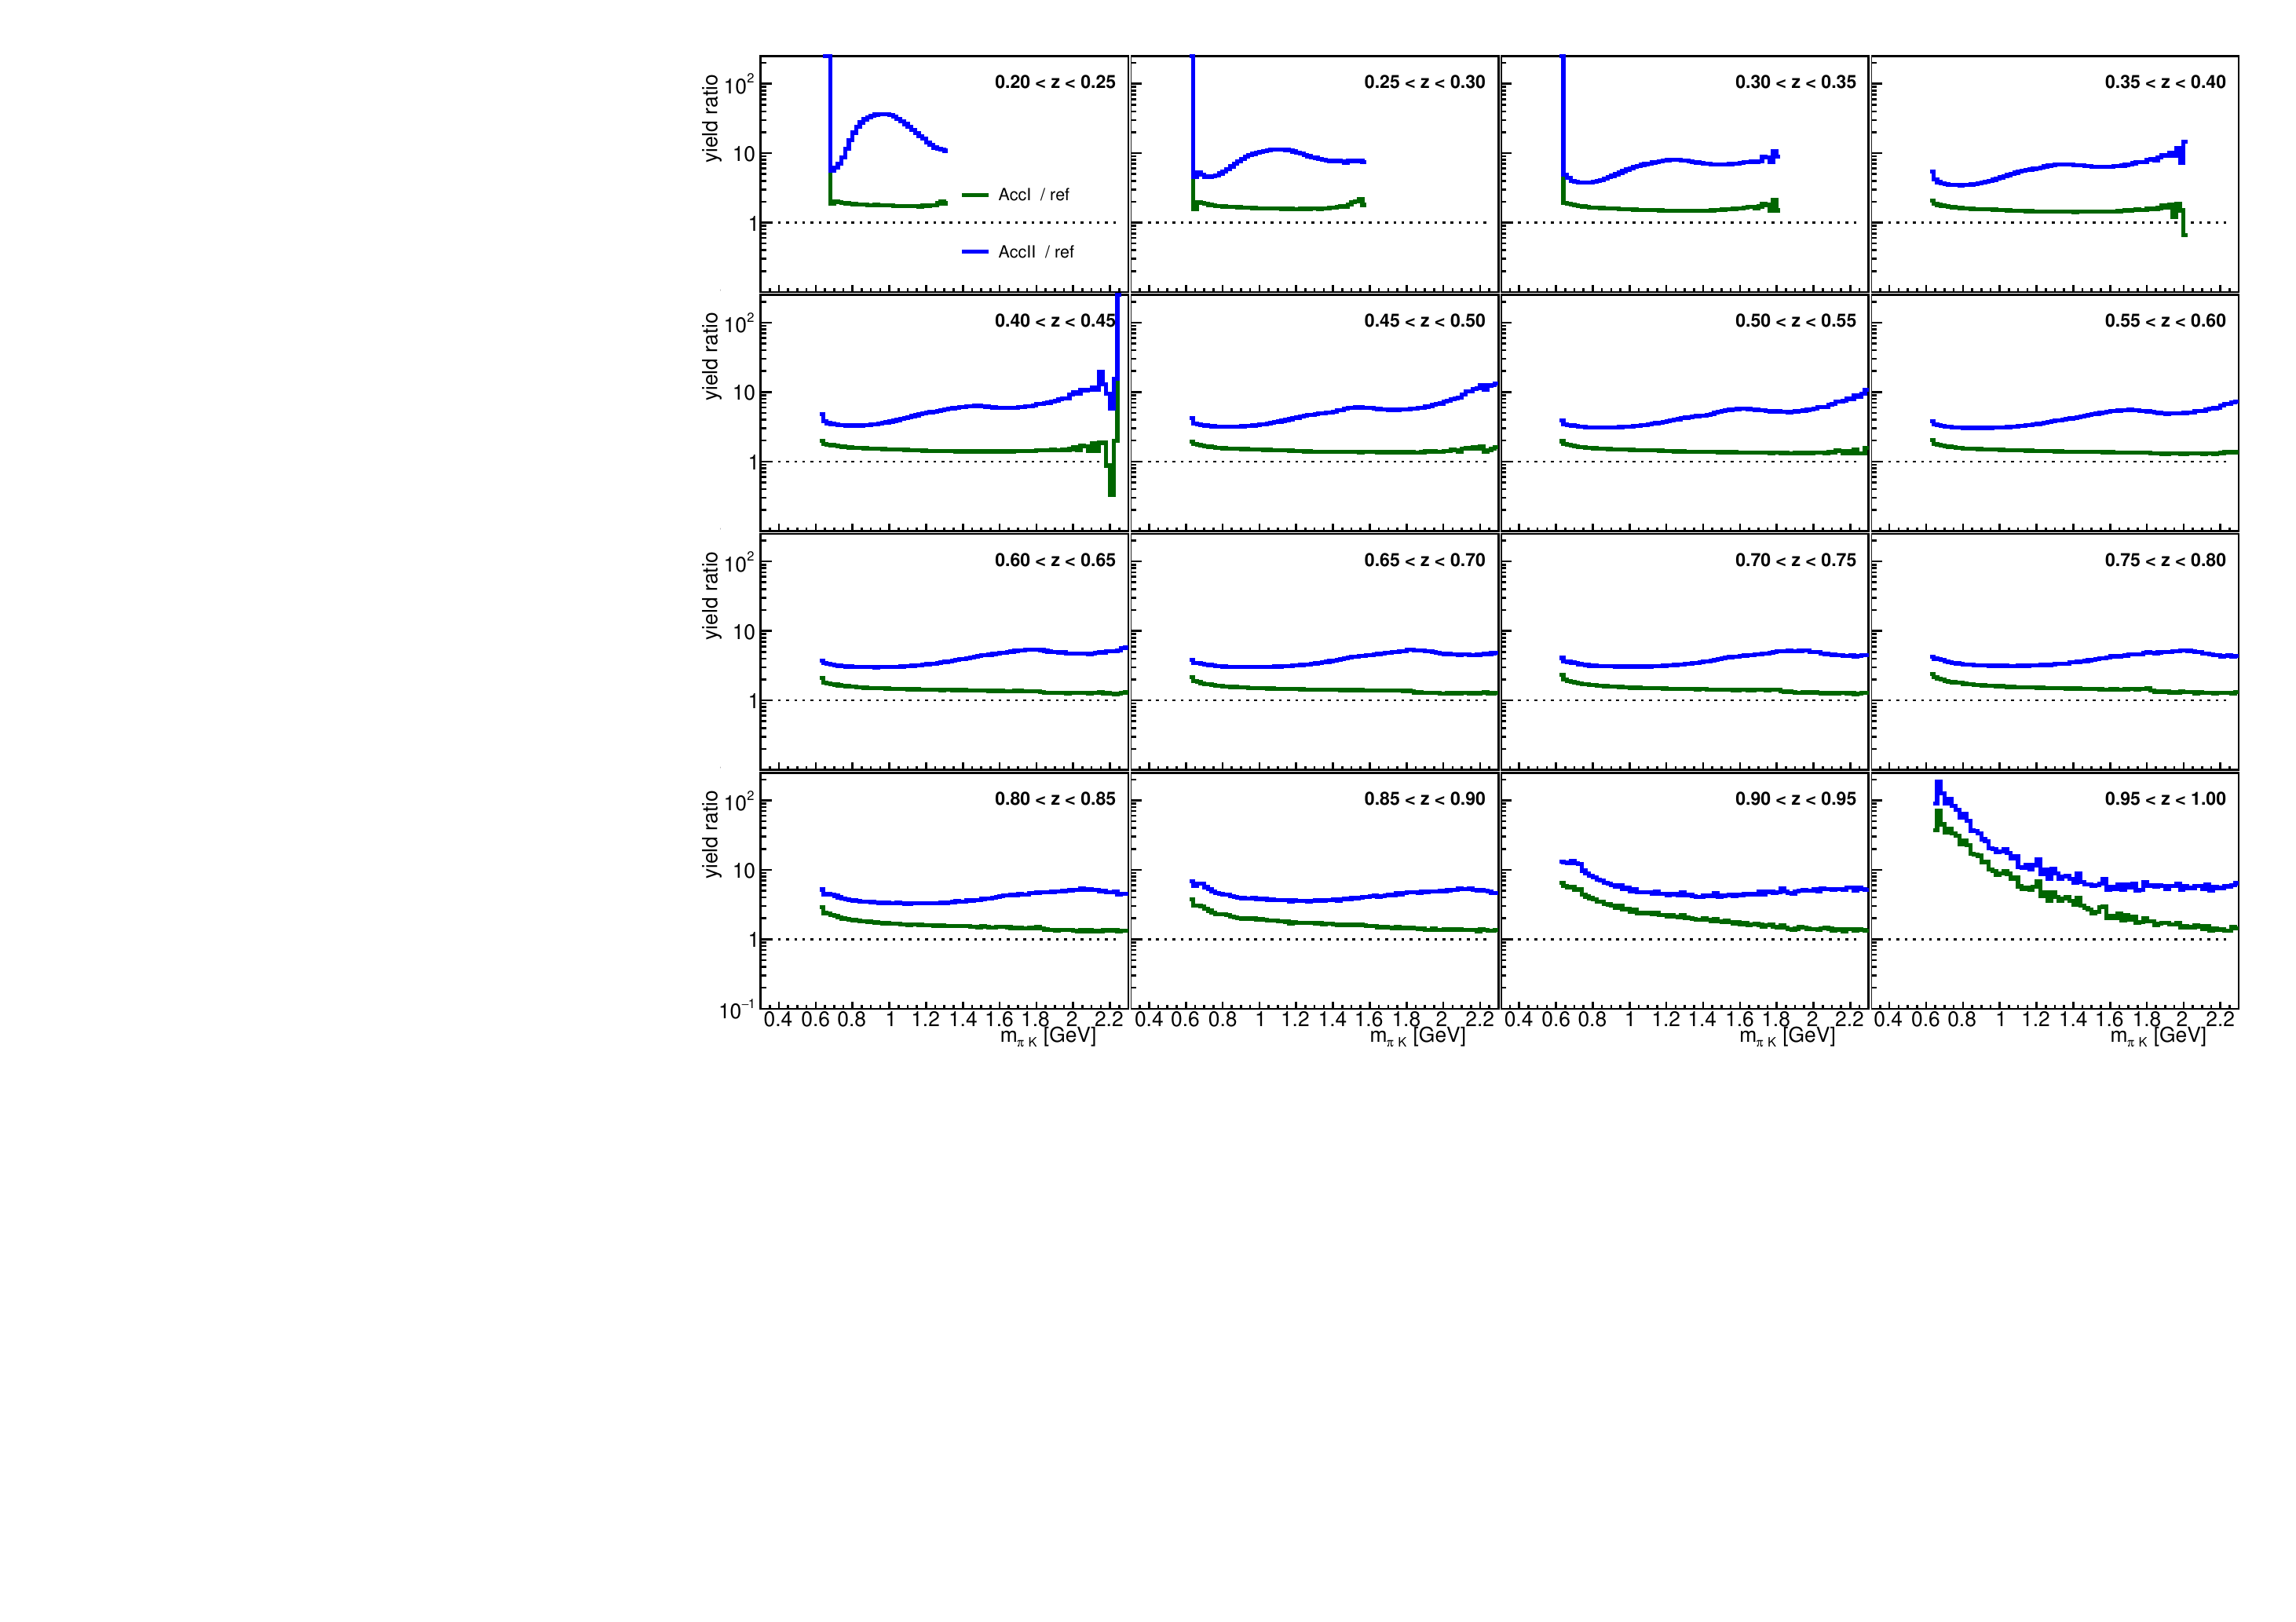} 
\caption{\label{fig:acceptance32}Yield ratios after successively applying all acceptance and efficiency corrections (labeled AccI and AccII as the two acceptance corrections discussed in the paper text) relative to the reference yields after non-$q\bar{q}$ removal for  $\pi^+K^+$ pairs as a function of $m_{K\pi}$ in bins of $z$.}
\end{center}
\end{figure*}

\begin{figure*}[ht]
\begin{center}
\includegraphics[width=0.8\textwidth]{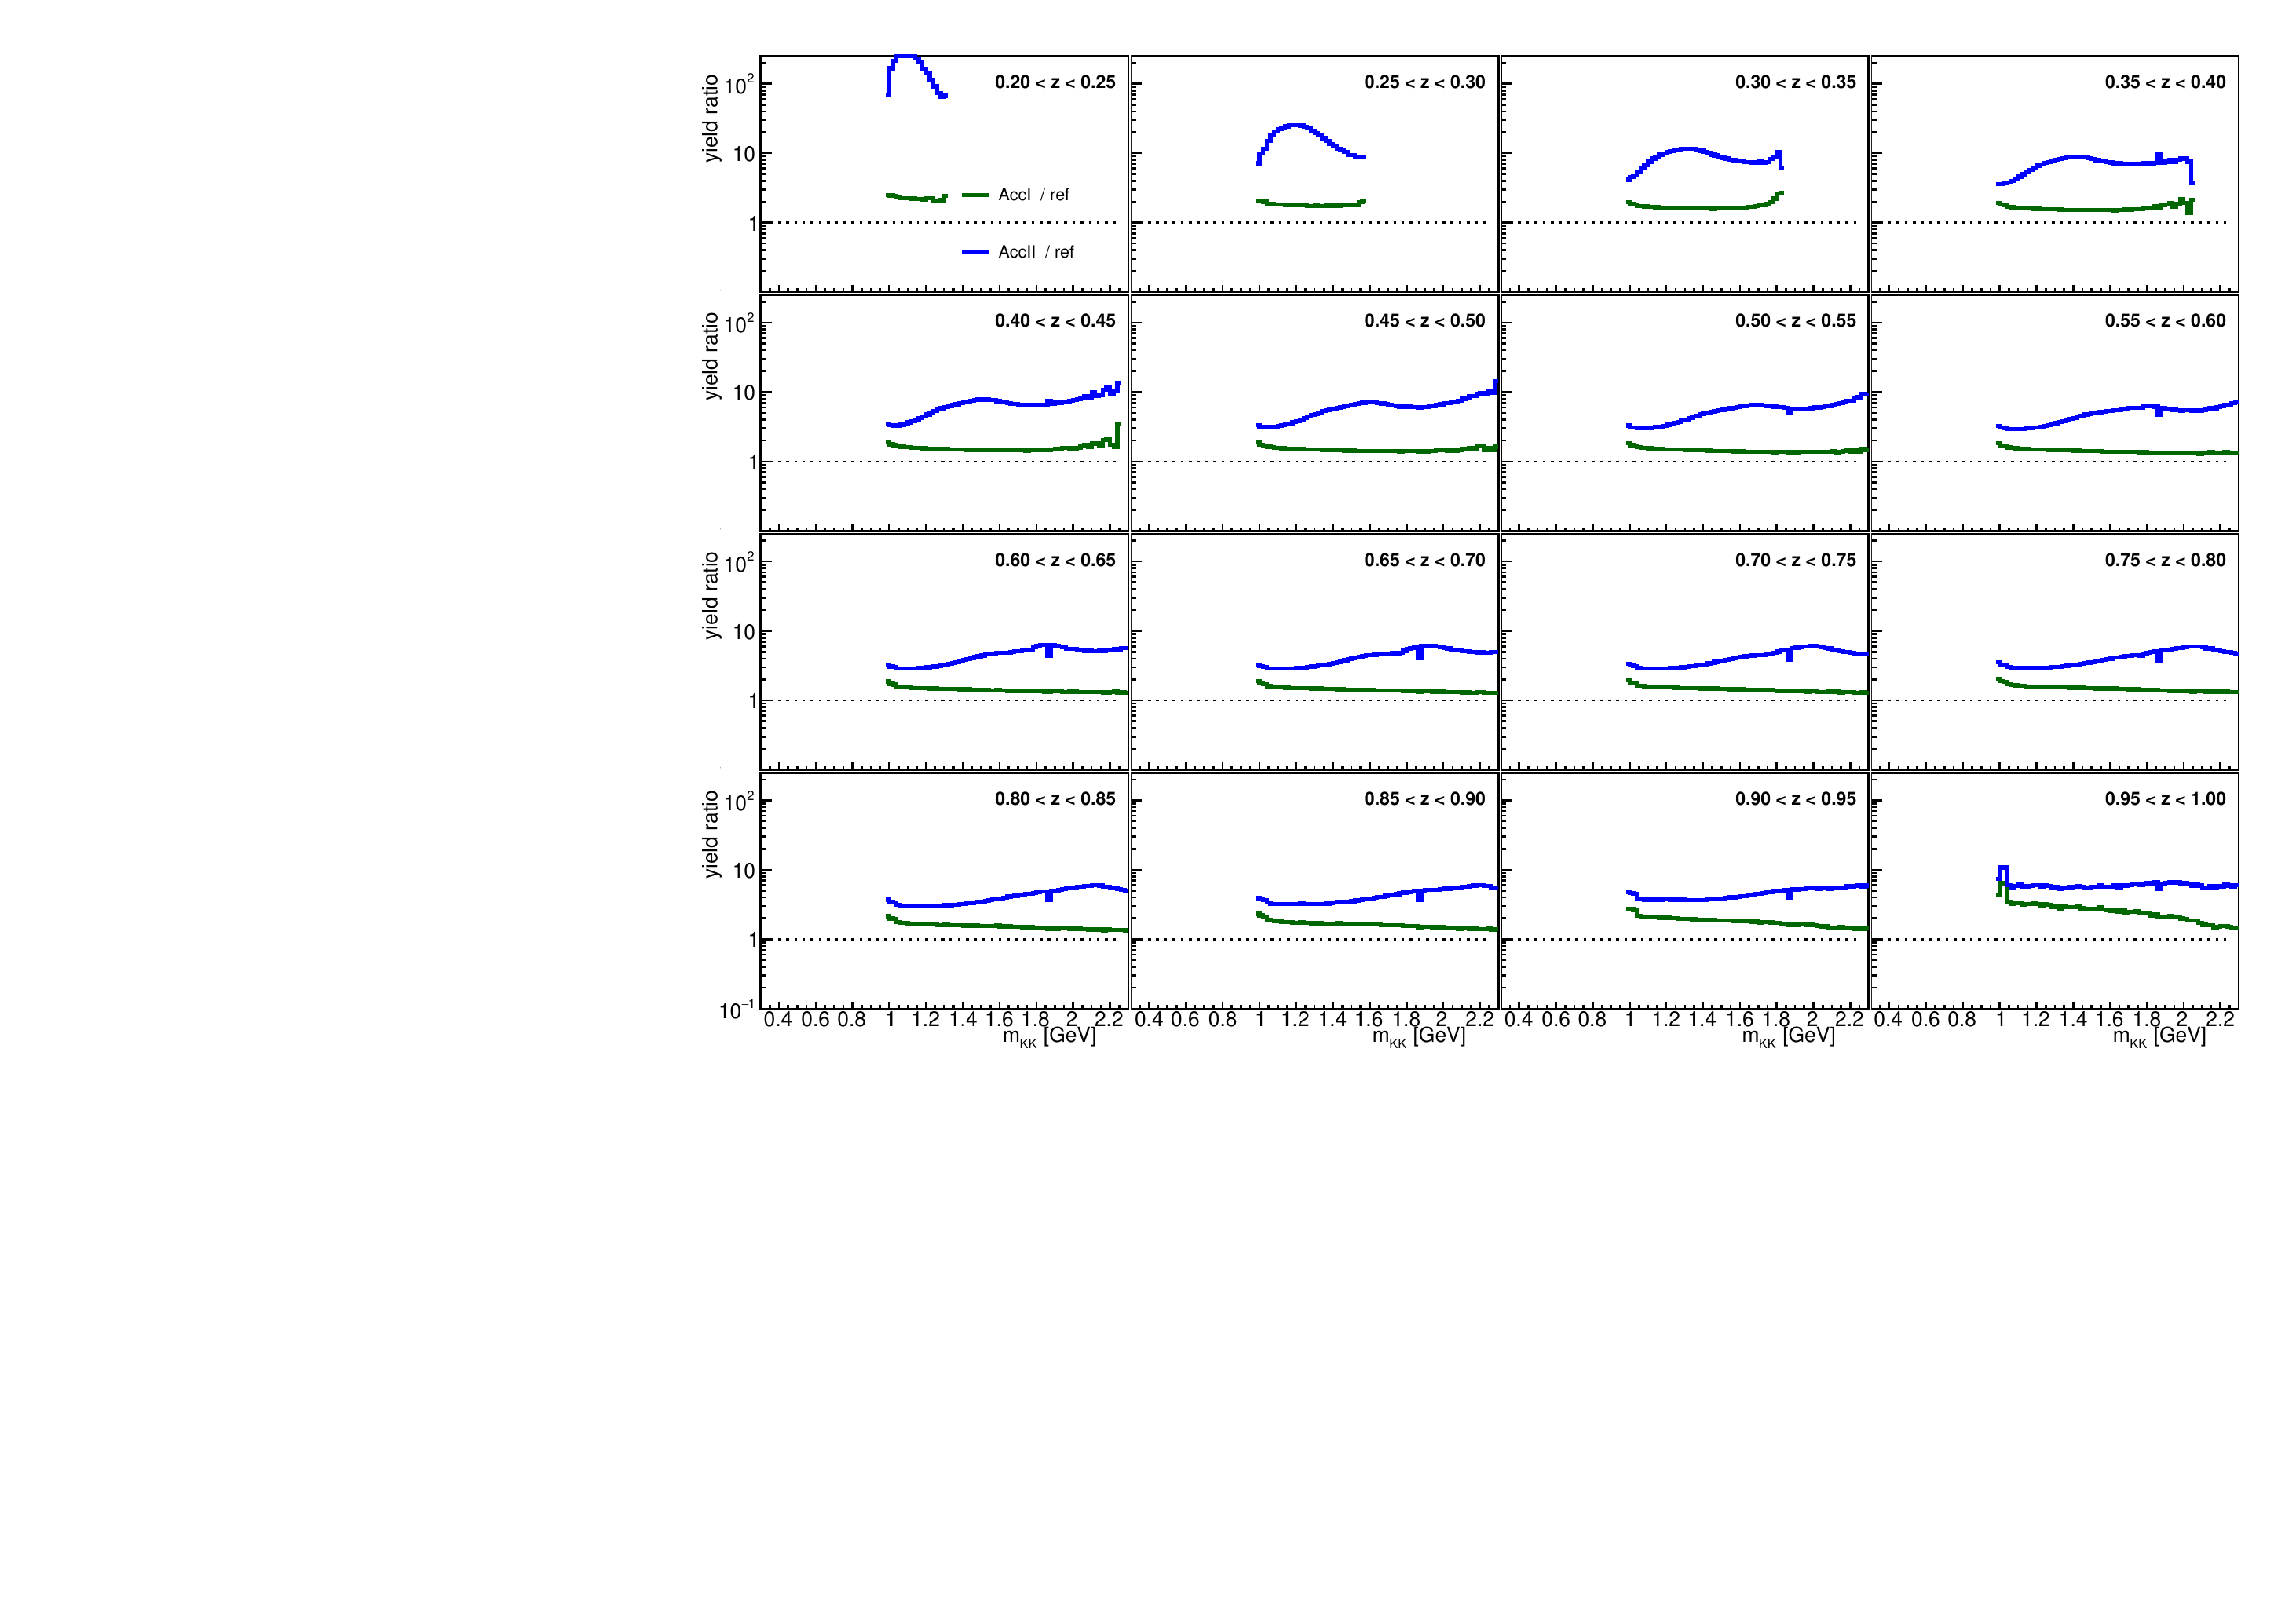} 
\caption{\label{fig:acceptance4096}Yield ratios after successively applying all acceptance and efficiency corrections (labeled AccI and AccII as the two acceptance corrections discussed in the paper text) relative to the reference yields after non-$q\bar{q}$ removal for  $K^+K^-$ pairs as a function of $m_{KK}$ in bins of $z$.}
\end{center}
\end{figure*}
\begin{figure*}[ht]
\begin{center}
\includegraphics[width=0.8\textwidth]{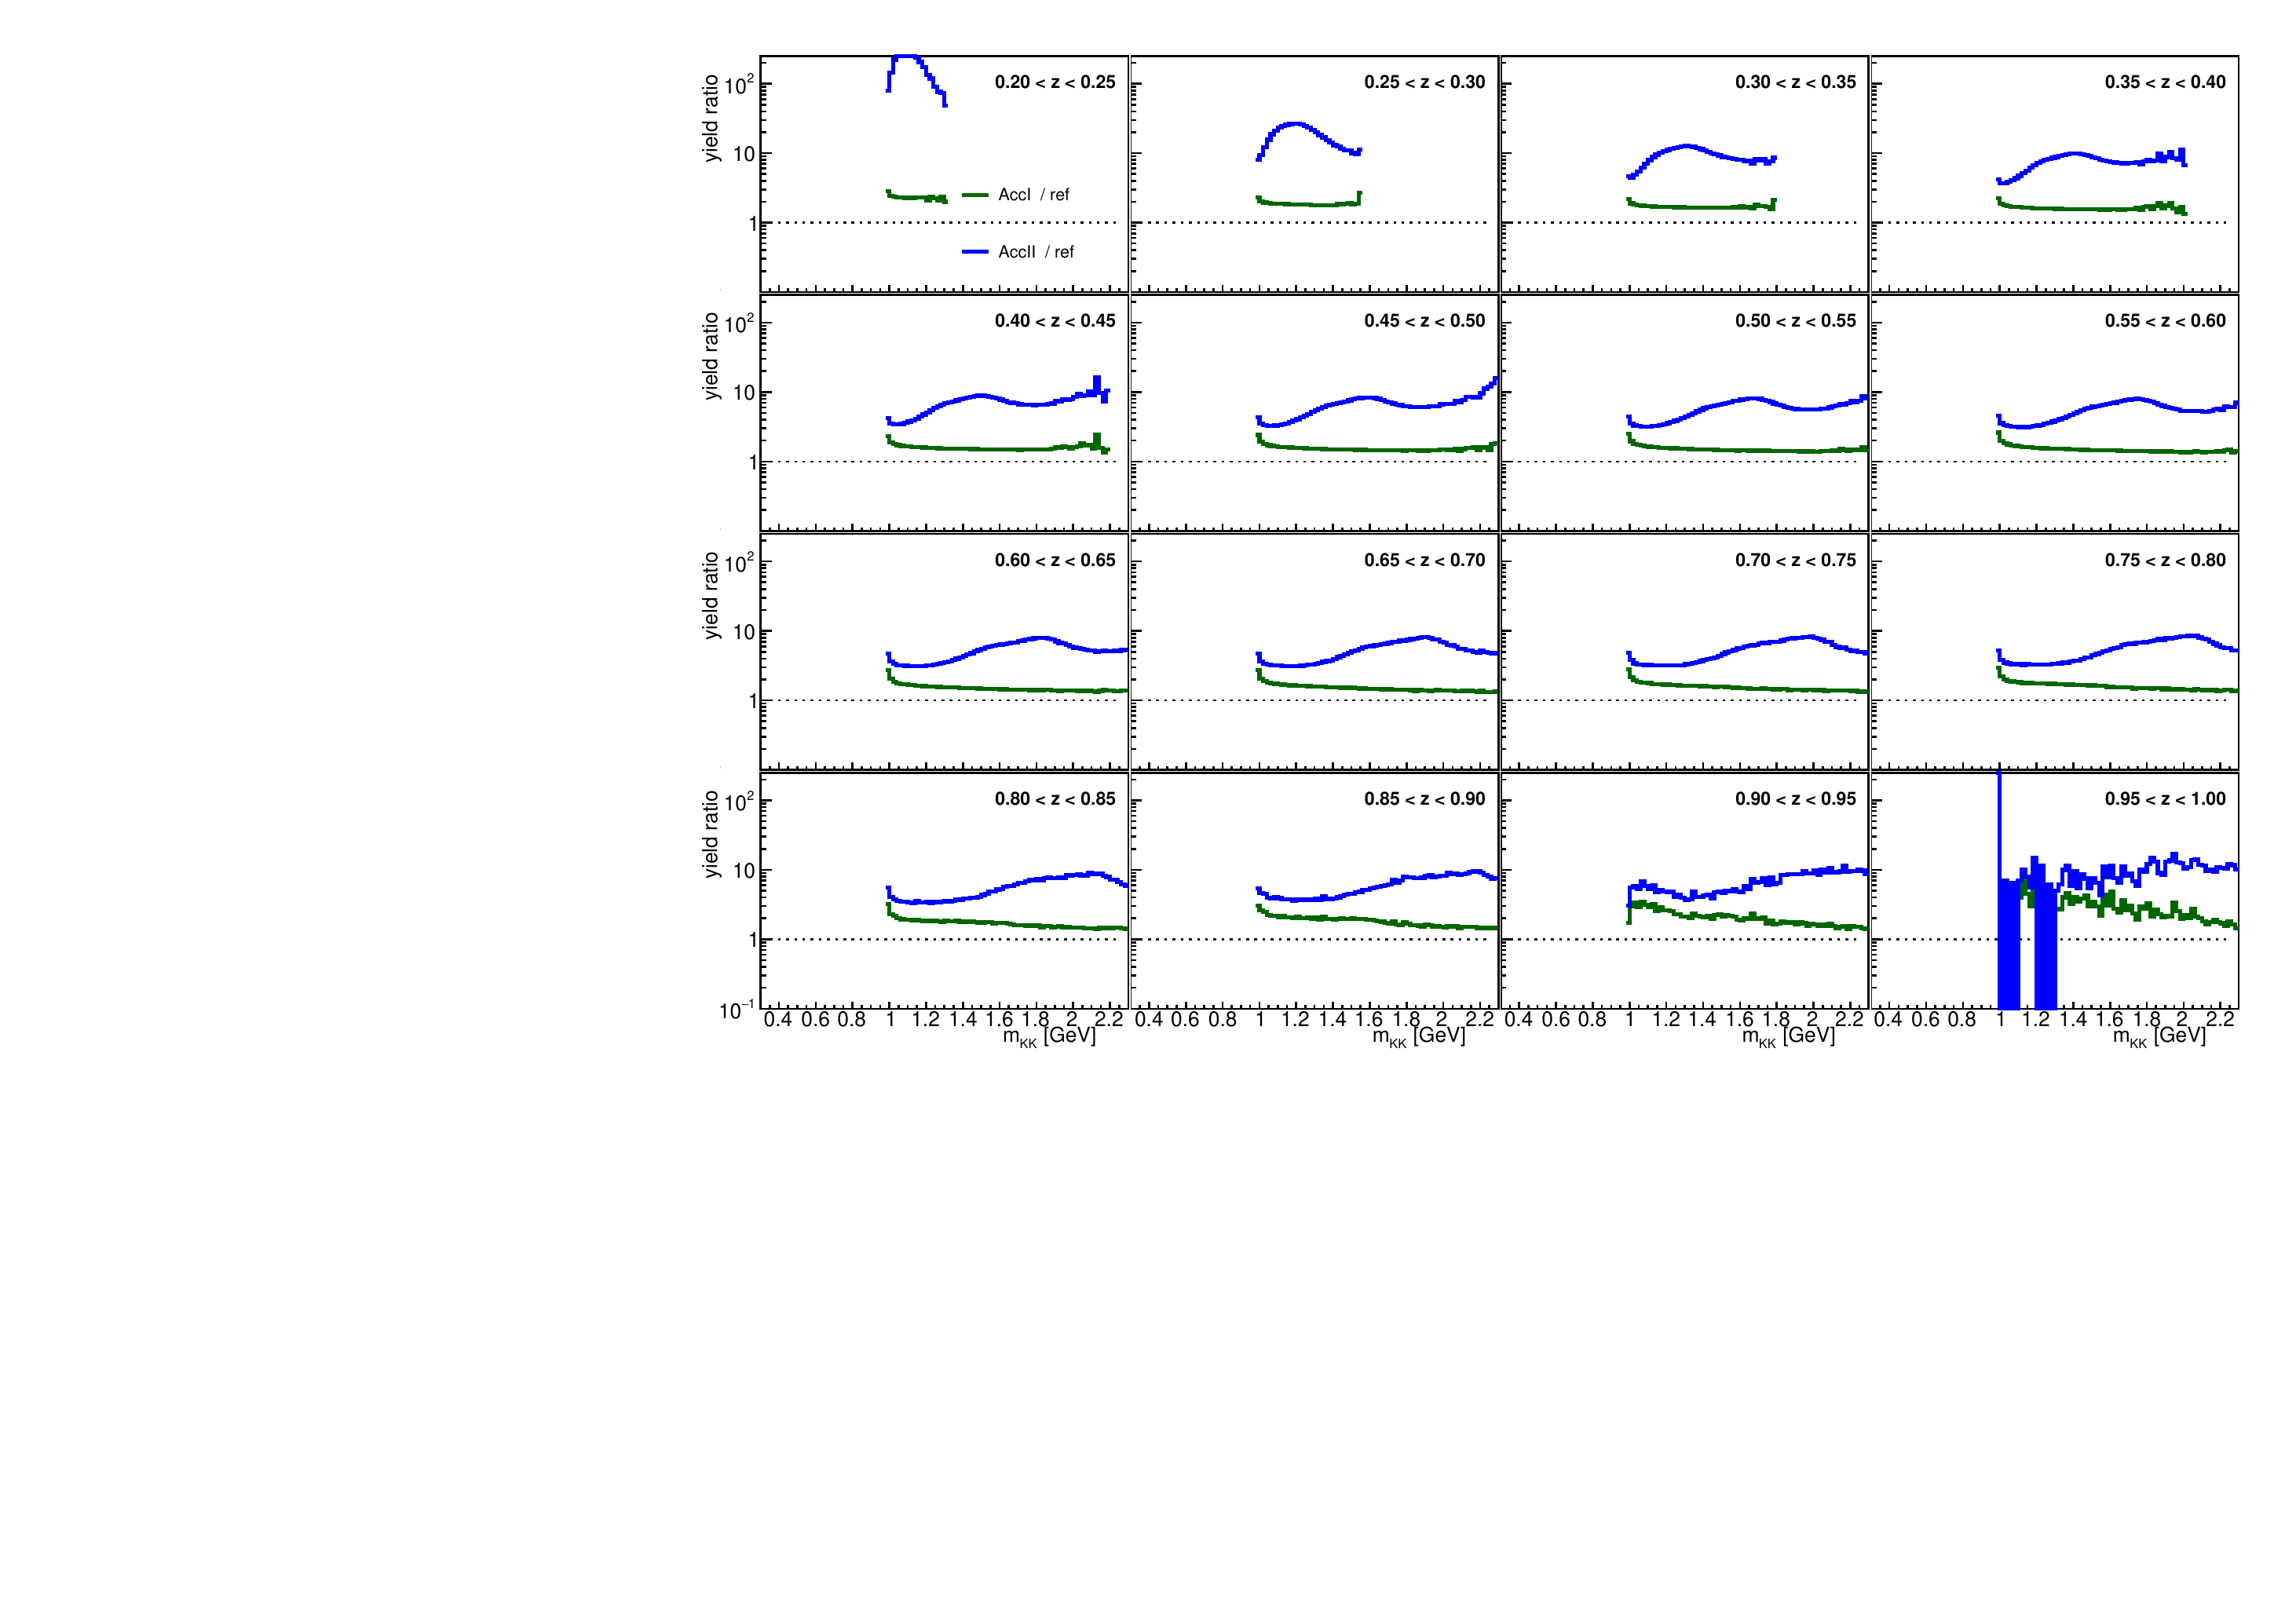} 
\caption{\label{fig:acceptance8192}Yield ratios after successively applying all acceptance and efficiency corrections (labeled AccI and AccII as the two acceptance corrections discussed in the paper text) relative to the reference yields after non-$q\bar{q}$ removal for  $K^+K^+$ pairs as a function of $m_{KK}$ in bins of $z$.}
\end{center}
\end{figure*}
\clearpage
\subsection{Systematic uncertainties}
Figures \ref{fig:systall_pid2} to \ref{fig:systall_pid8192} display the statistical and systematic (upper and lower) uncertainties for the same-sign hadron pairs as well as the opposite-sign pion-kaon and kaon pairs.

\begin{figure*}[htb]
\begin{center}
\includegraphics[width=0.8\textwidth]{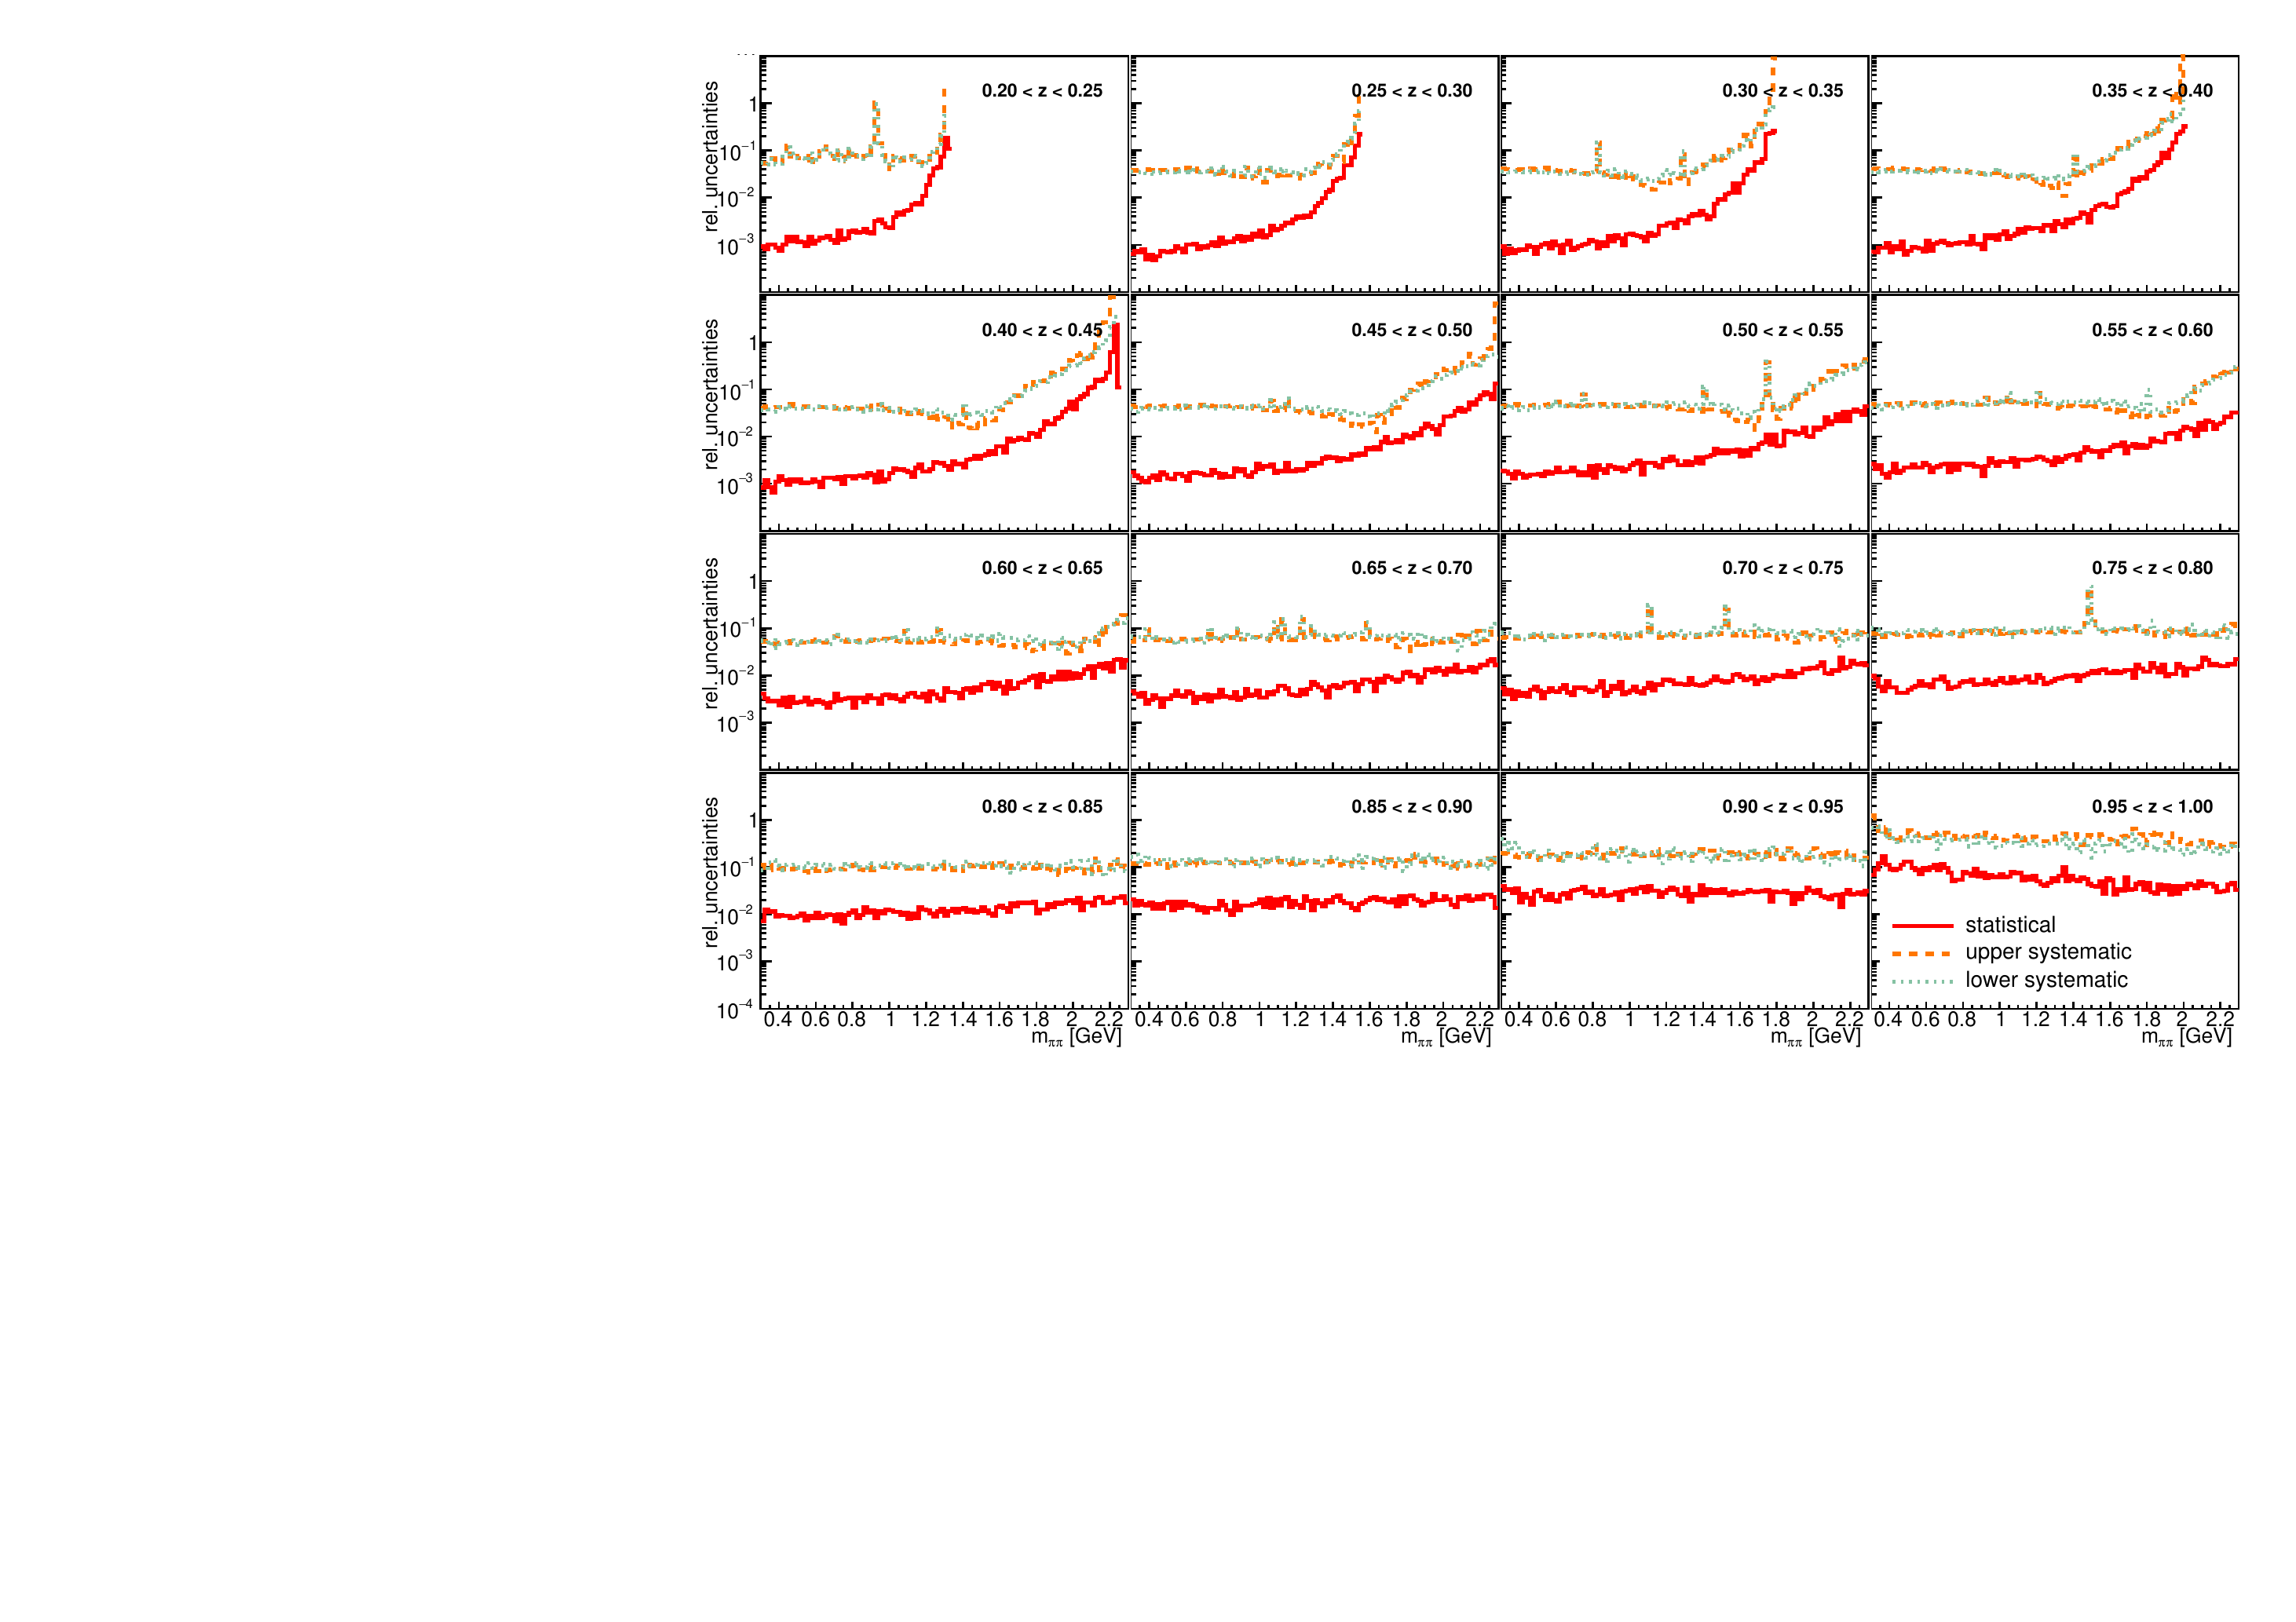}
\caption{\label{fig:systall_pid2} Relative (asymmetric) systematic uncertainties (upper, dashed lines; lower, dotted lines) and statistical uncertainties (full lines) for same-sign pion pairs as a function of $m_{\pi\pi}$ in bins of $z$.}
\end{center}
\end{figure*}
\begin{figure*}[htb]
\begin{center}
\includegraphics[width=0.8\textwidth]{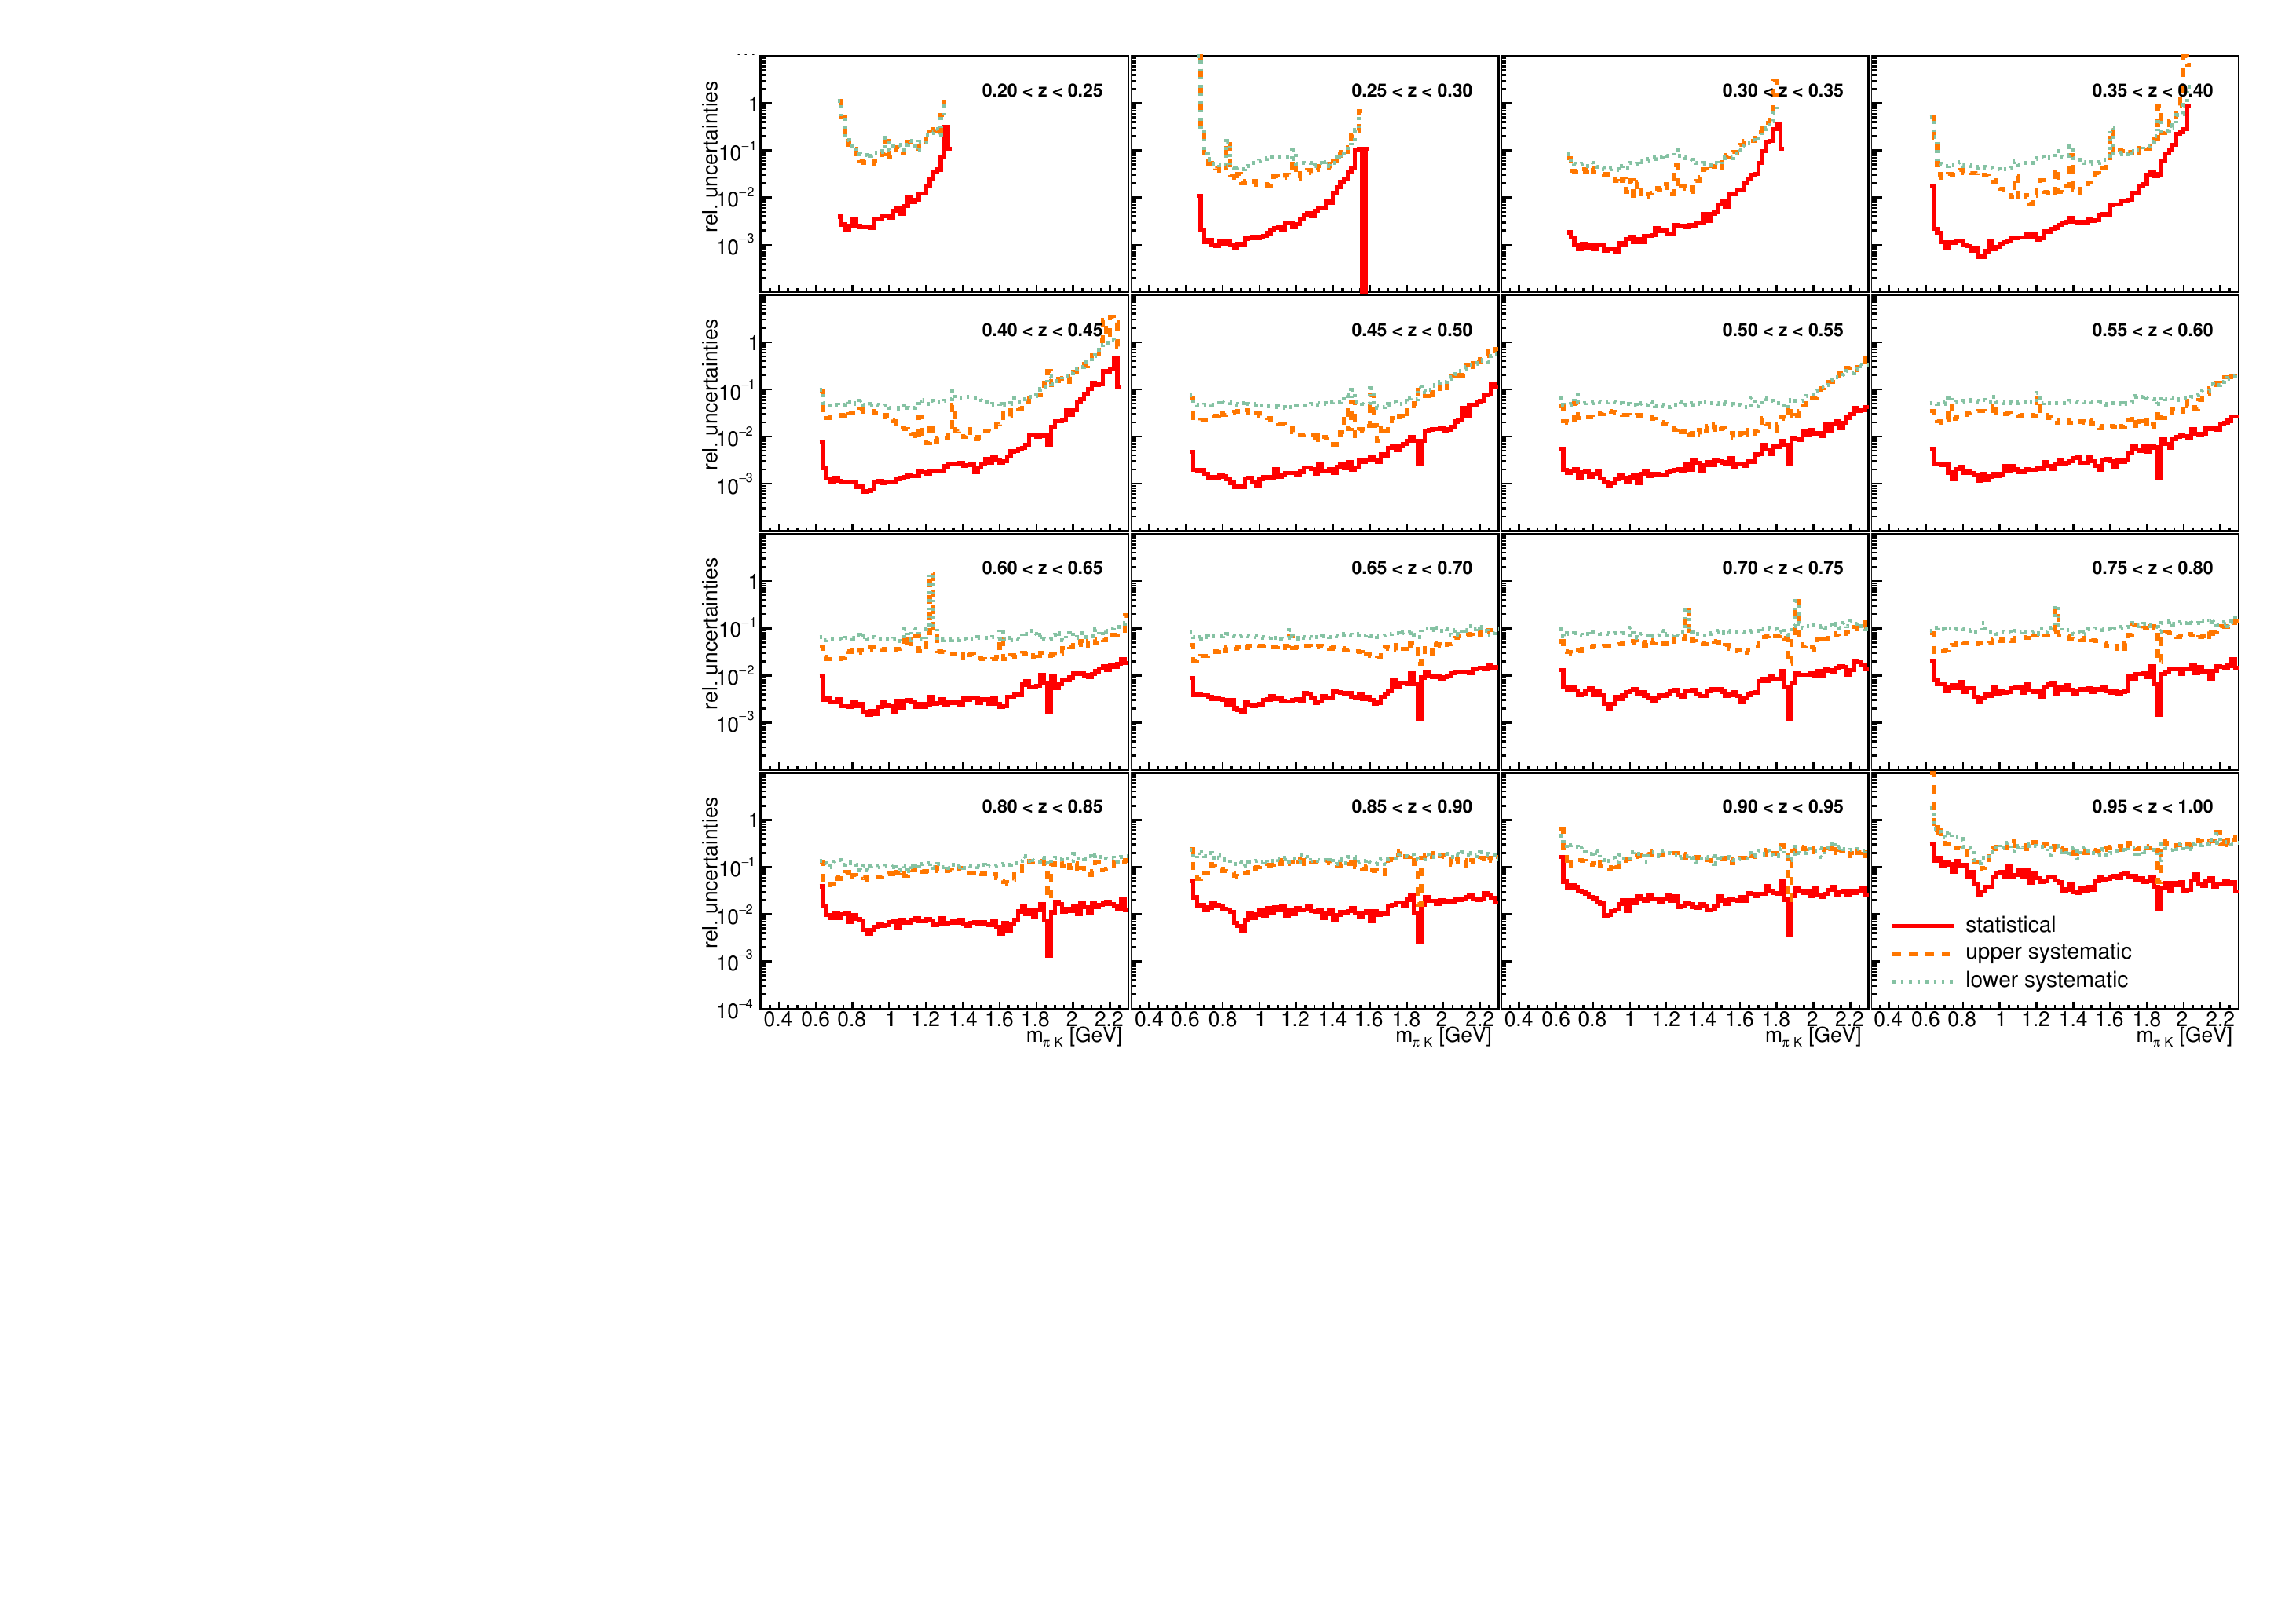}
\caption{\label{fig:systall_pid16} Relative (asymmetric) systematic uncertainties (upper, dashed lines; lower, dotted lines) and statistical uncertainties (full lines) for opposite-sign pion-kaon pairs as a function of $m_{K\pi}$ in bins of $z$.}
\end{center}
\end{figure*}
\begin{figure*}[htb]
\begin{center}
\includegraphics[width=0.8\textwidth]{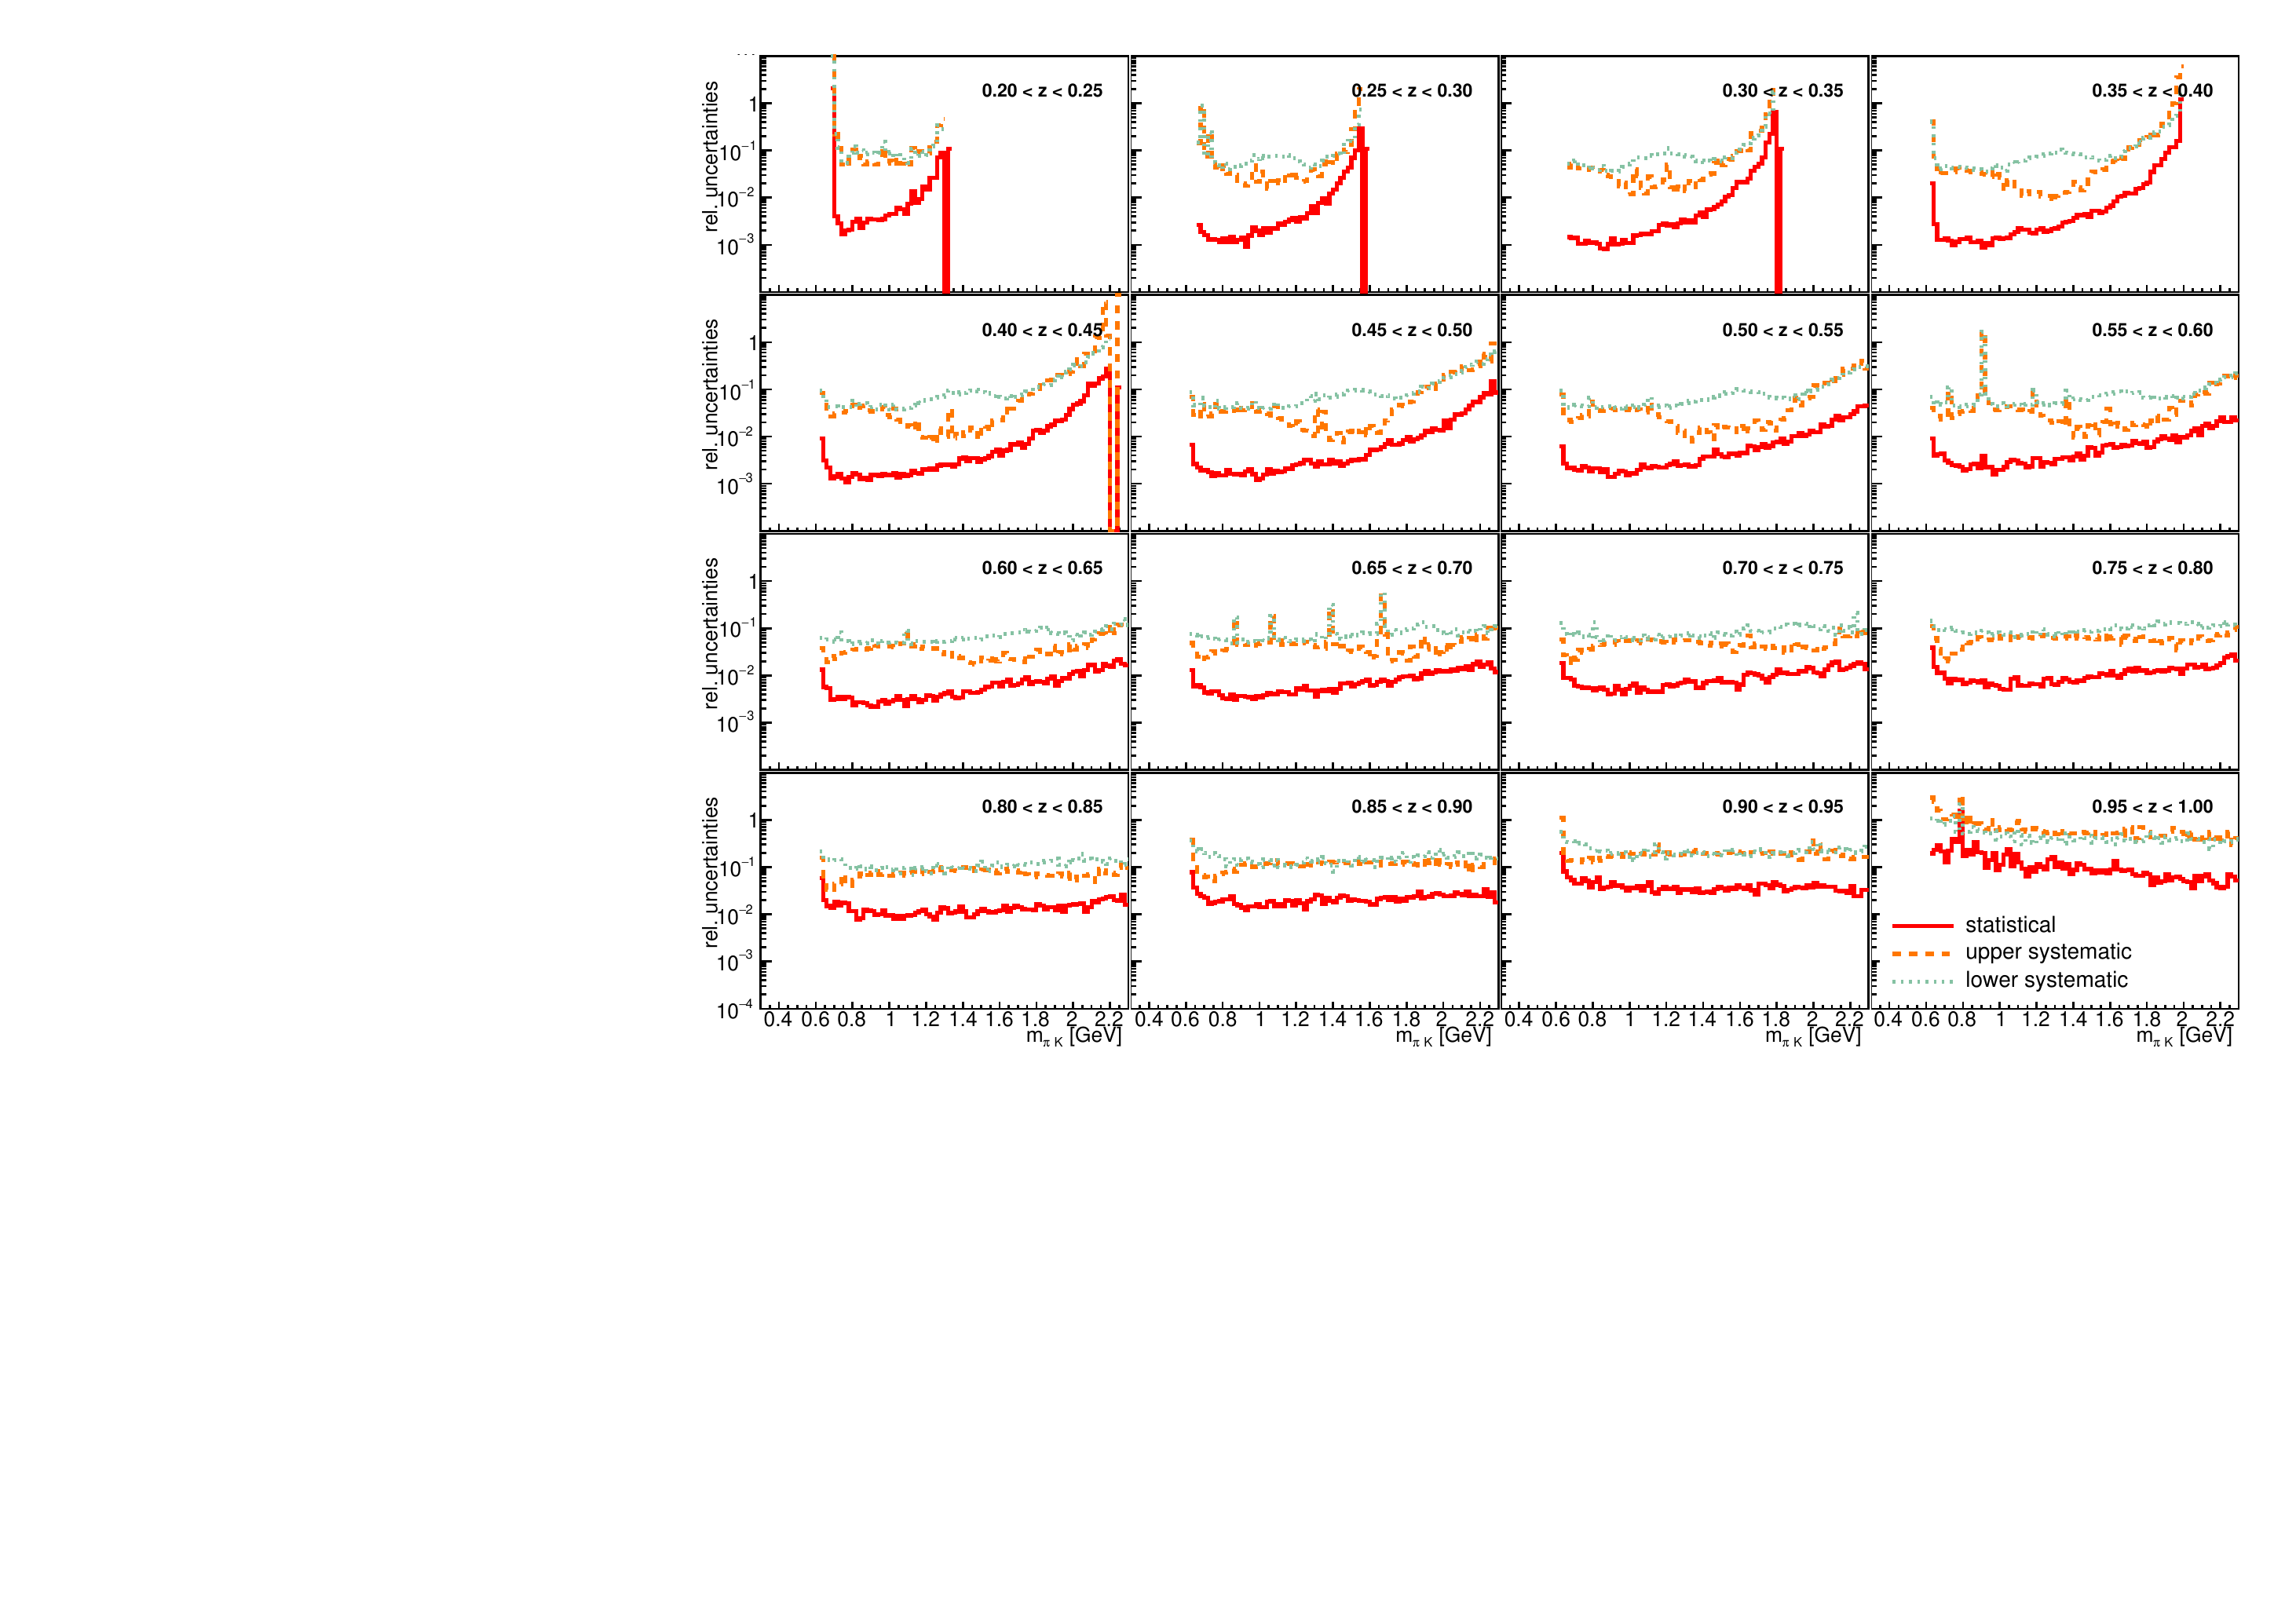}
\caption{\label{fig:systall_pid32} Relative (asymmetric) systematic uncertainties (upper, dashed lines; lower, dotted lines) and statistical uncertainties (full lines) for same-sign pion-kaon pairs as a function of $m_{K\pi}$ in bins of $z$.}
\end{center}
\end{figure*}

\begin{figure*}[htb]
\begin{center}
\includegraphics[width=0.8\textwidth]{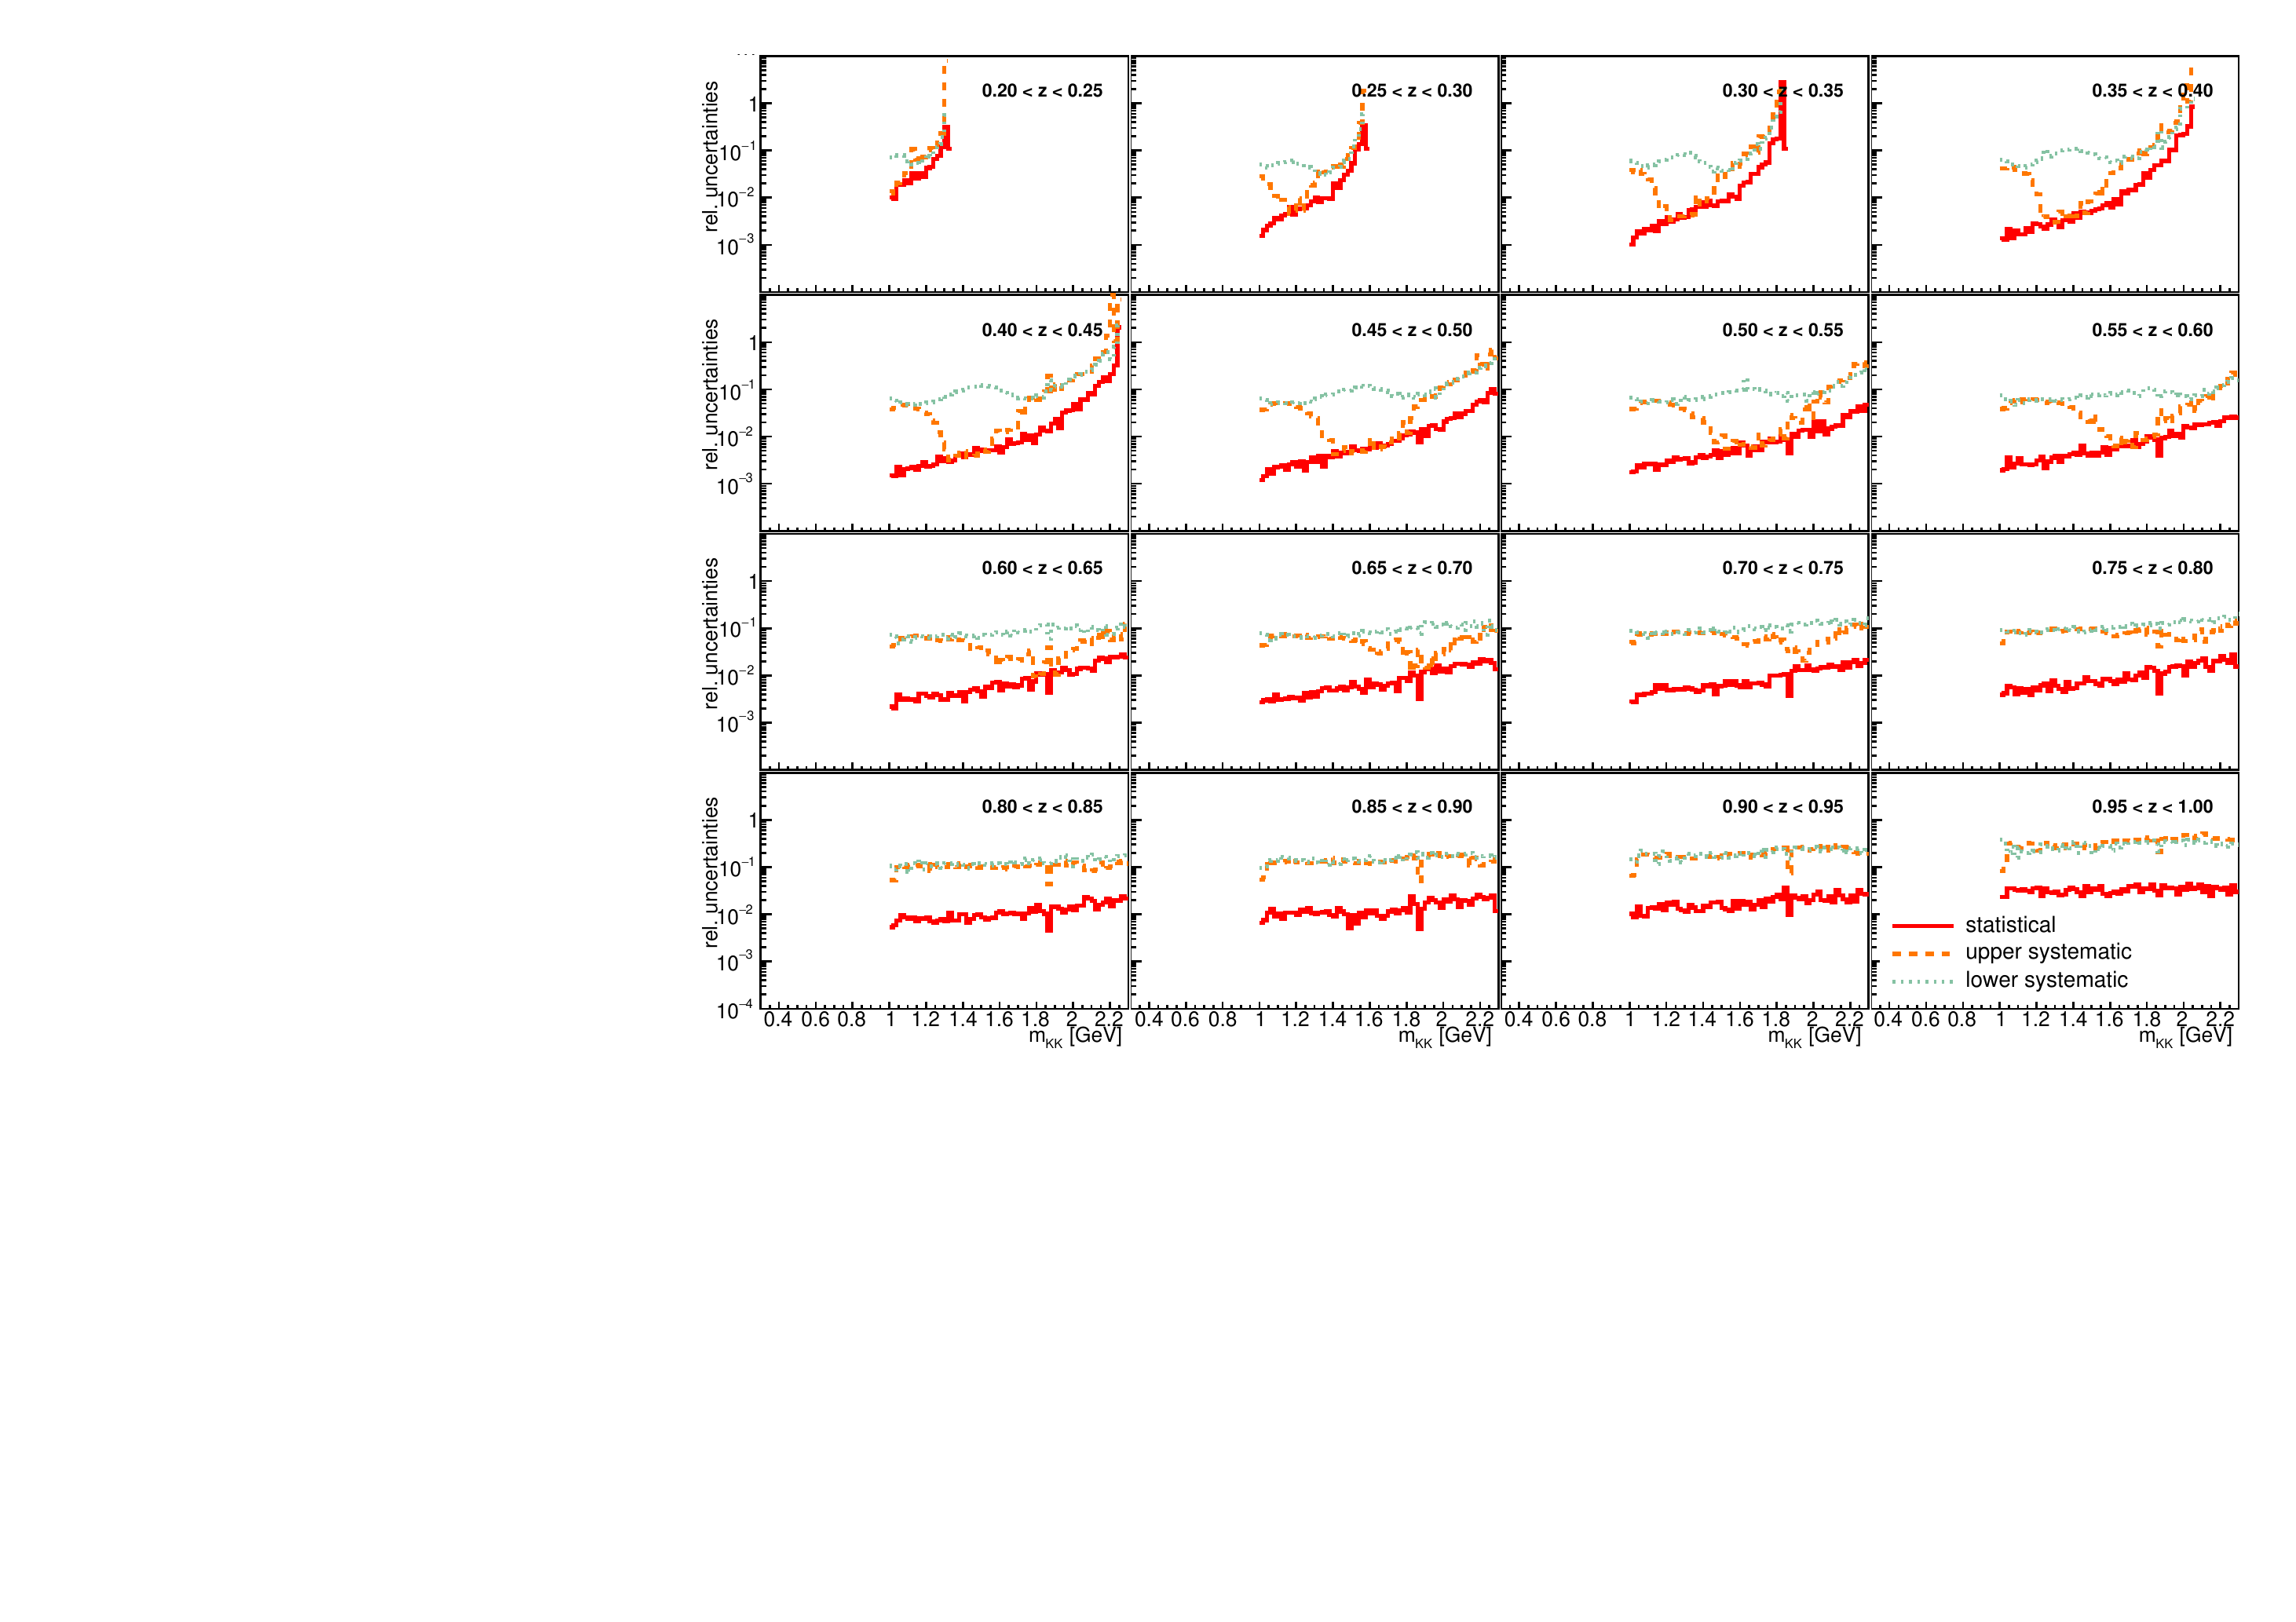}
\caption{\label{fig:systall_pid4096} Relative (asymmetric) systematic uncertainties (upper, dashed lines; lower, dotted lines) and statistical uncertainties (full lines) for opposite-sign kaon pairs as a function of $m_{KK}$ in bins of $z$.}
\end{center}
\end{figure*}
\begin{figure*}[htb]
\begin{center}
\includegraphics[width=0.8\textwidth]{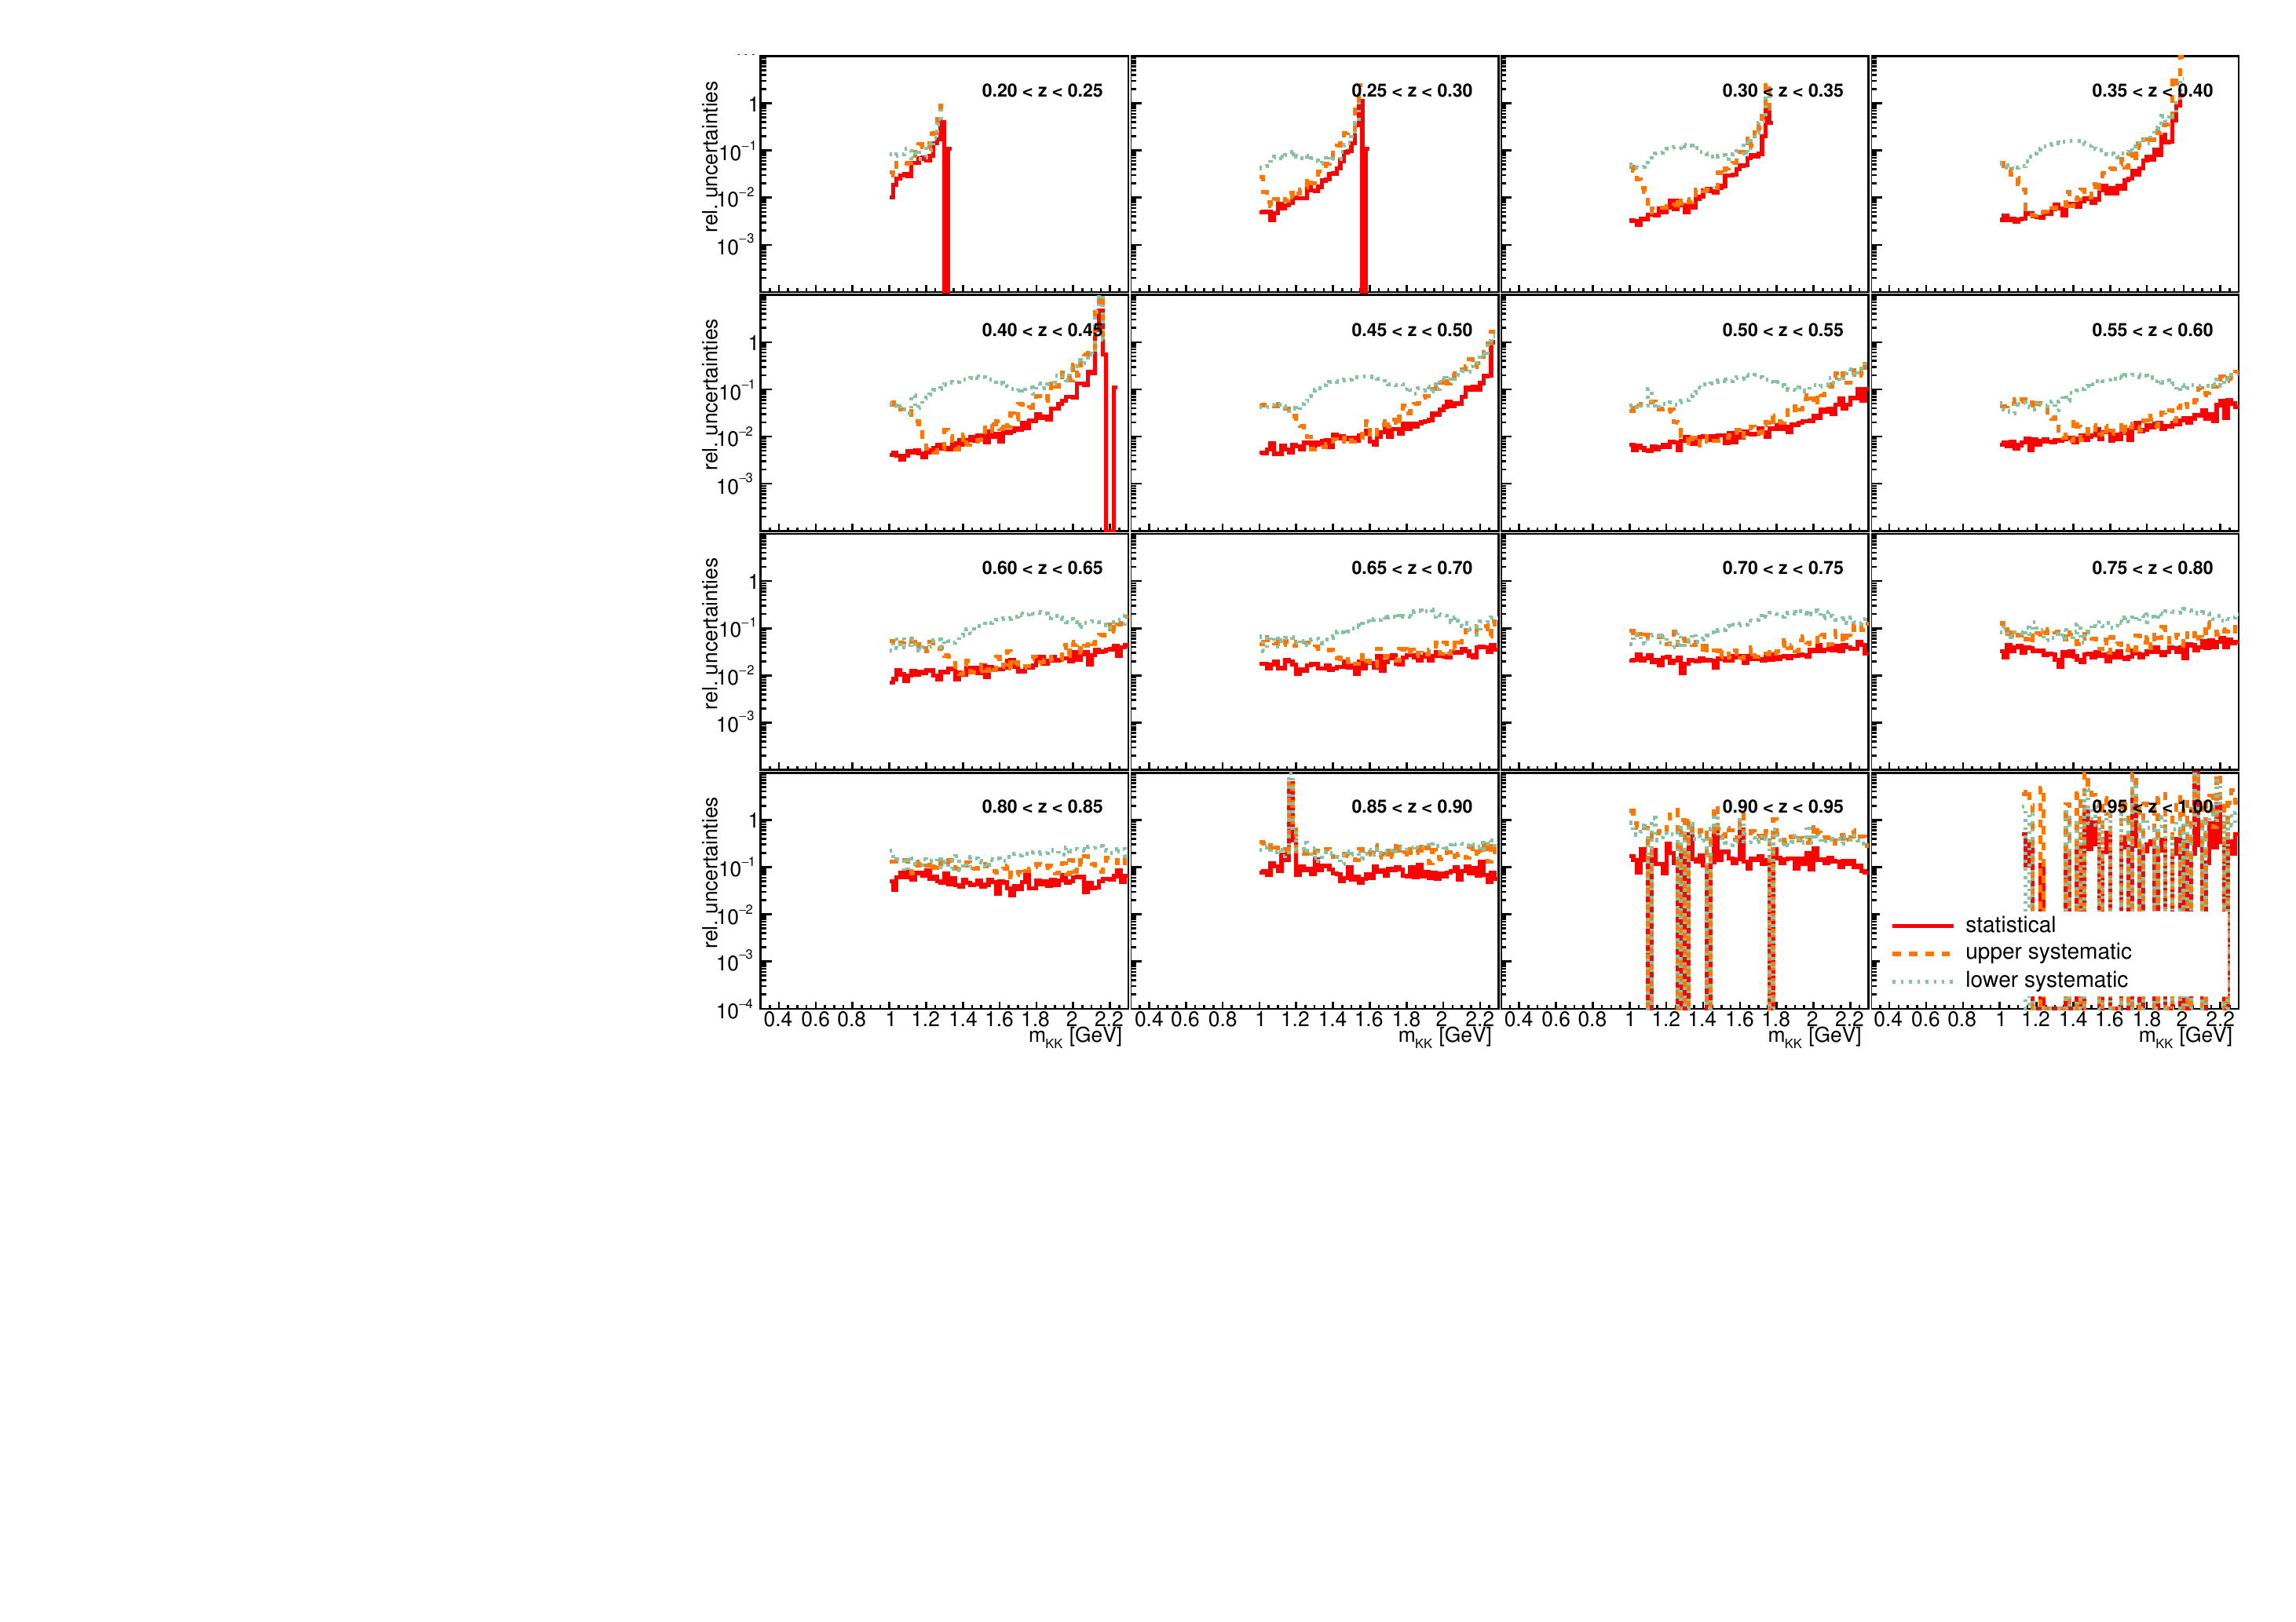}
\caption{\label{fig:systall_pid8192} Relative (asymmetric) systematic uncertainties (upper, dashed lines; lower, dotted lines) and statistical uncertainties (full lines) for same-sign kaon pairs as a function of $m_{KK}$ in bins of $z$.}
\end{center}
\end{figure*}
\clearpage
\subsection{Results}
Figures \ref{fig:results:massdists1} to \ref{fig:results:massdists13} compare the final cross sections with MC simulations indicating the origin of the various peaks for same-sign hadron paris as well as opposite-sign pion-kaon and kaon pairs. 

\begin{figure*}[htb]
\begin{center}
\includegraphics[width=0.9\textwidth]{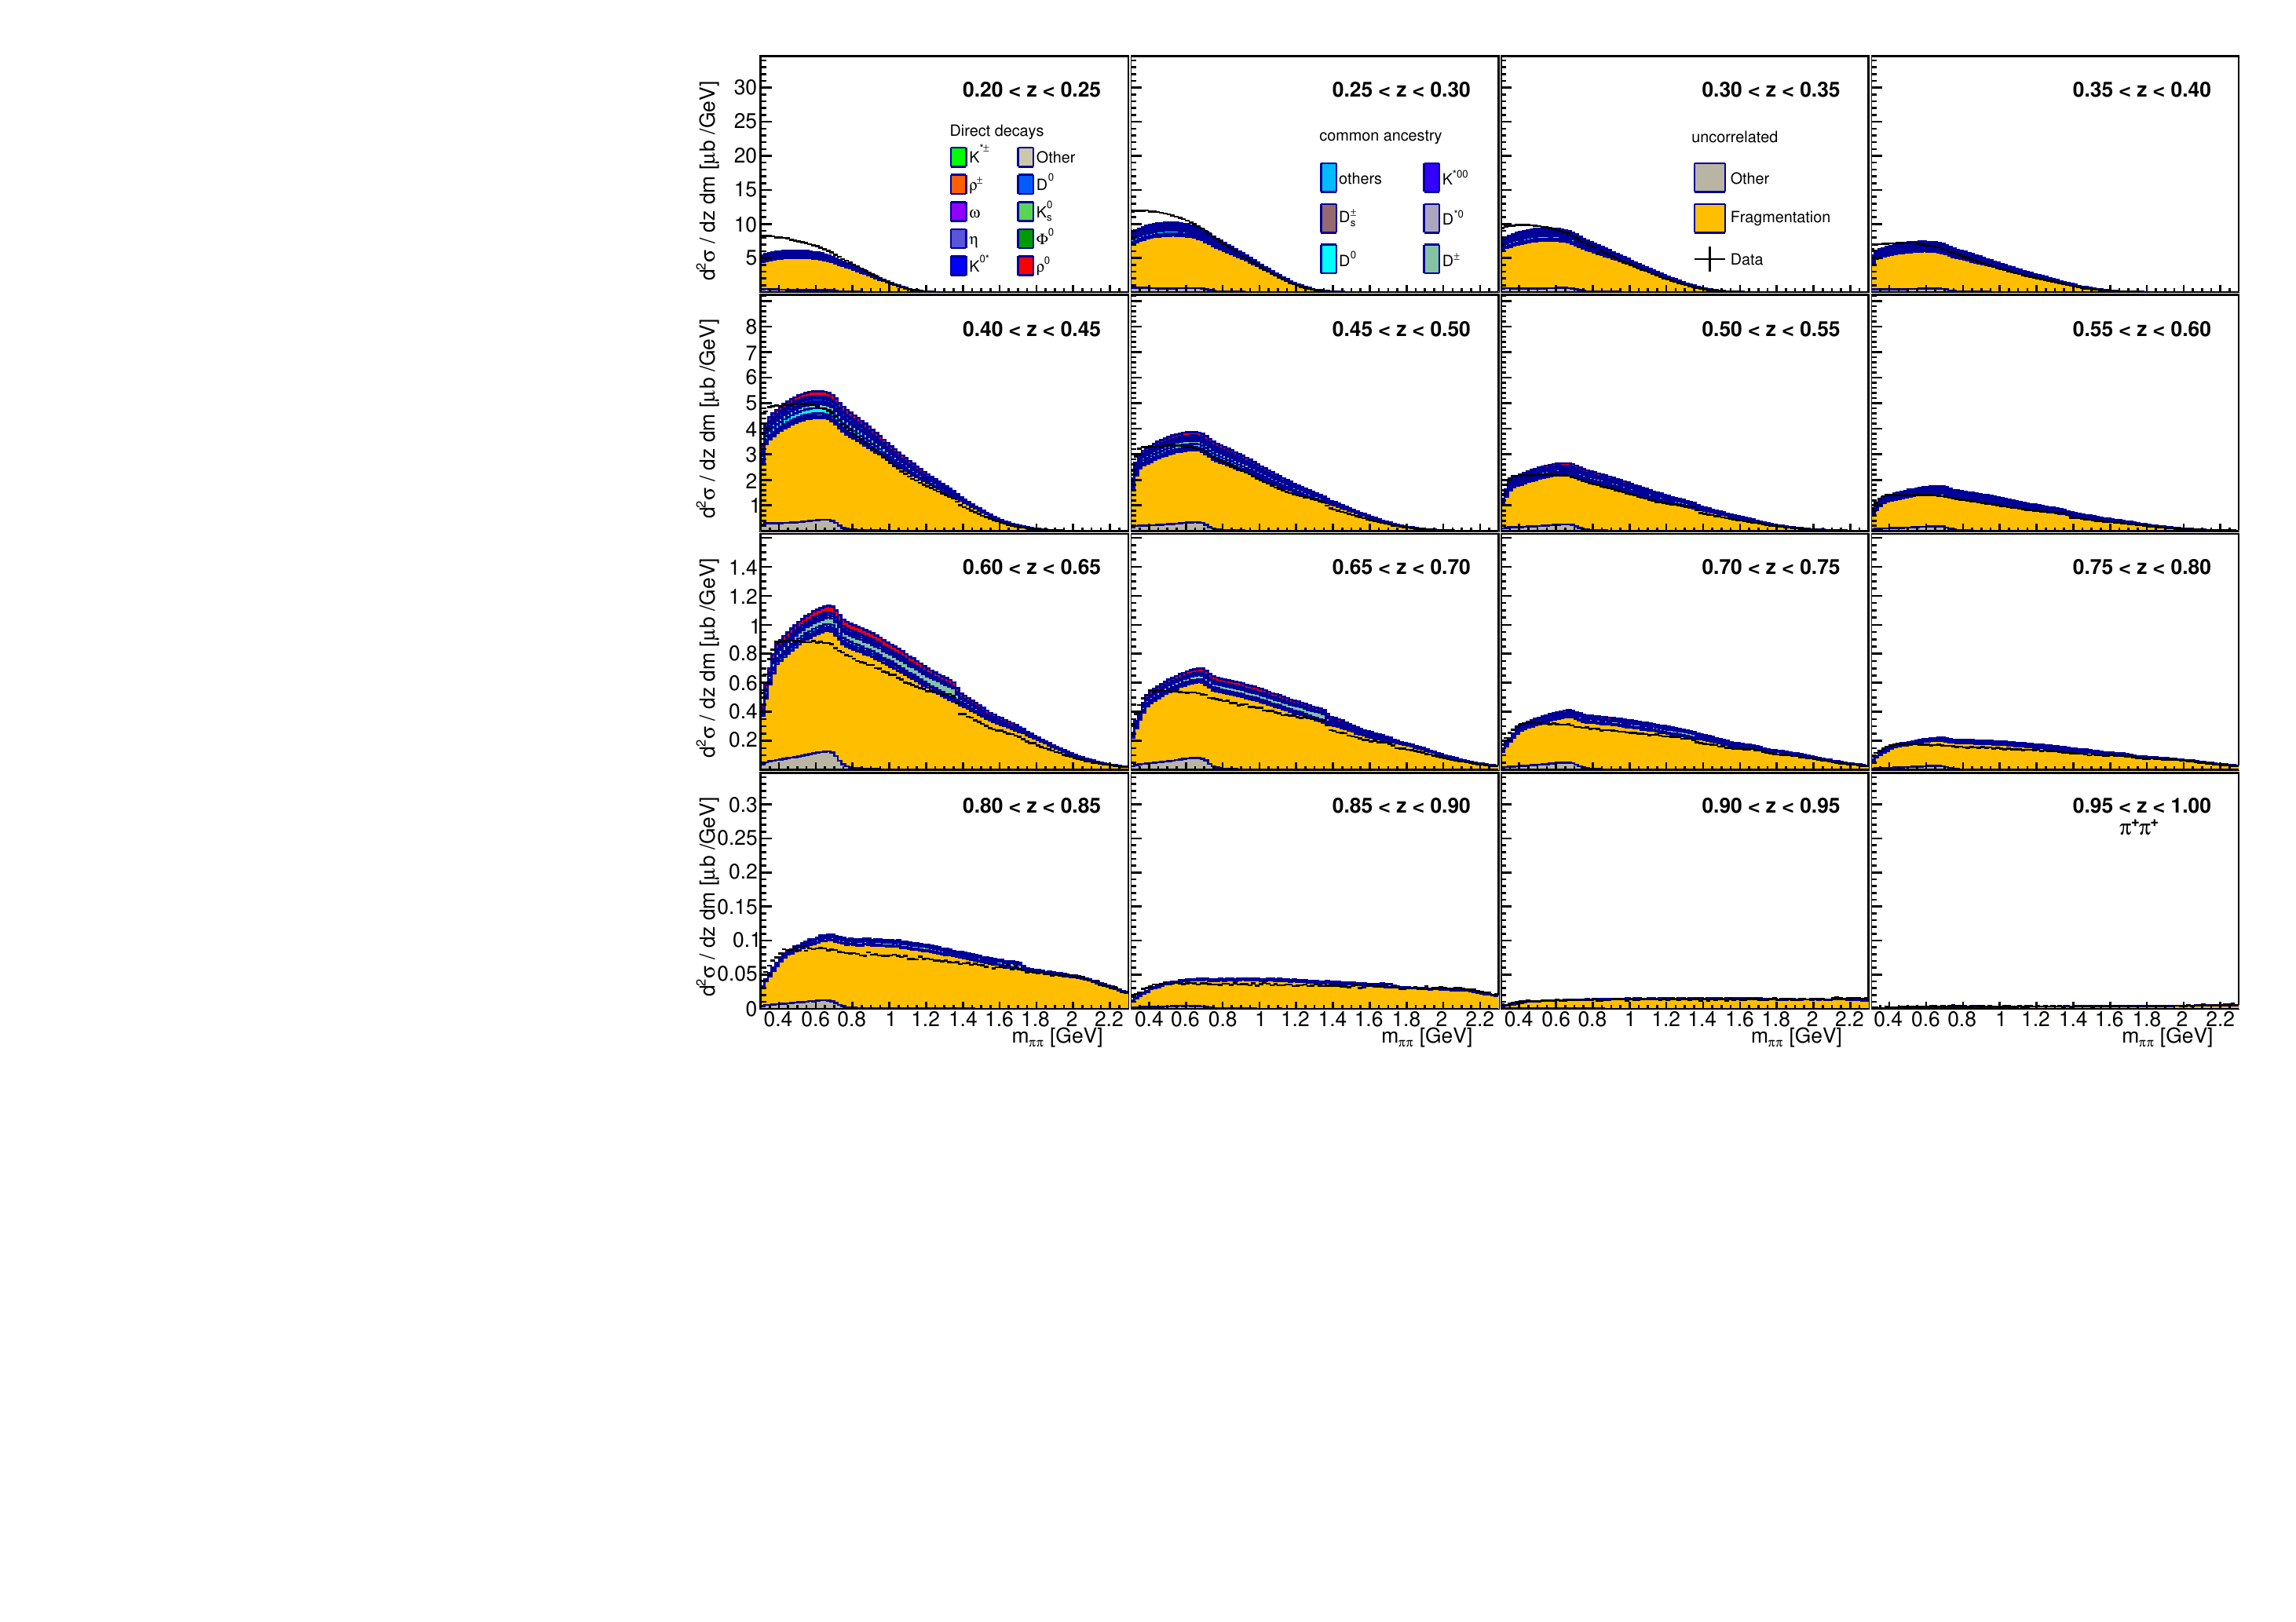}
\includegraphics[width=0.9\textwidth]{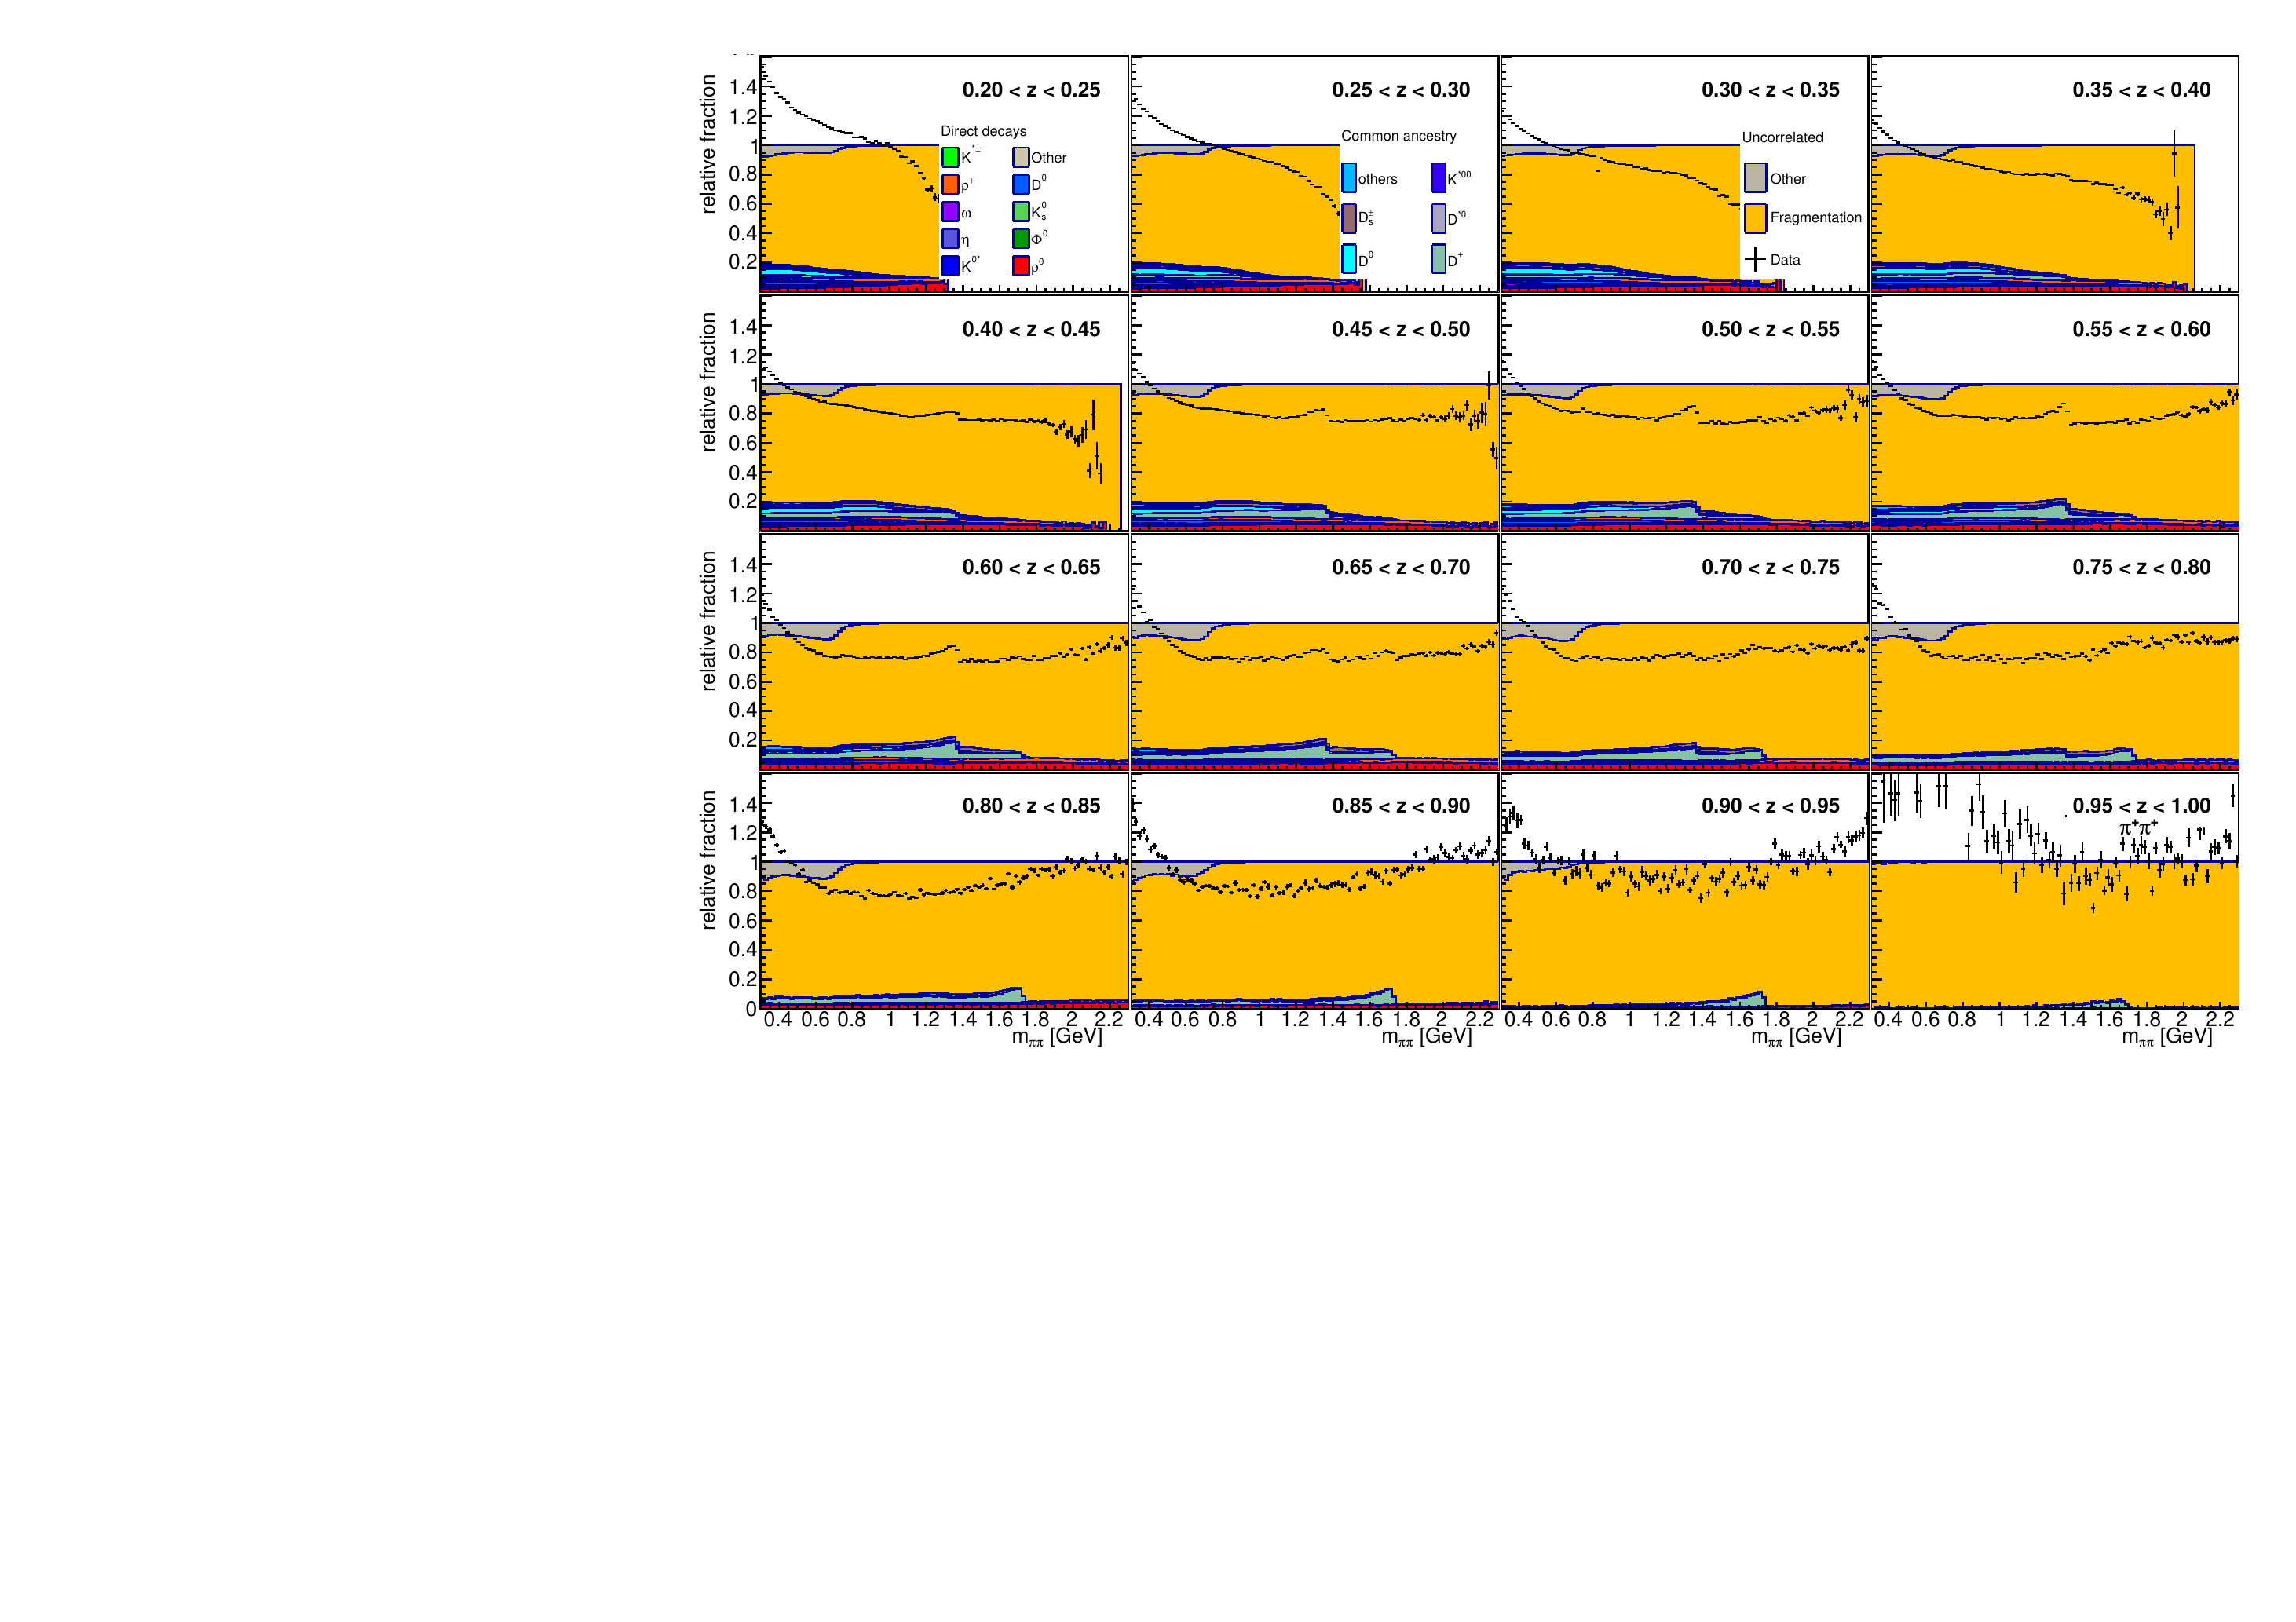}

\caption{\label{fig:results:massdists1} MC decomposition of the same-sign pion pairs as a function of $m_{\pi\pi}$ in bins of $z$ for various resonance, partial resonant and non-resonant parents, displayed in linear scale (top) and as a relative fraction of the total cross section (bottom).}
\end{center}
\end{figure*}

\begin{figure*}[htb]
\begin{center}
\includegraphics[width=0.9\textwidth]{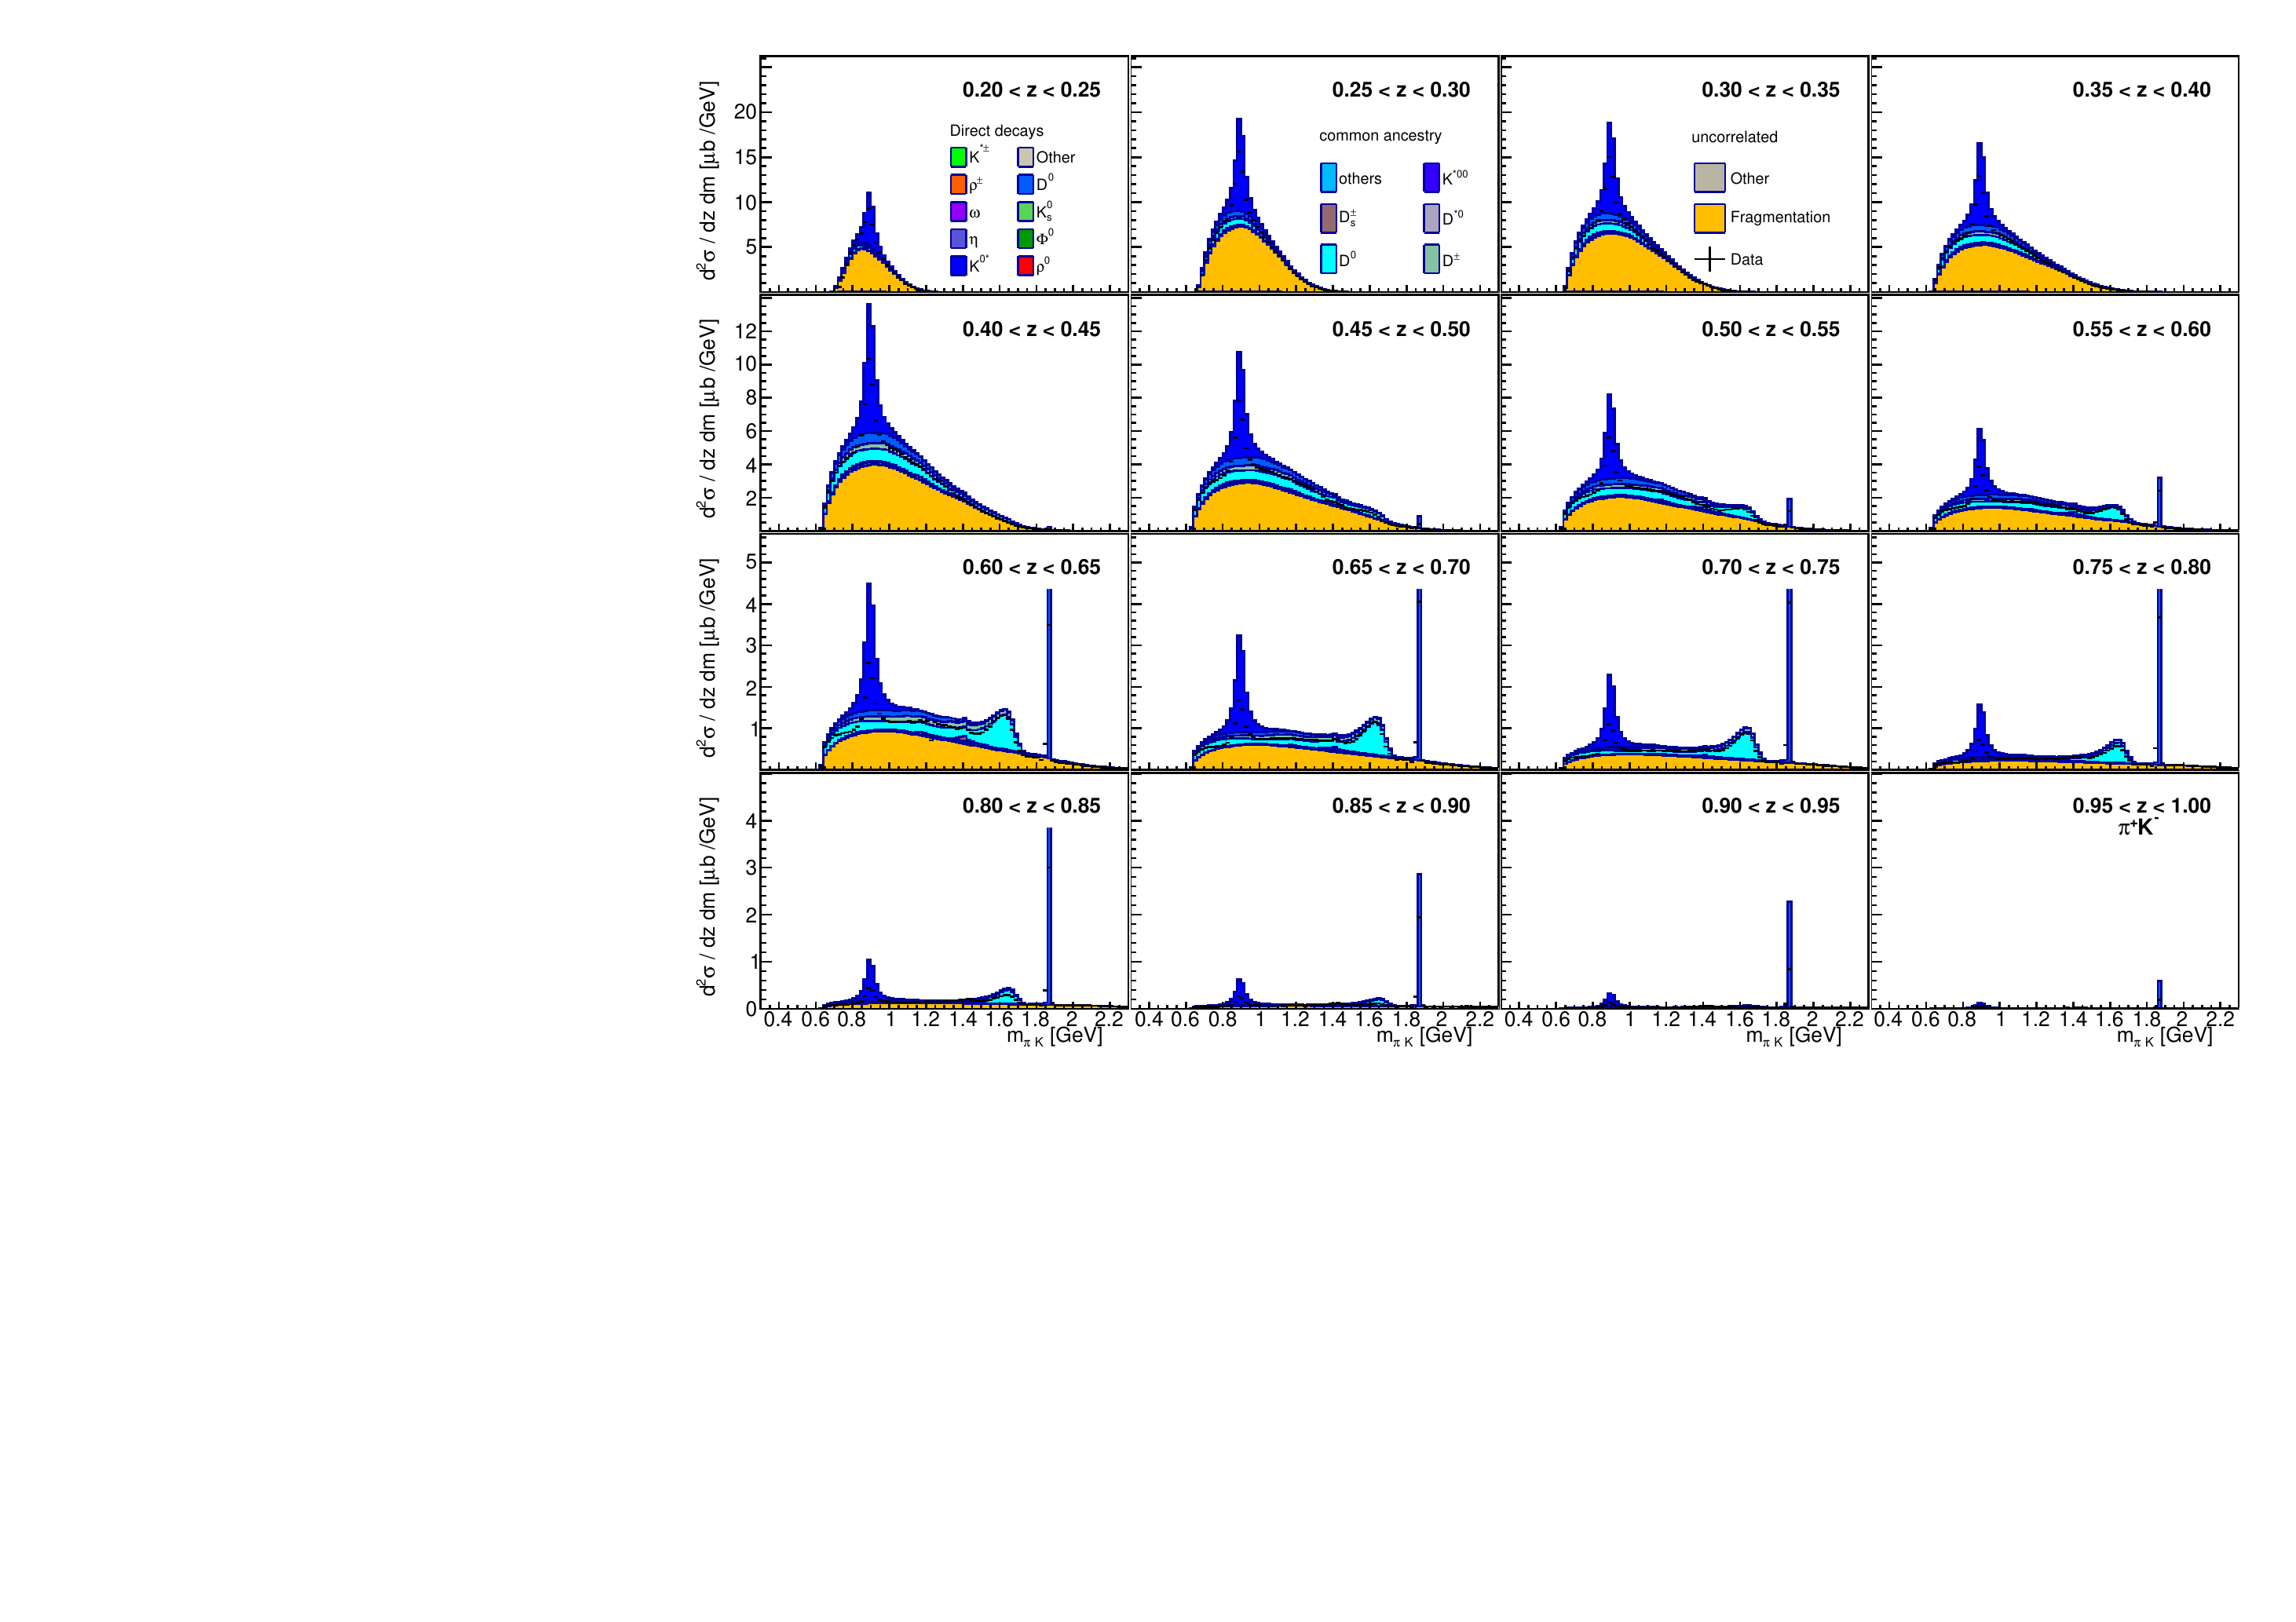}
\includegraphics[width=0.9\textwidth]{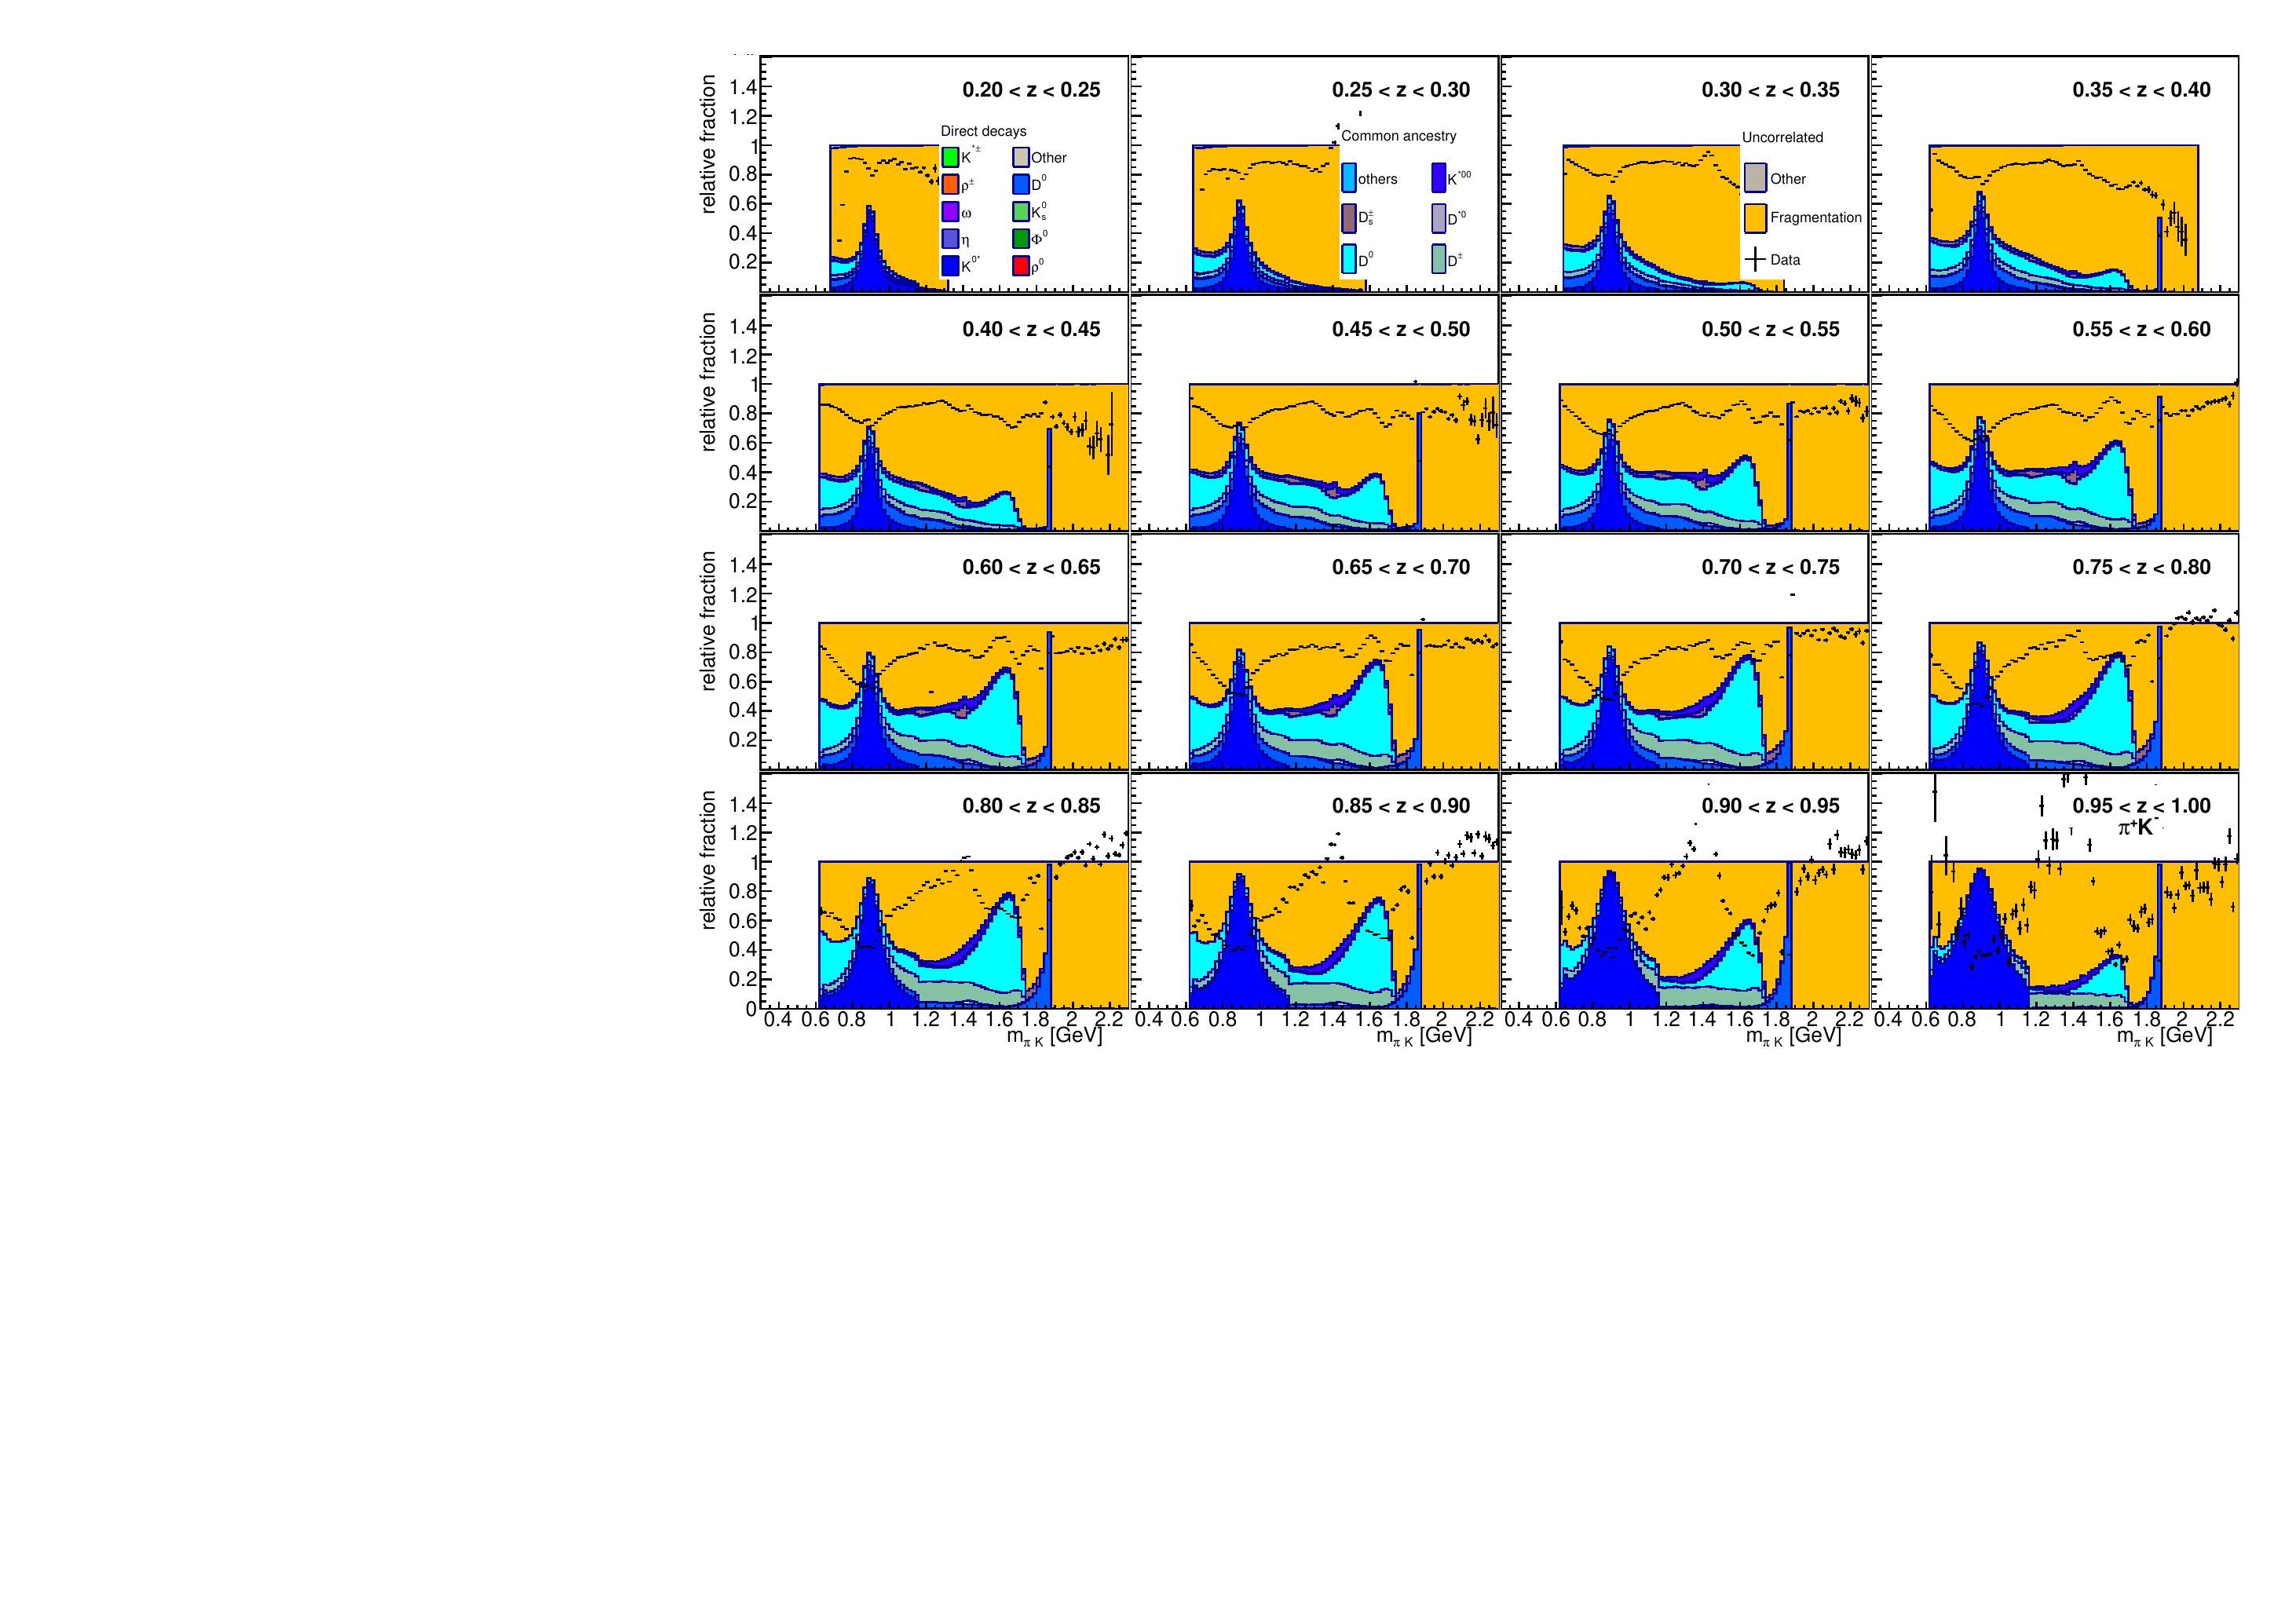}

\caption{\label{fig:results:massdists4} MC decomposition of the opposite-sign pion-kaon pairs as a function of $m_{K\pi}$ in bins of $z$ for various resonance, partial resonant and non-resonant parents, displayed in linear scale (top) and as a relative fraction of the total cross section (bottom).}
\end{center}
\end{figure*}

\begin{figure*}[htb]
\begin{center}
\includegraphics[width=0.9\textwidth]{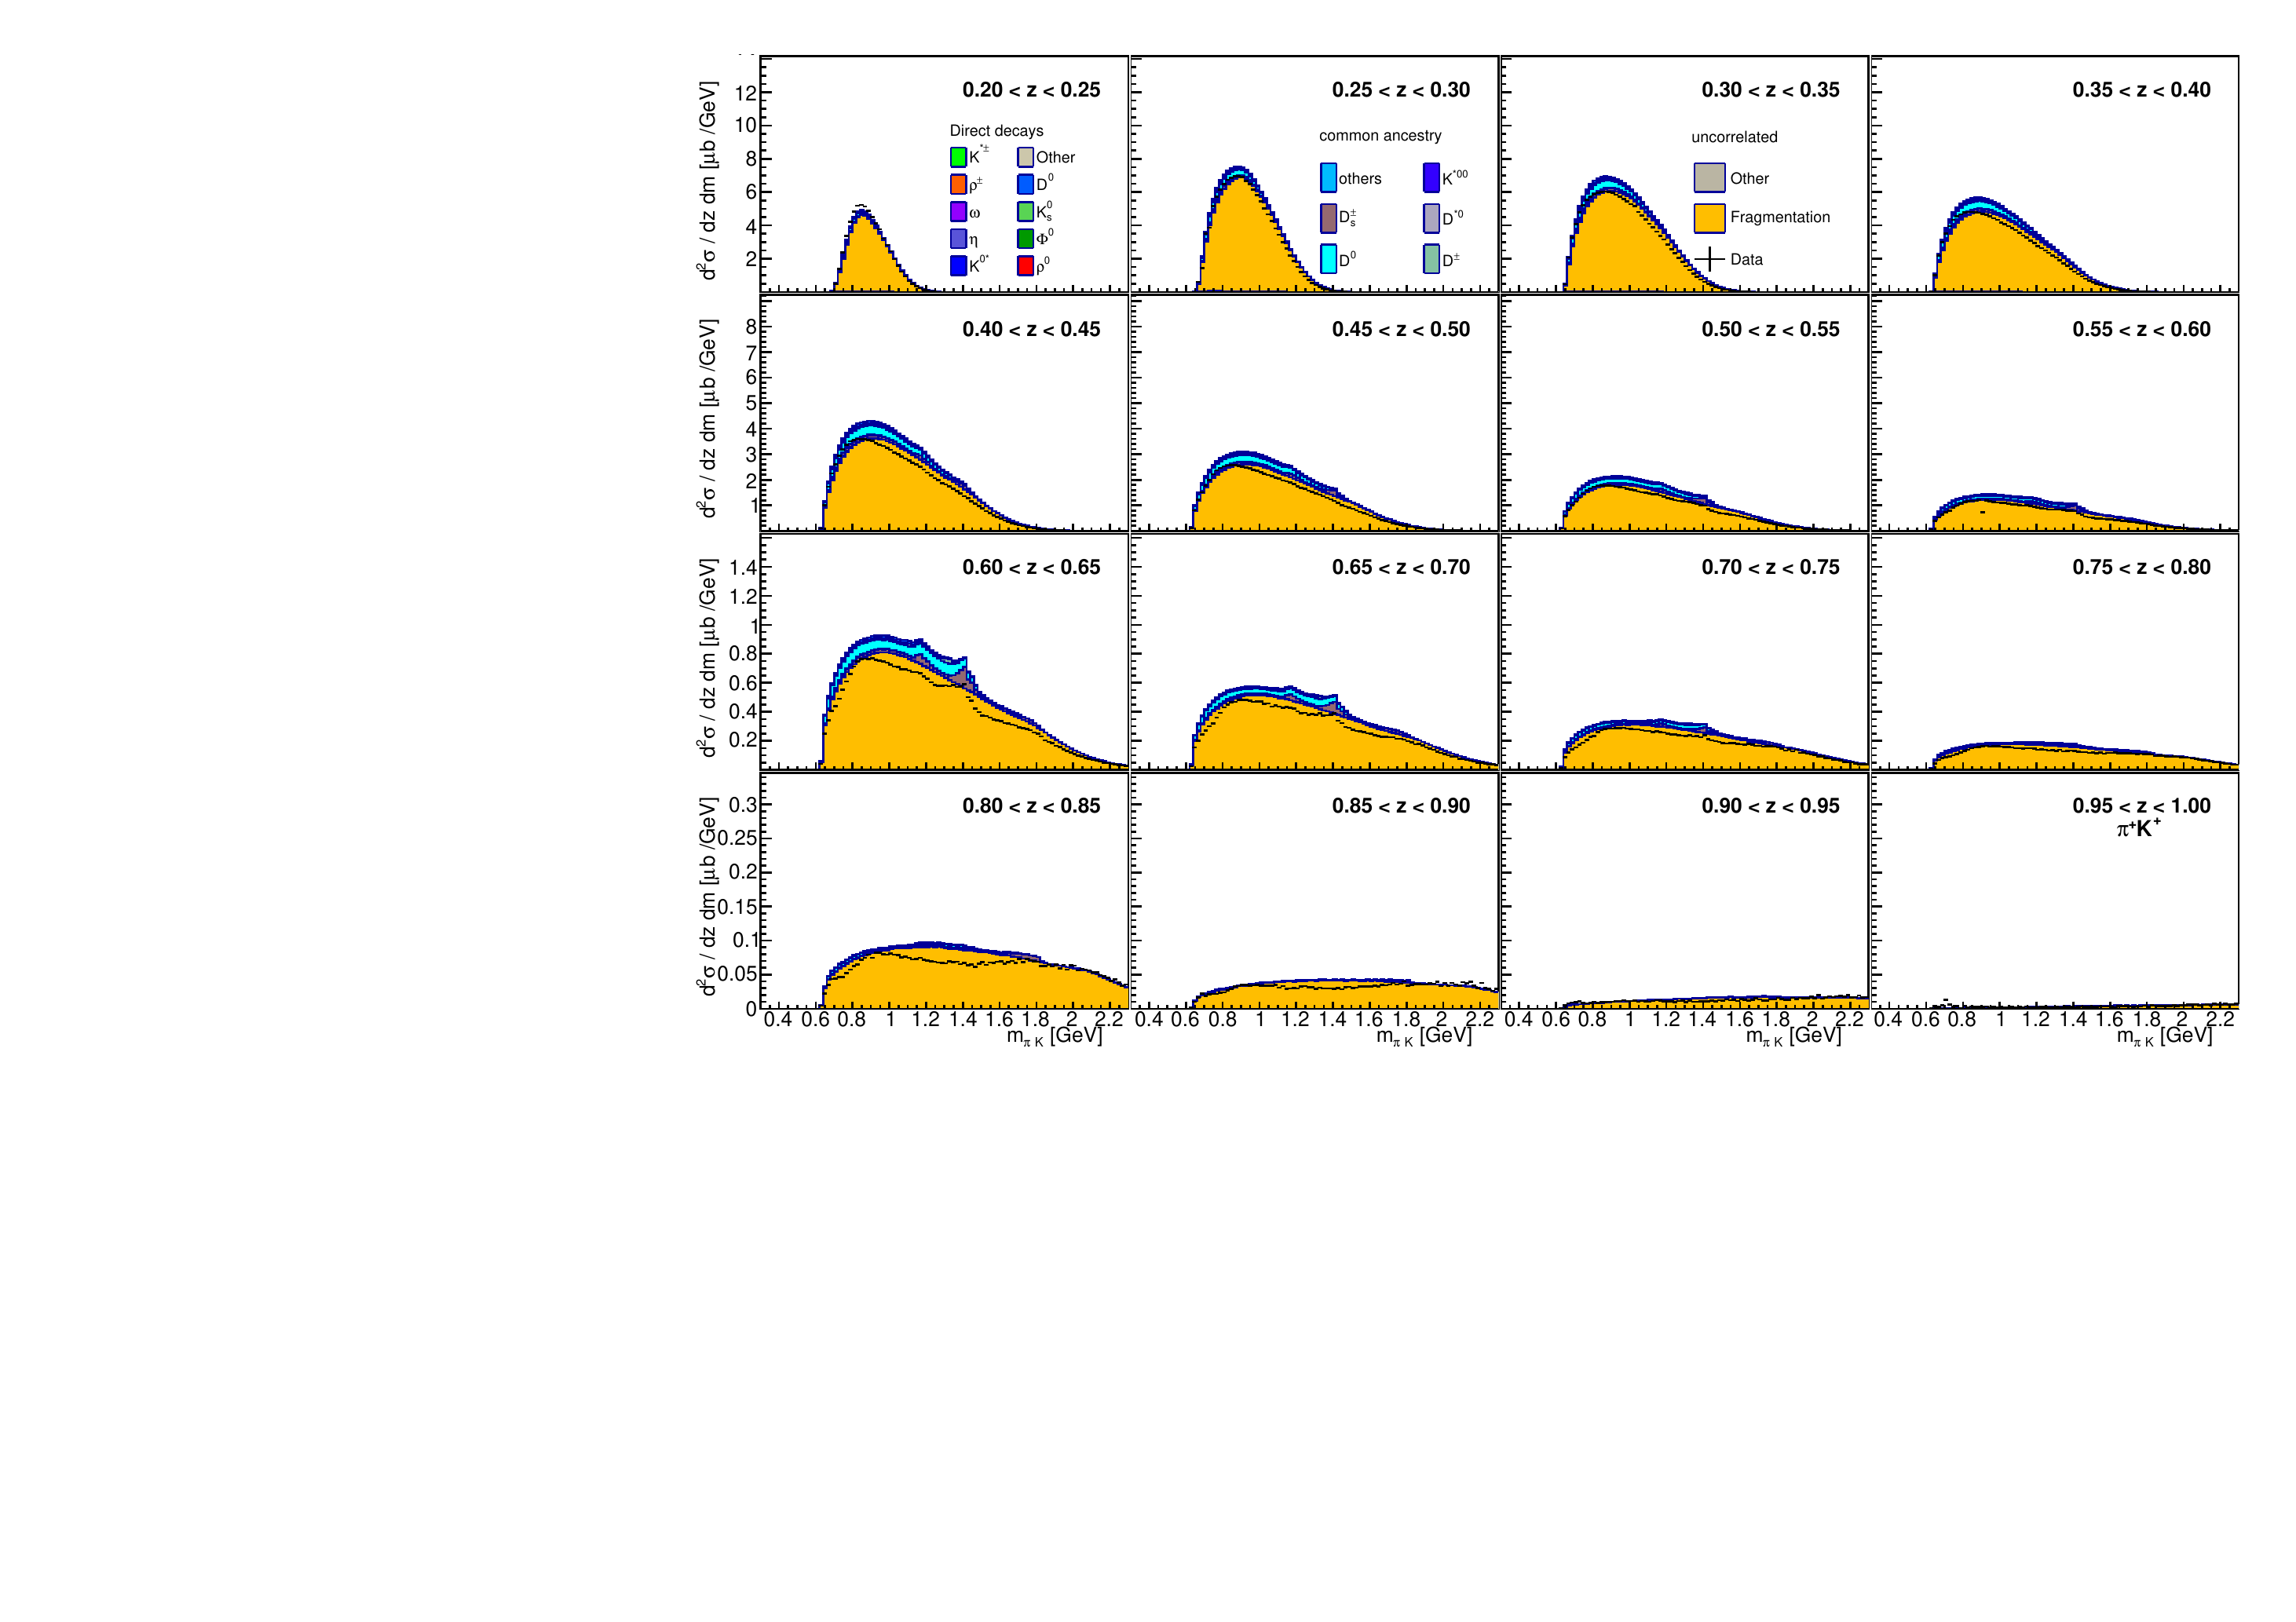}
\includegraphics[width=0.9\textwidth]{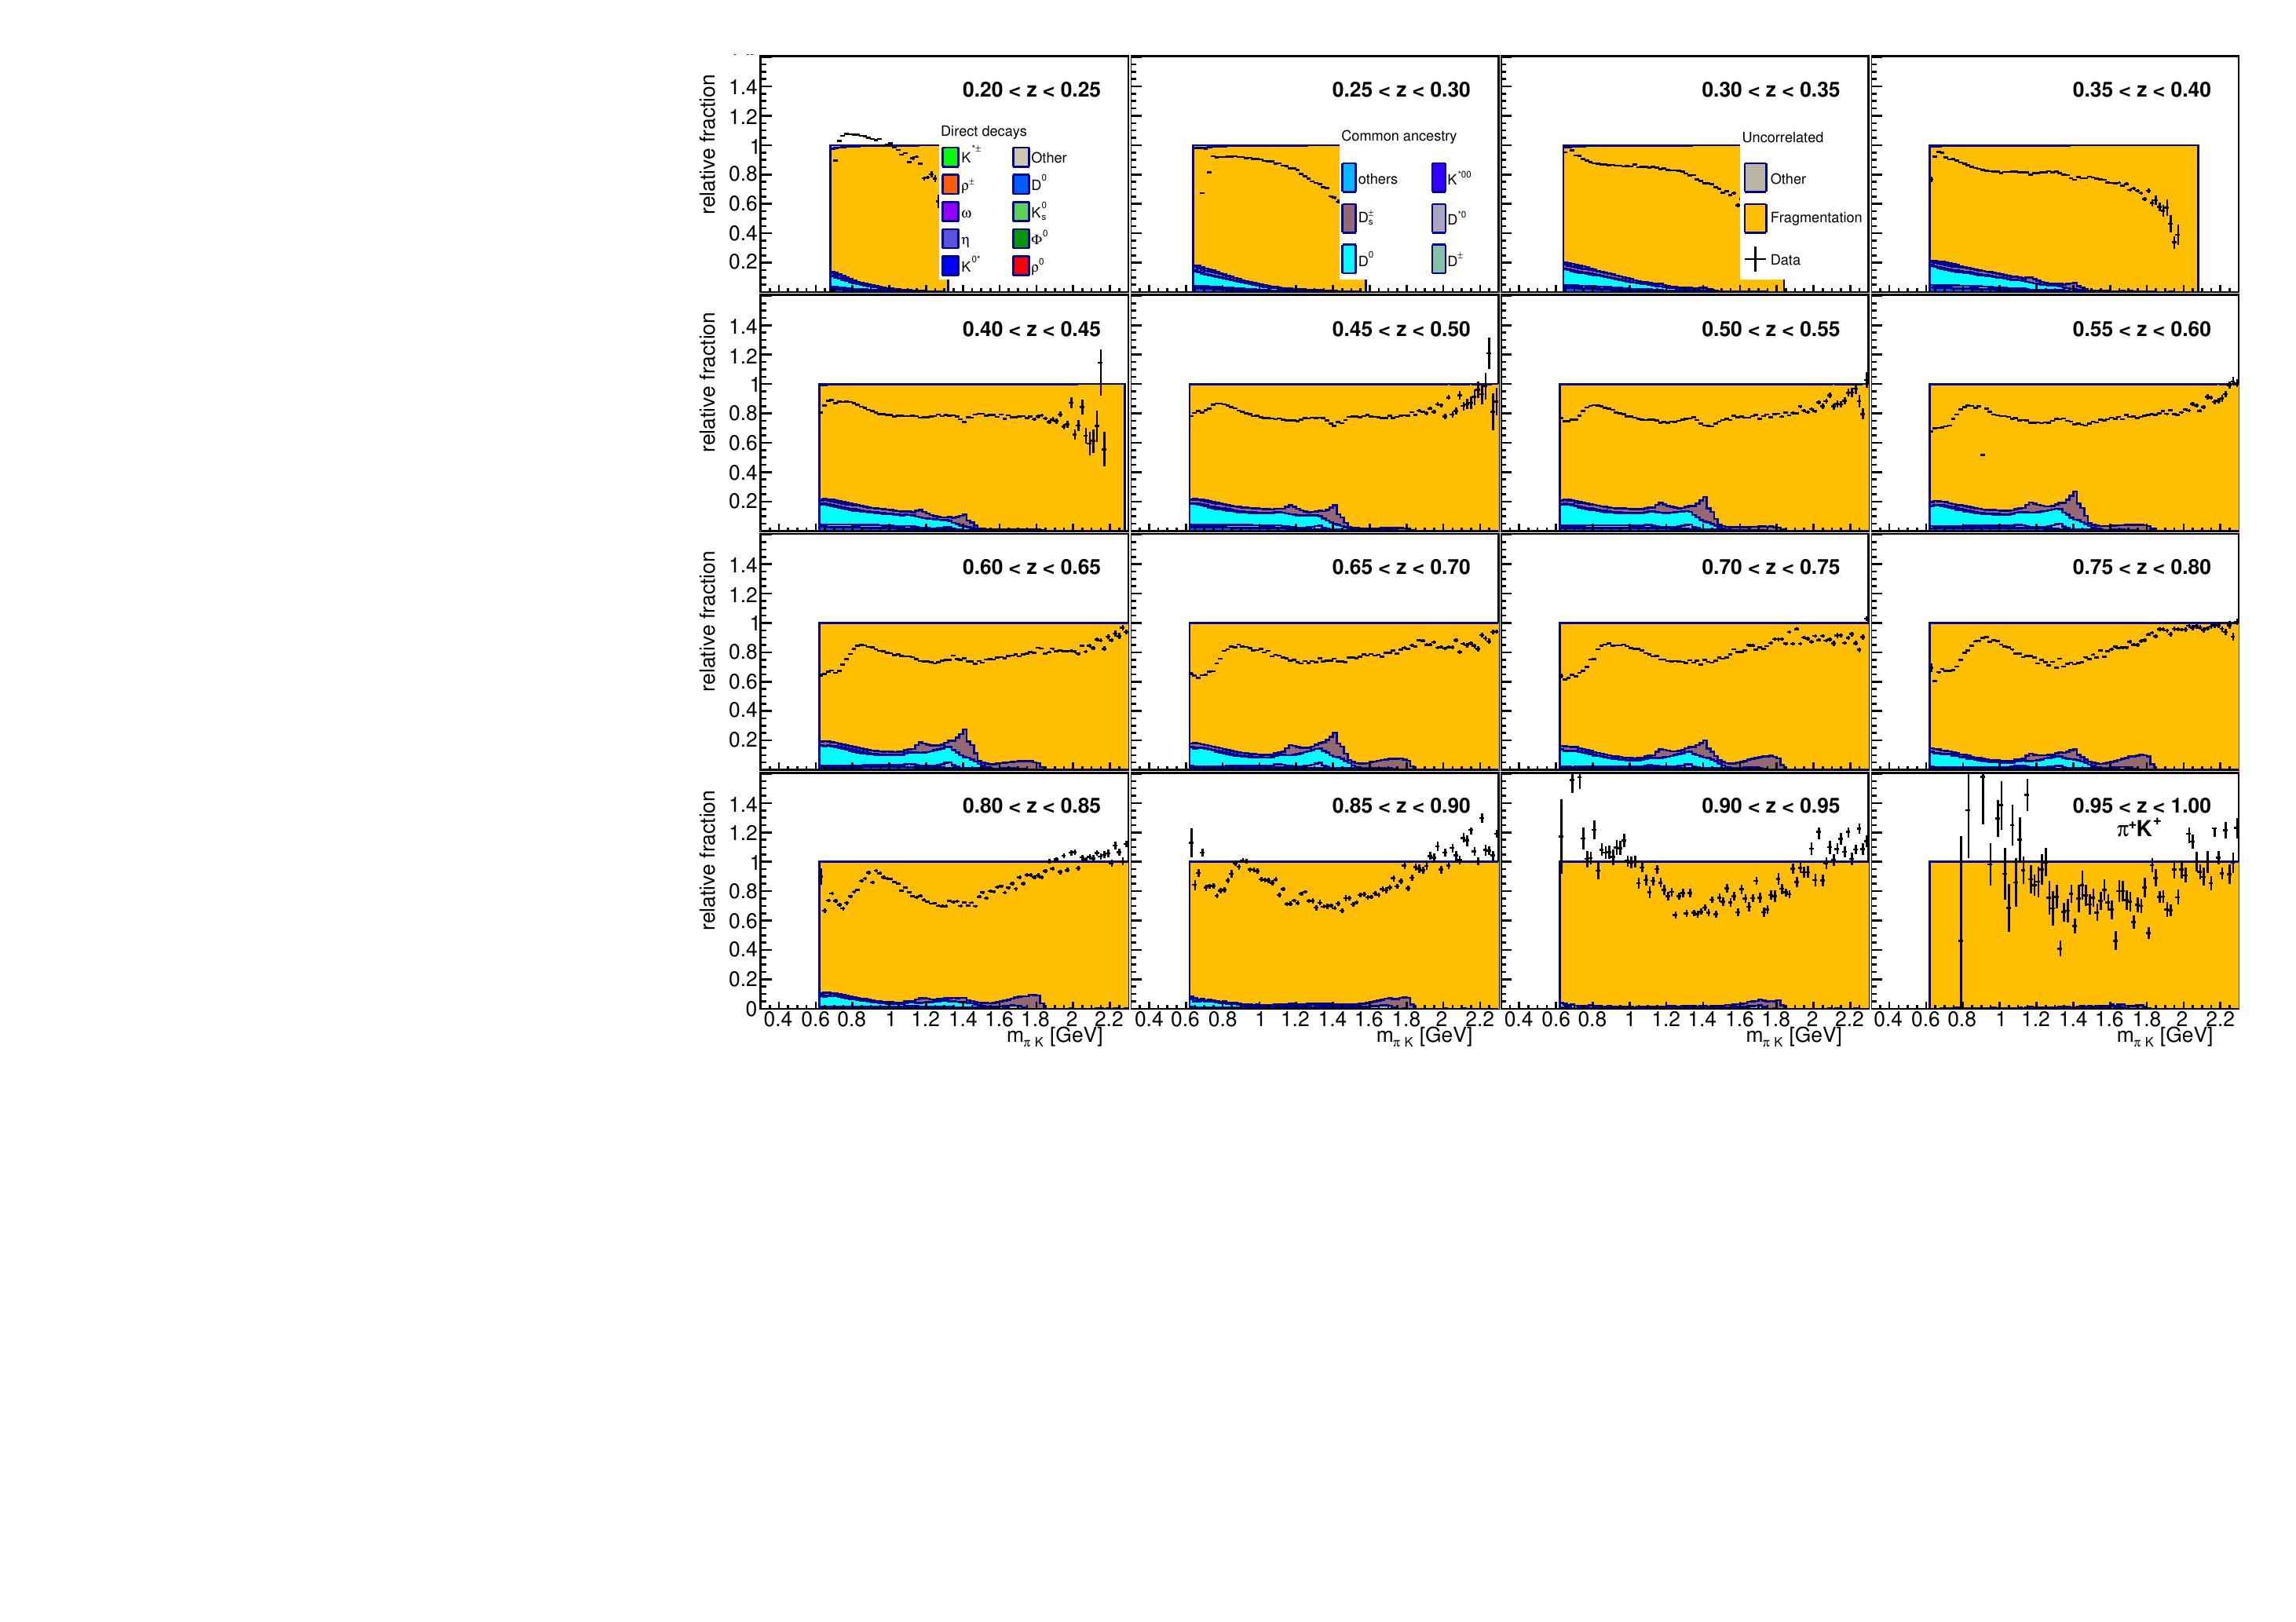}

\caption{\label{fig:results:massdists5} MC decomposition of the same-sign pion-kaon pairs as a function of $m_{K\pi}$ in bins of $z$ for various resonance, partial resonant and non-resonant parents, displayed in linear scale (top) and as a relative fraction of the total cross section (bottom).}
\end{center}
\end{figure*}

\begin{figure*}[htb]
\begin{center}
\includegraphics[width=0.9\textwidth]{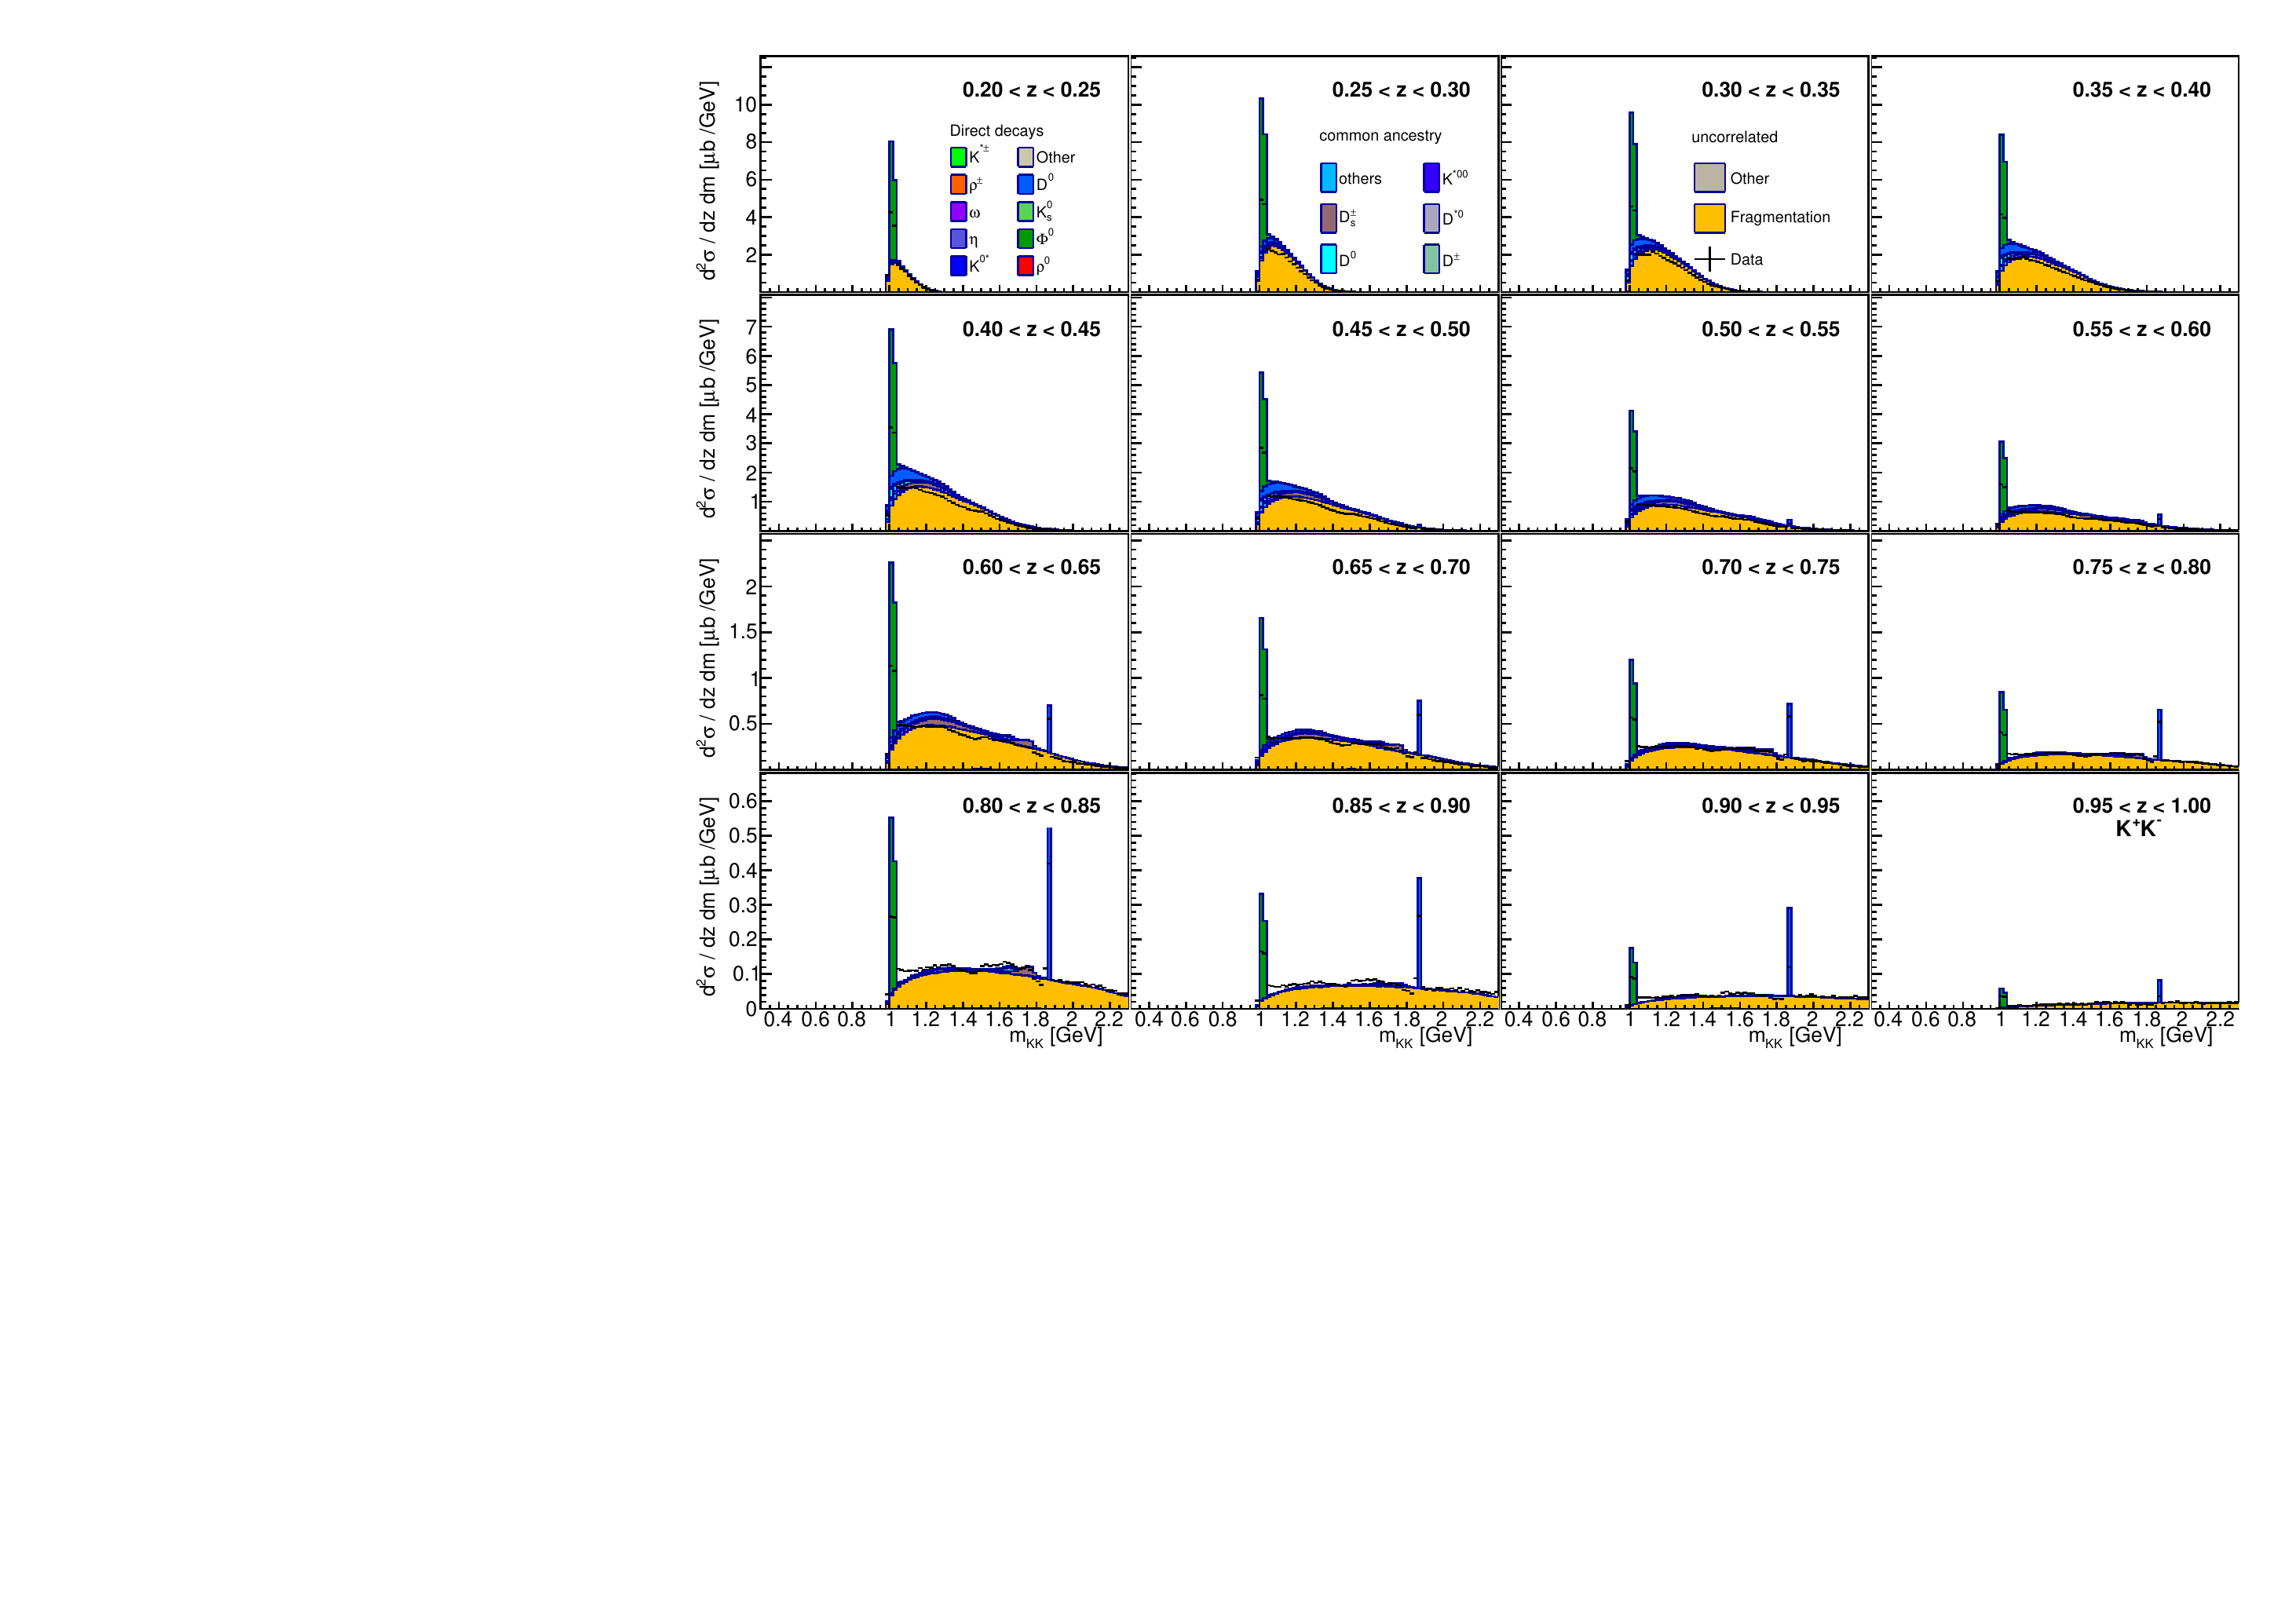}
\includegraphics[width=0.9\textwidth]{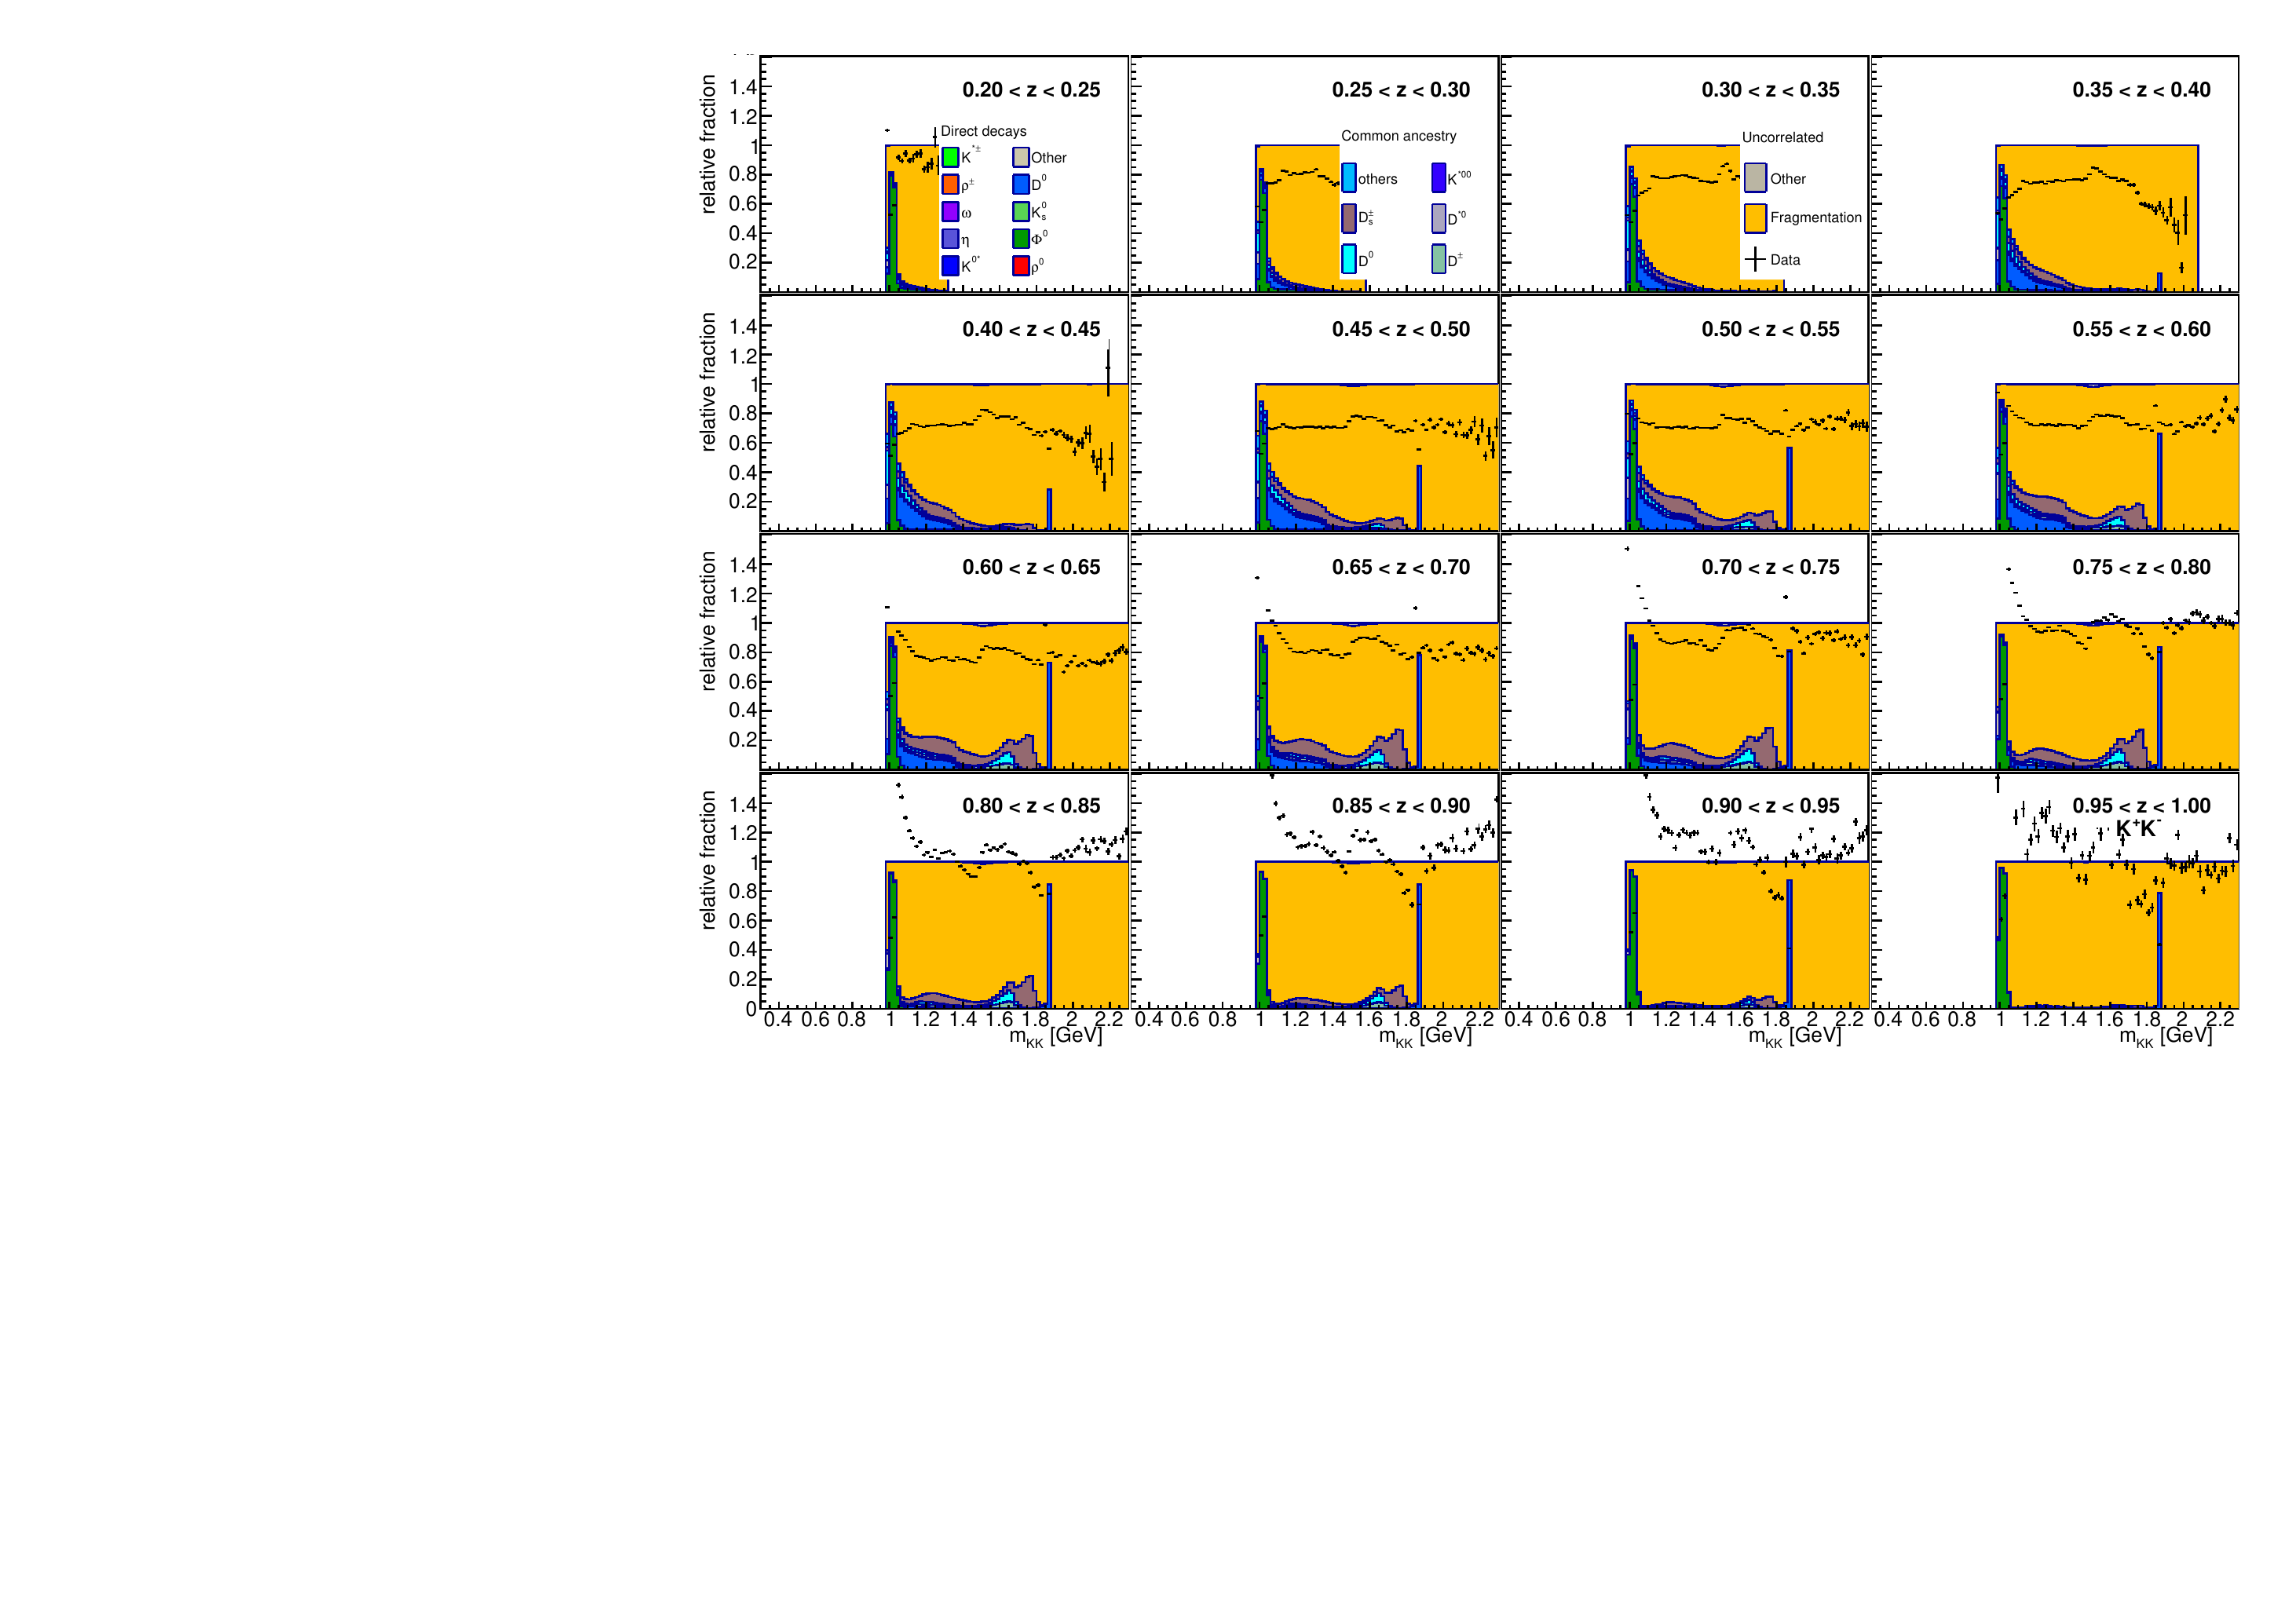}

\caption{\label{fig:results:massdists12} MC decomposition of the opposite-sign kaon pairs as a function of $m_{KK}$ in bins of $z$ for various resonance, partial resonant and non-resonant parents, displayed in linear scale (top) and as a relative fraction of the total cross section (bottom).}
\end{center}
\end{figure*}
\begin{figure*}[htb]
\begin{center}
\includegraphics[width=0.9\textwidth]{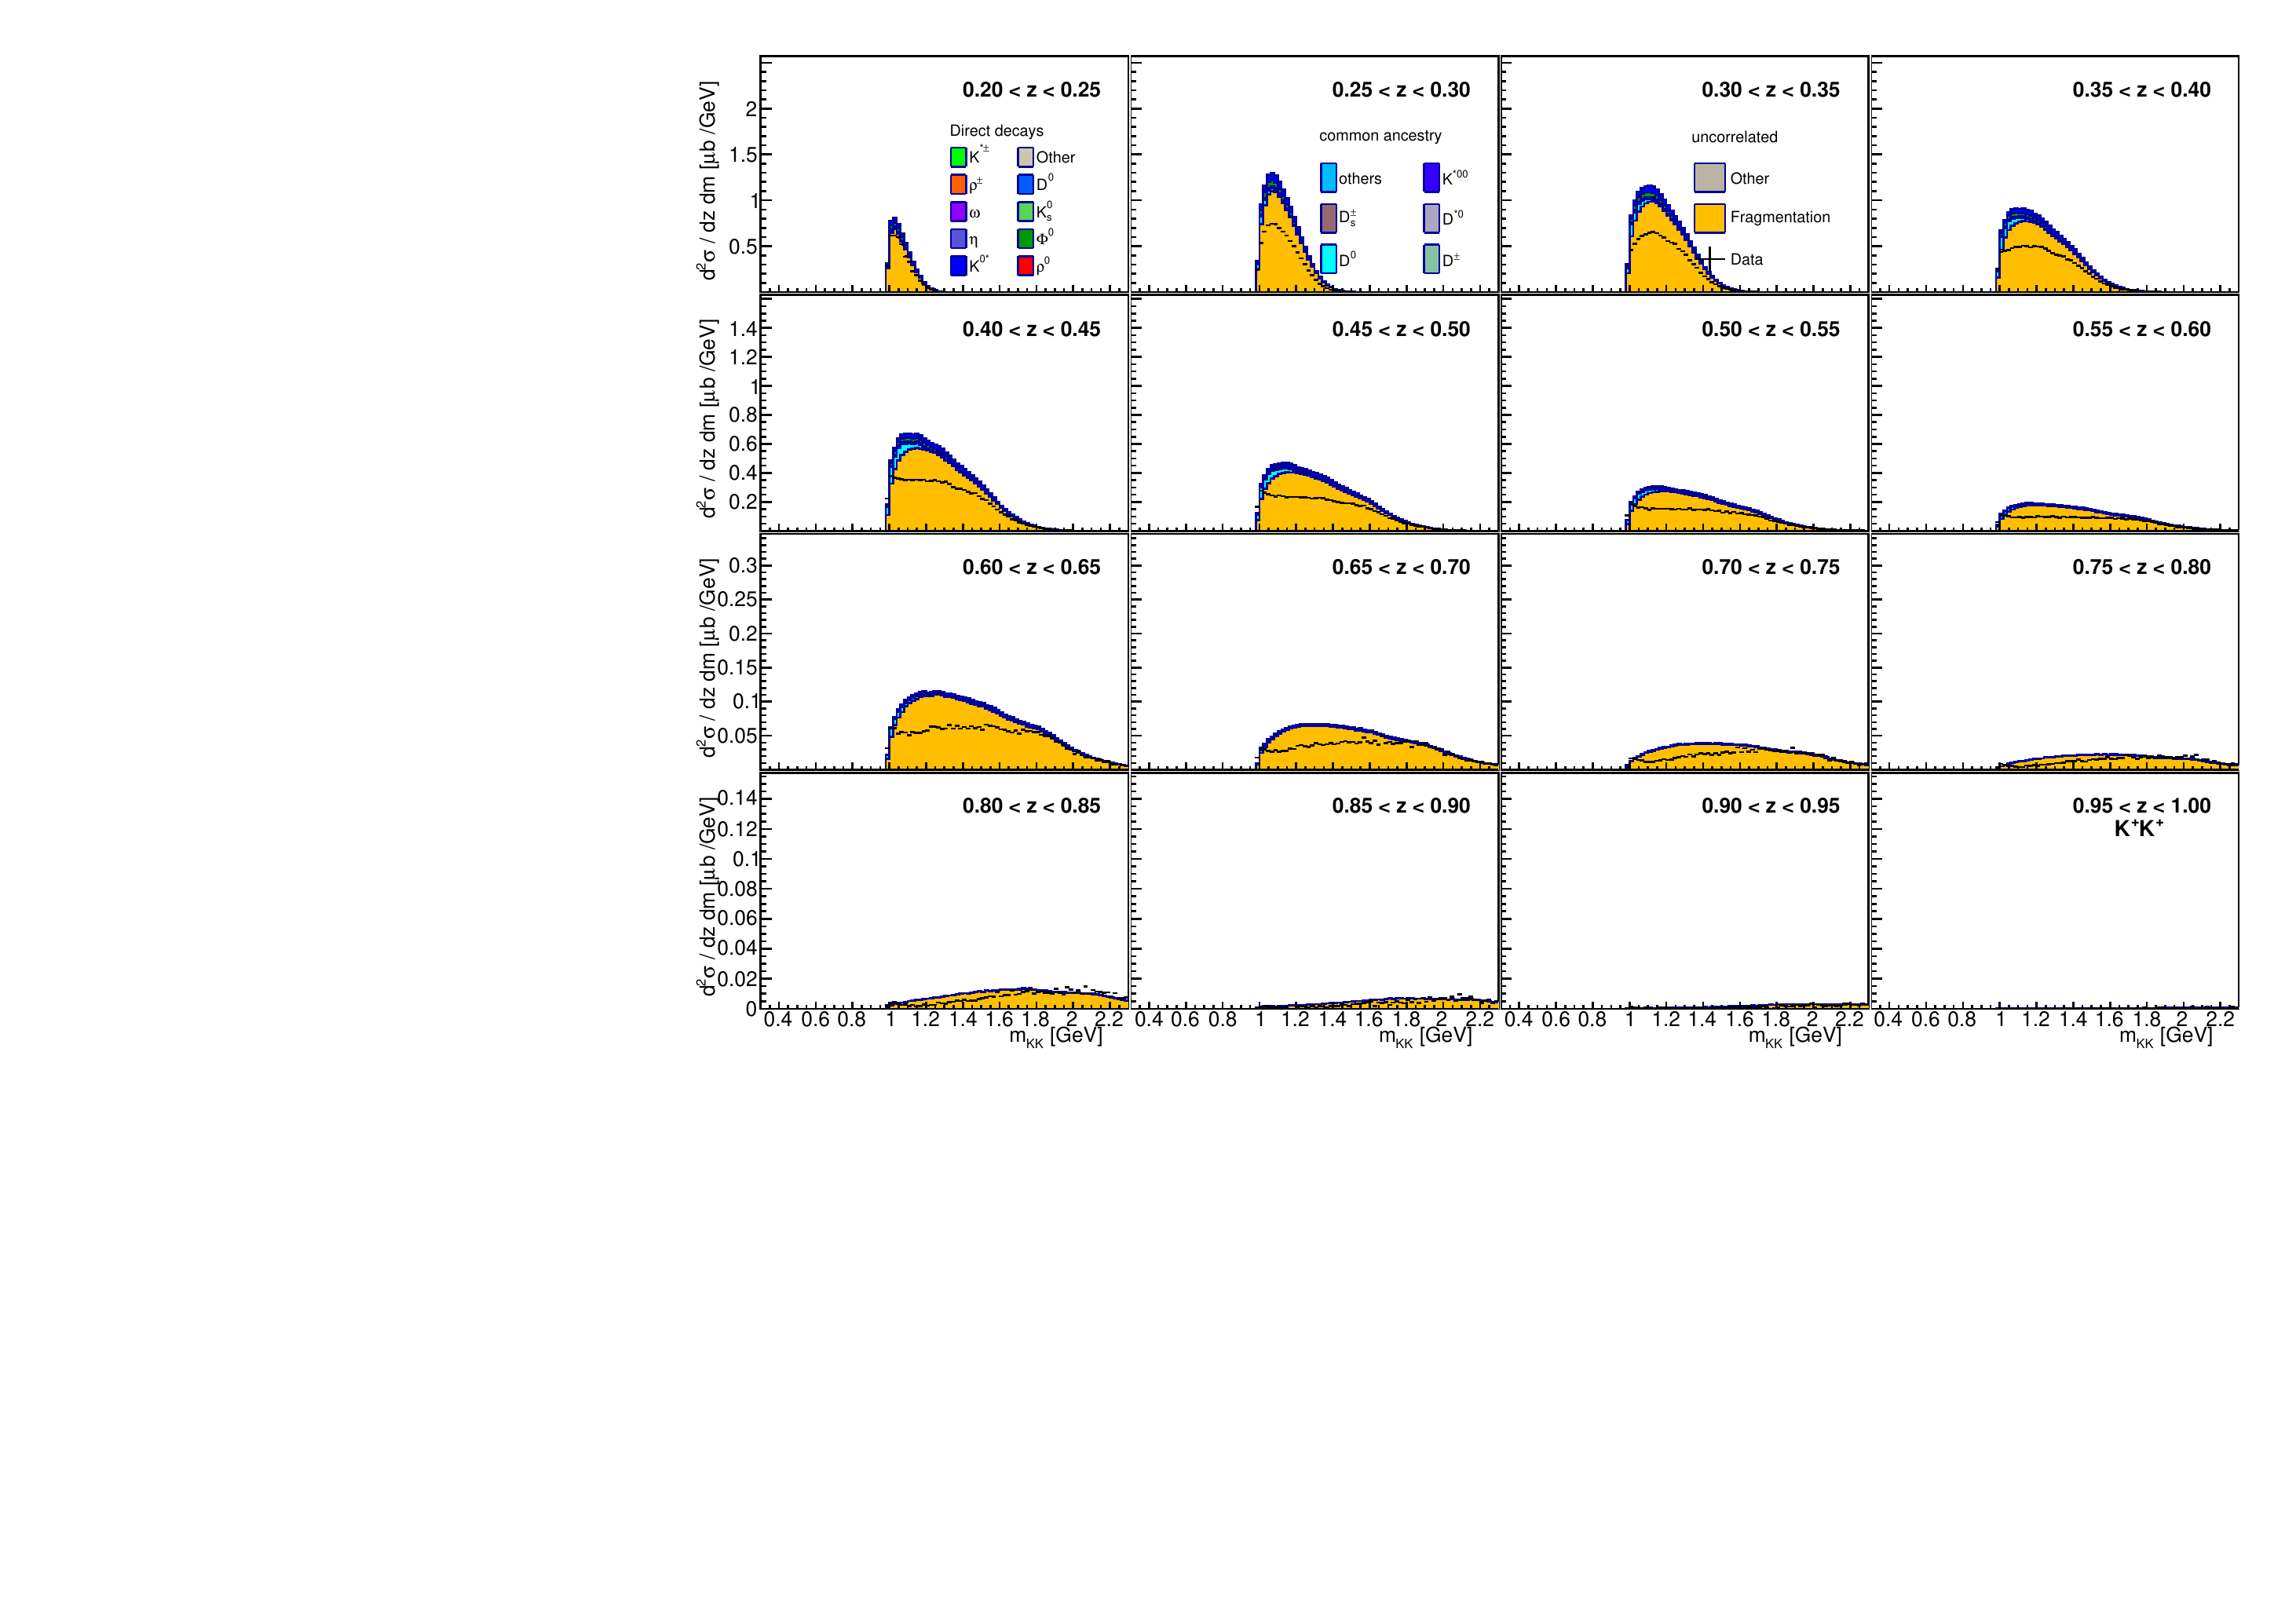}
\includegraphics[width=0.9\textwidth]{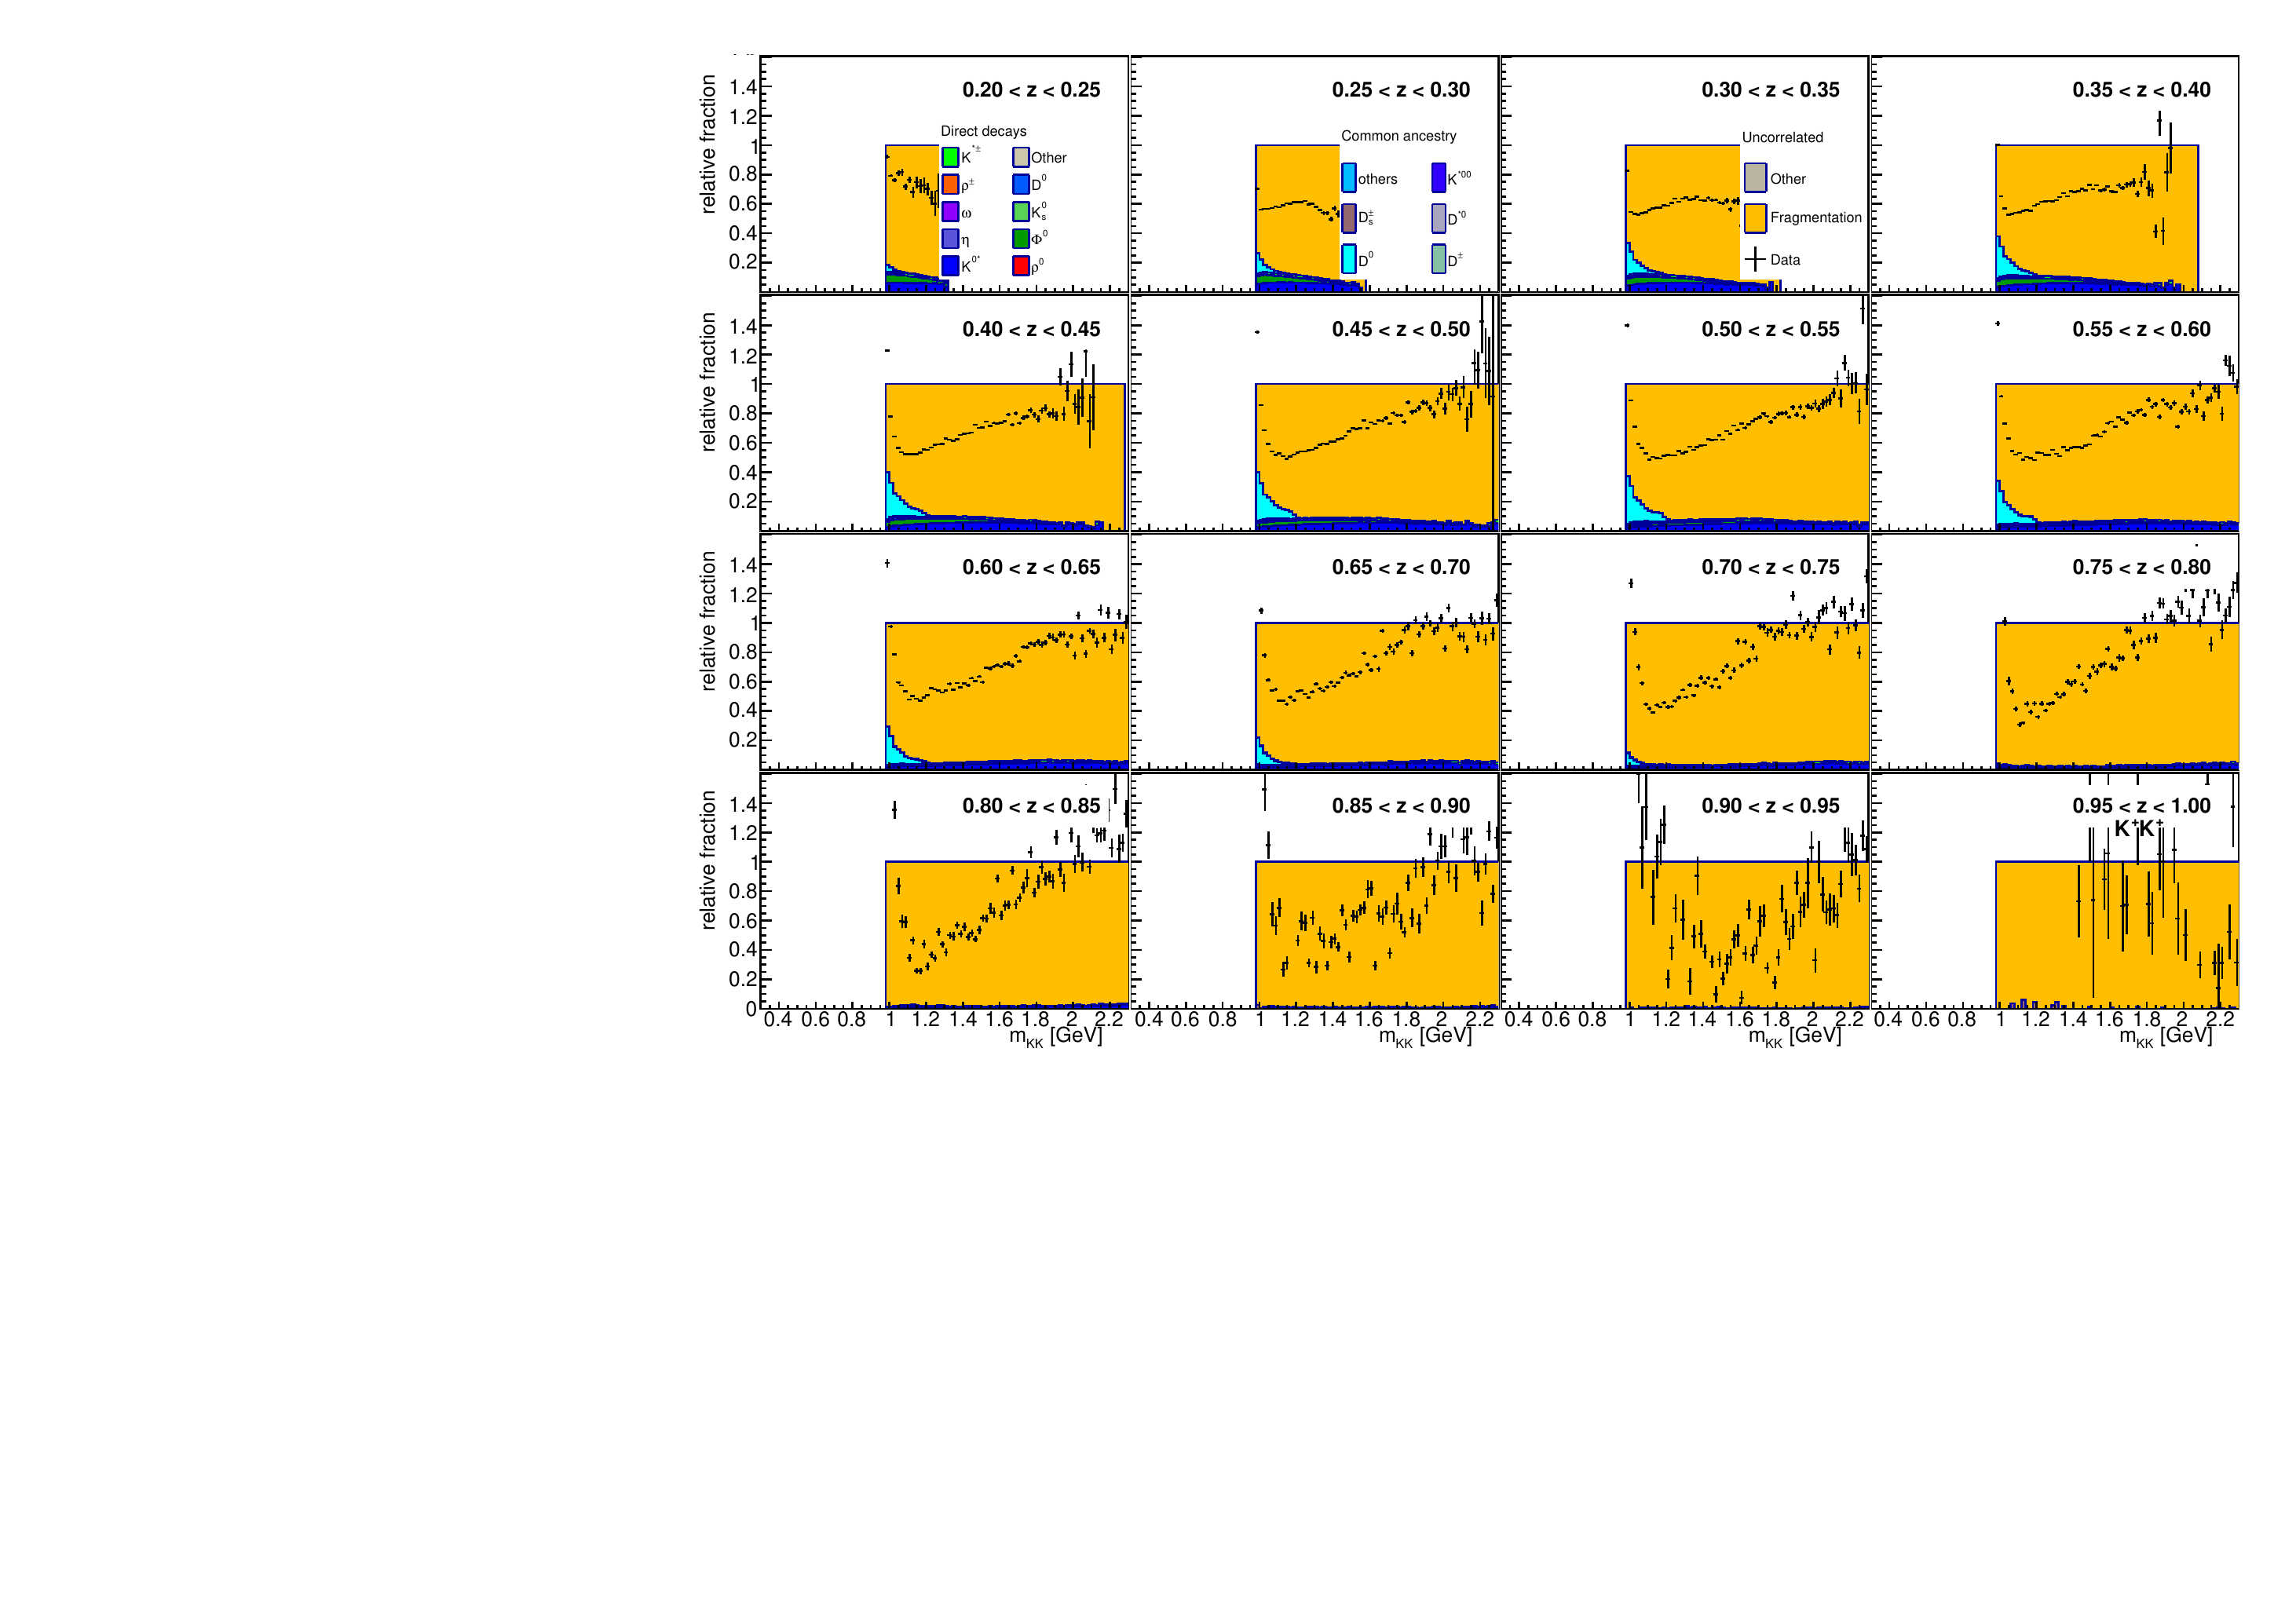}

\caption{\label{fig:results:massdists13} MC decomposition of the like-sign kaon pairs as a function of $m_{KK}$ in bins of $z$ for various resonance, partial resonant and non-resonant parents, displayed in linear scale (top) and as a relative fraction of the total cross section (bottom).}
\end{center}
\end{figure*}

\clearpage

\subsection{MC generator comparison}
Figures \ref{fig:allxsec_pid2_mix1_c8_32518153} to \ref{fig:allxsec_pid8192_mix1_c8_32518153} display the comparison of the di-hadron cross sections with various MC tunes.
\begin{figure*}[htb]
\begin{center}
\includegraphics[width=0.8\textwidth]{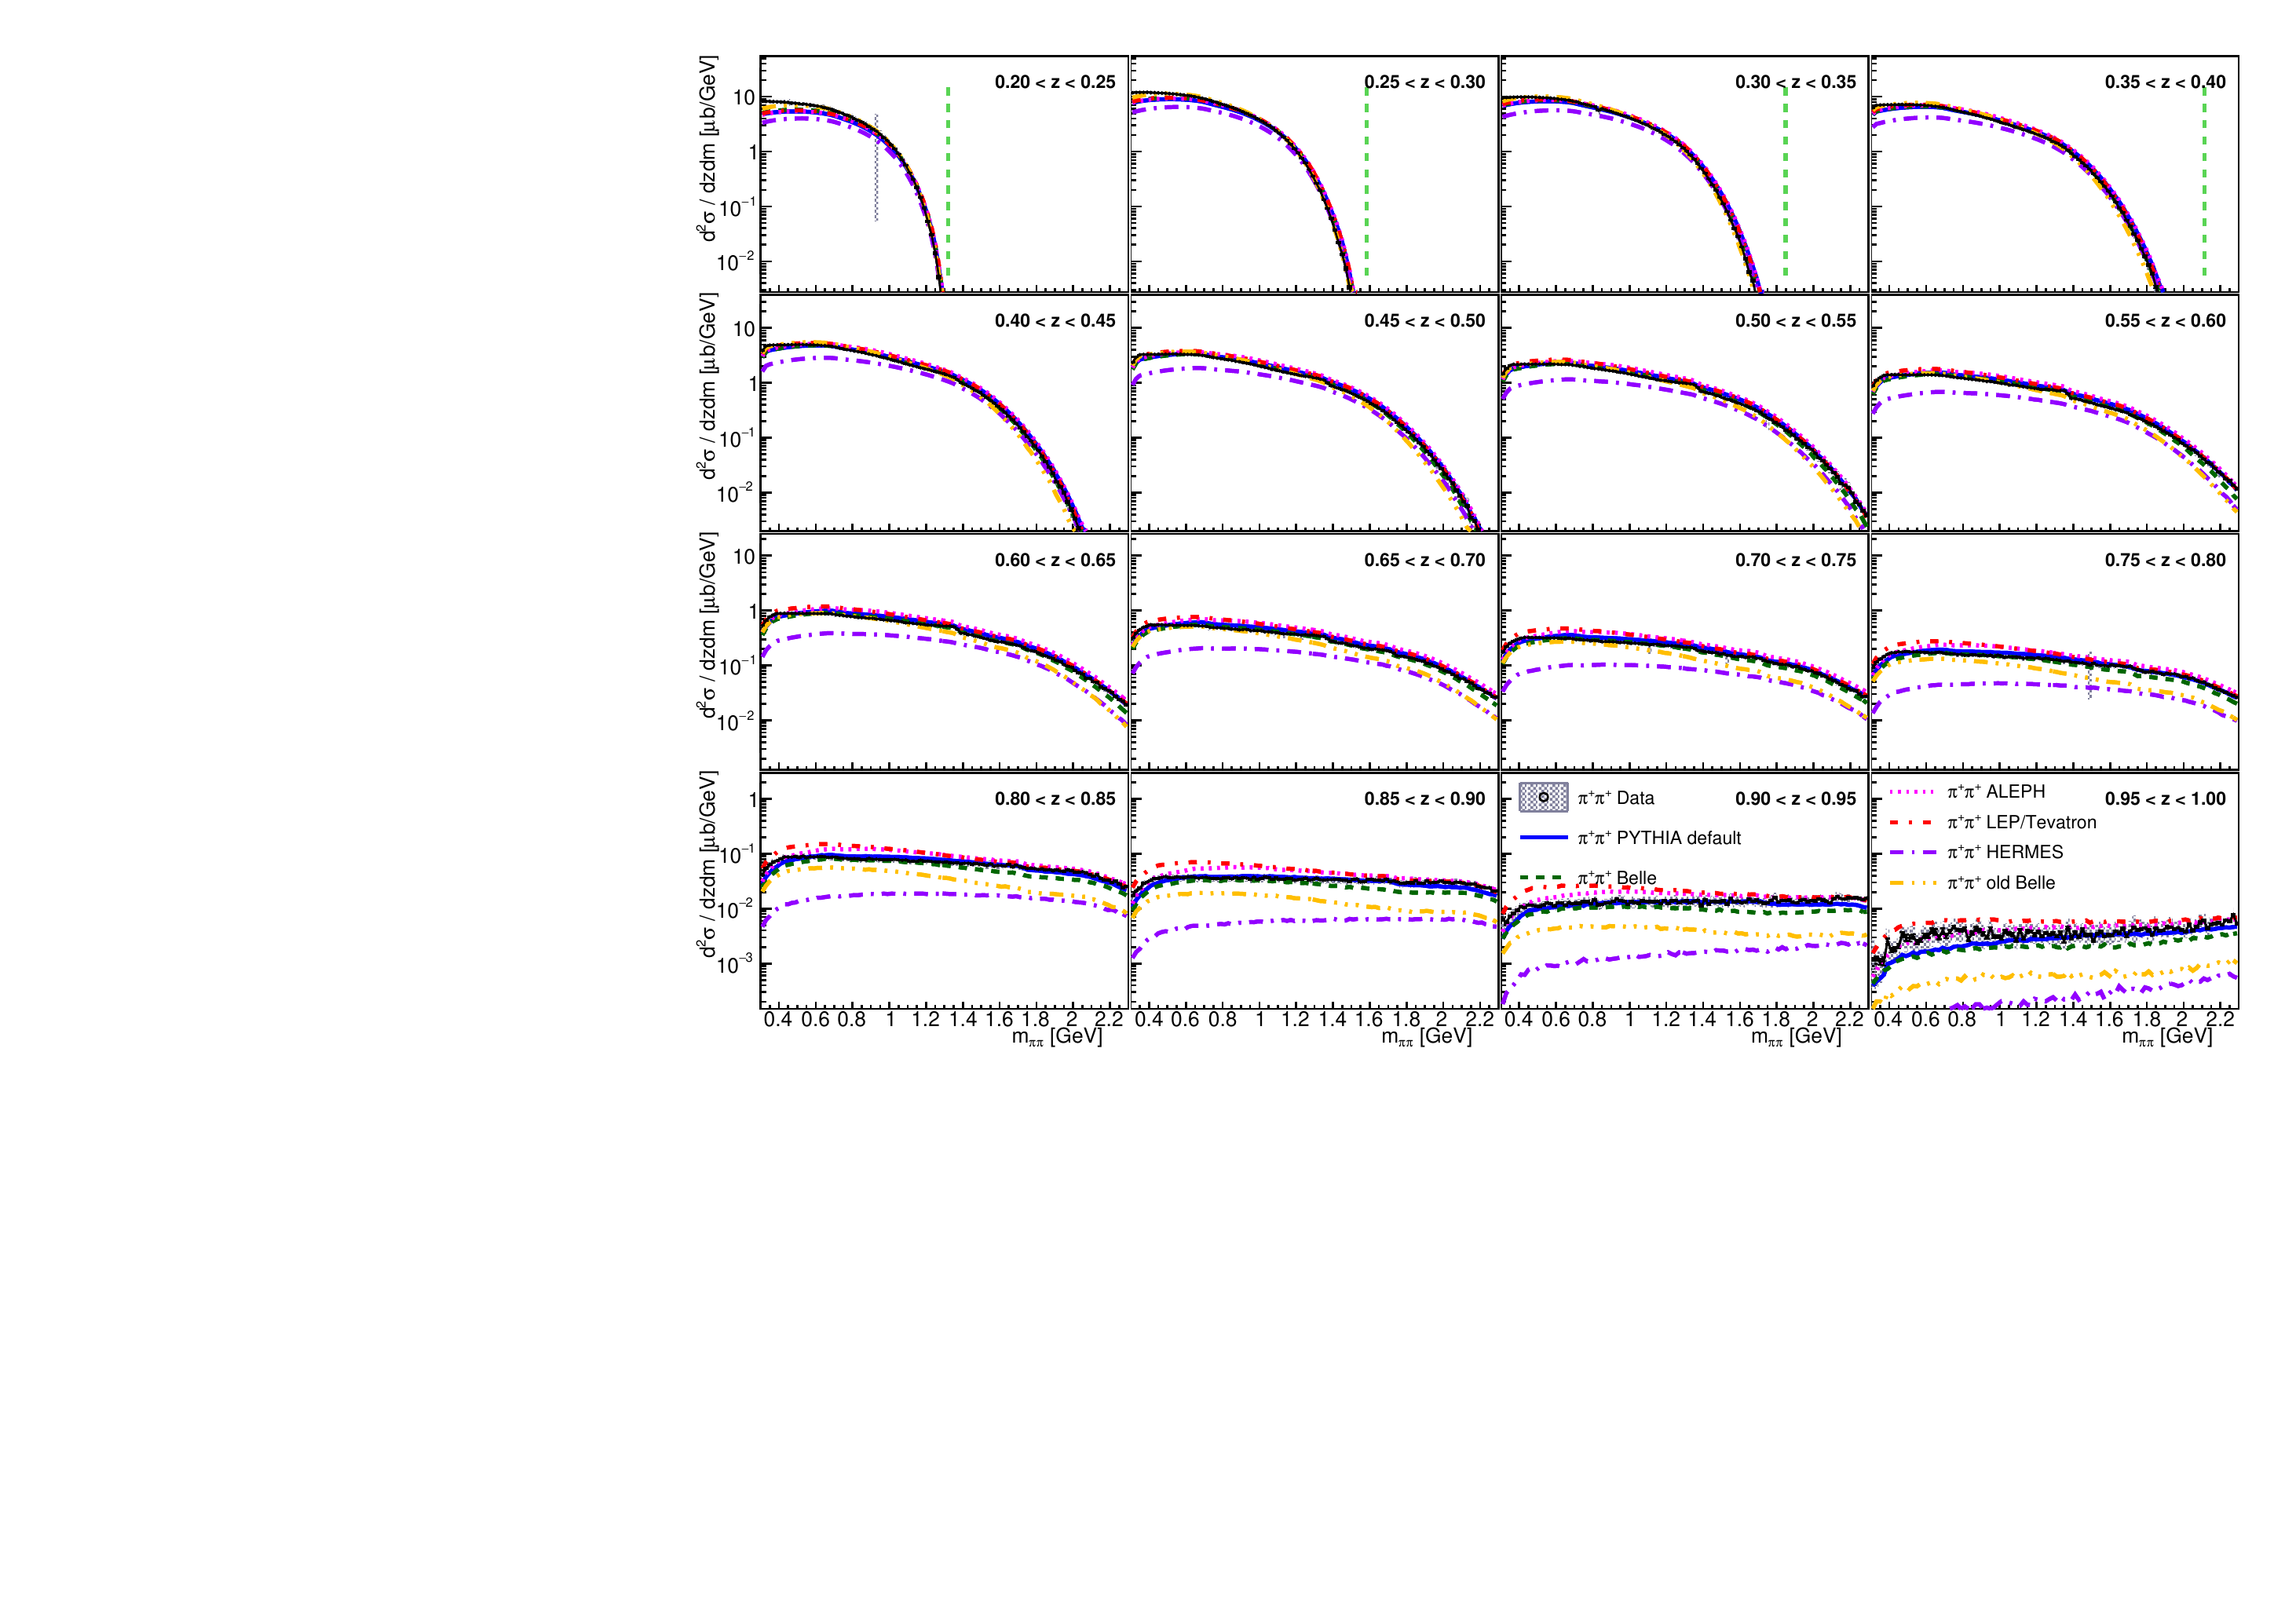}
\caption{\label{fig:allxsec_pid2_mix1_c8_32518153}Differential cross sections for $\pi^+\pi^++\ c.c.$ pairs as a function of $m_{\pi\pi}$ in bins of $z$. Various {\sc Pythia} tunes are also displayed as described in the paper text. The vertical green dashed line corresponds to the kinematic limit. An overall 1.6\% scale uncertainty is not shown.}
\end{center}
\end{figure*}

\begin{figure*}[htb]
\begin{center}
\includegraphics[width=0.8\textwidth]{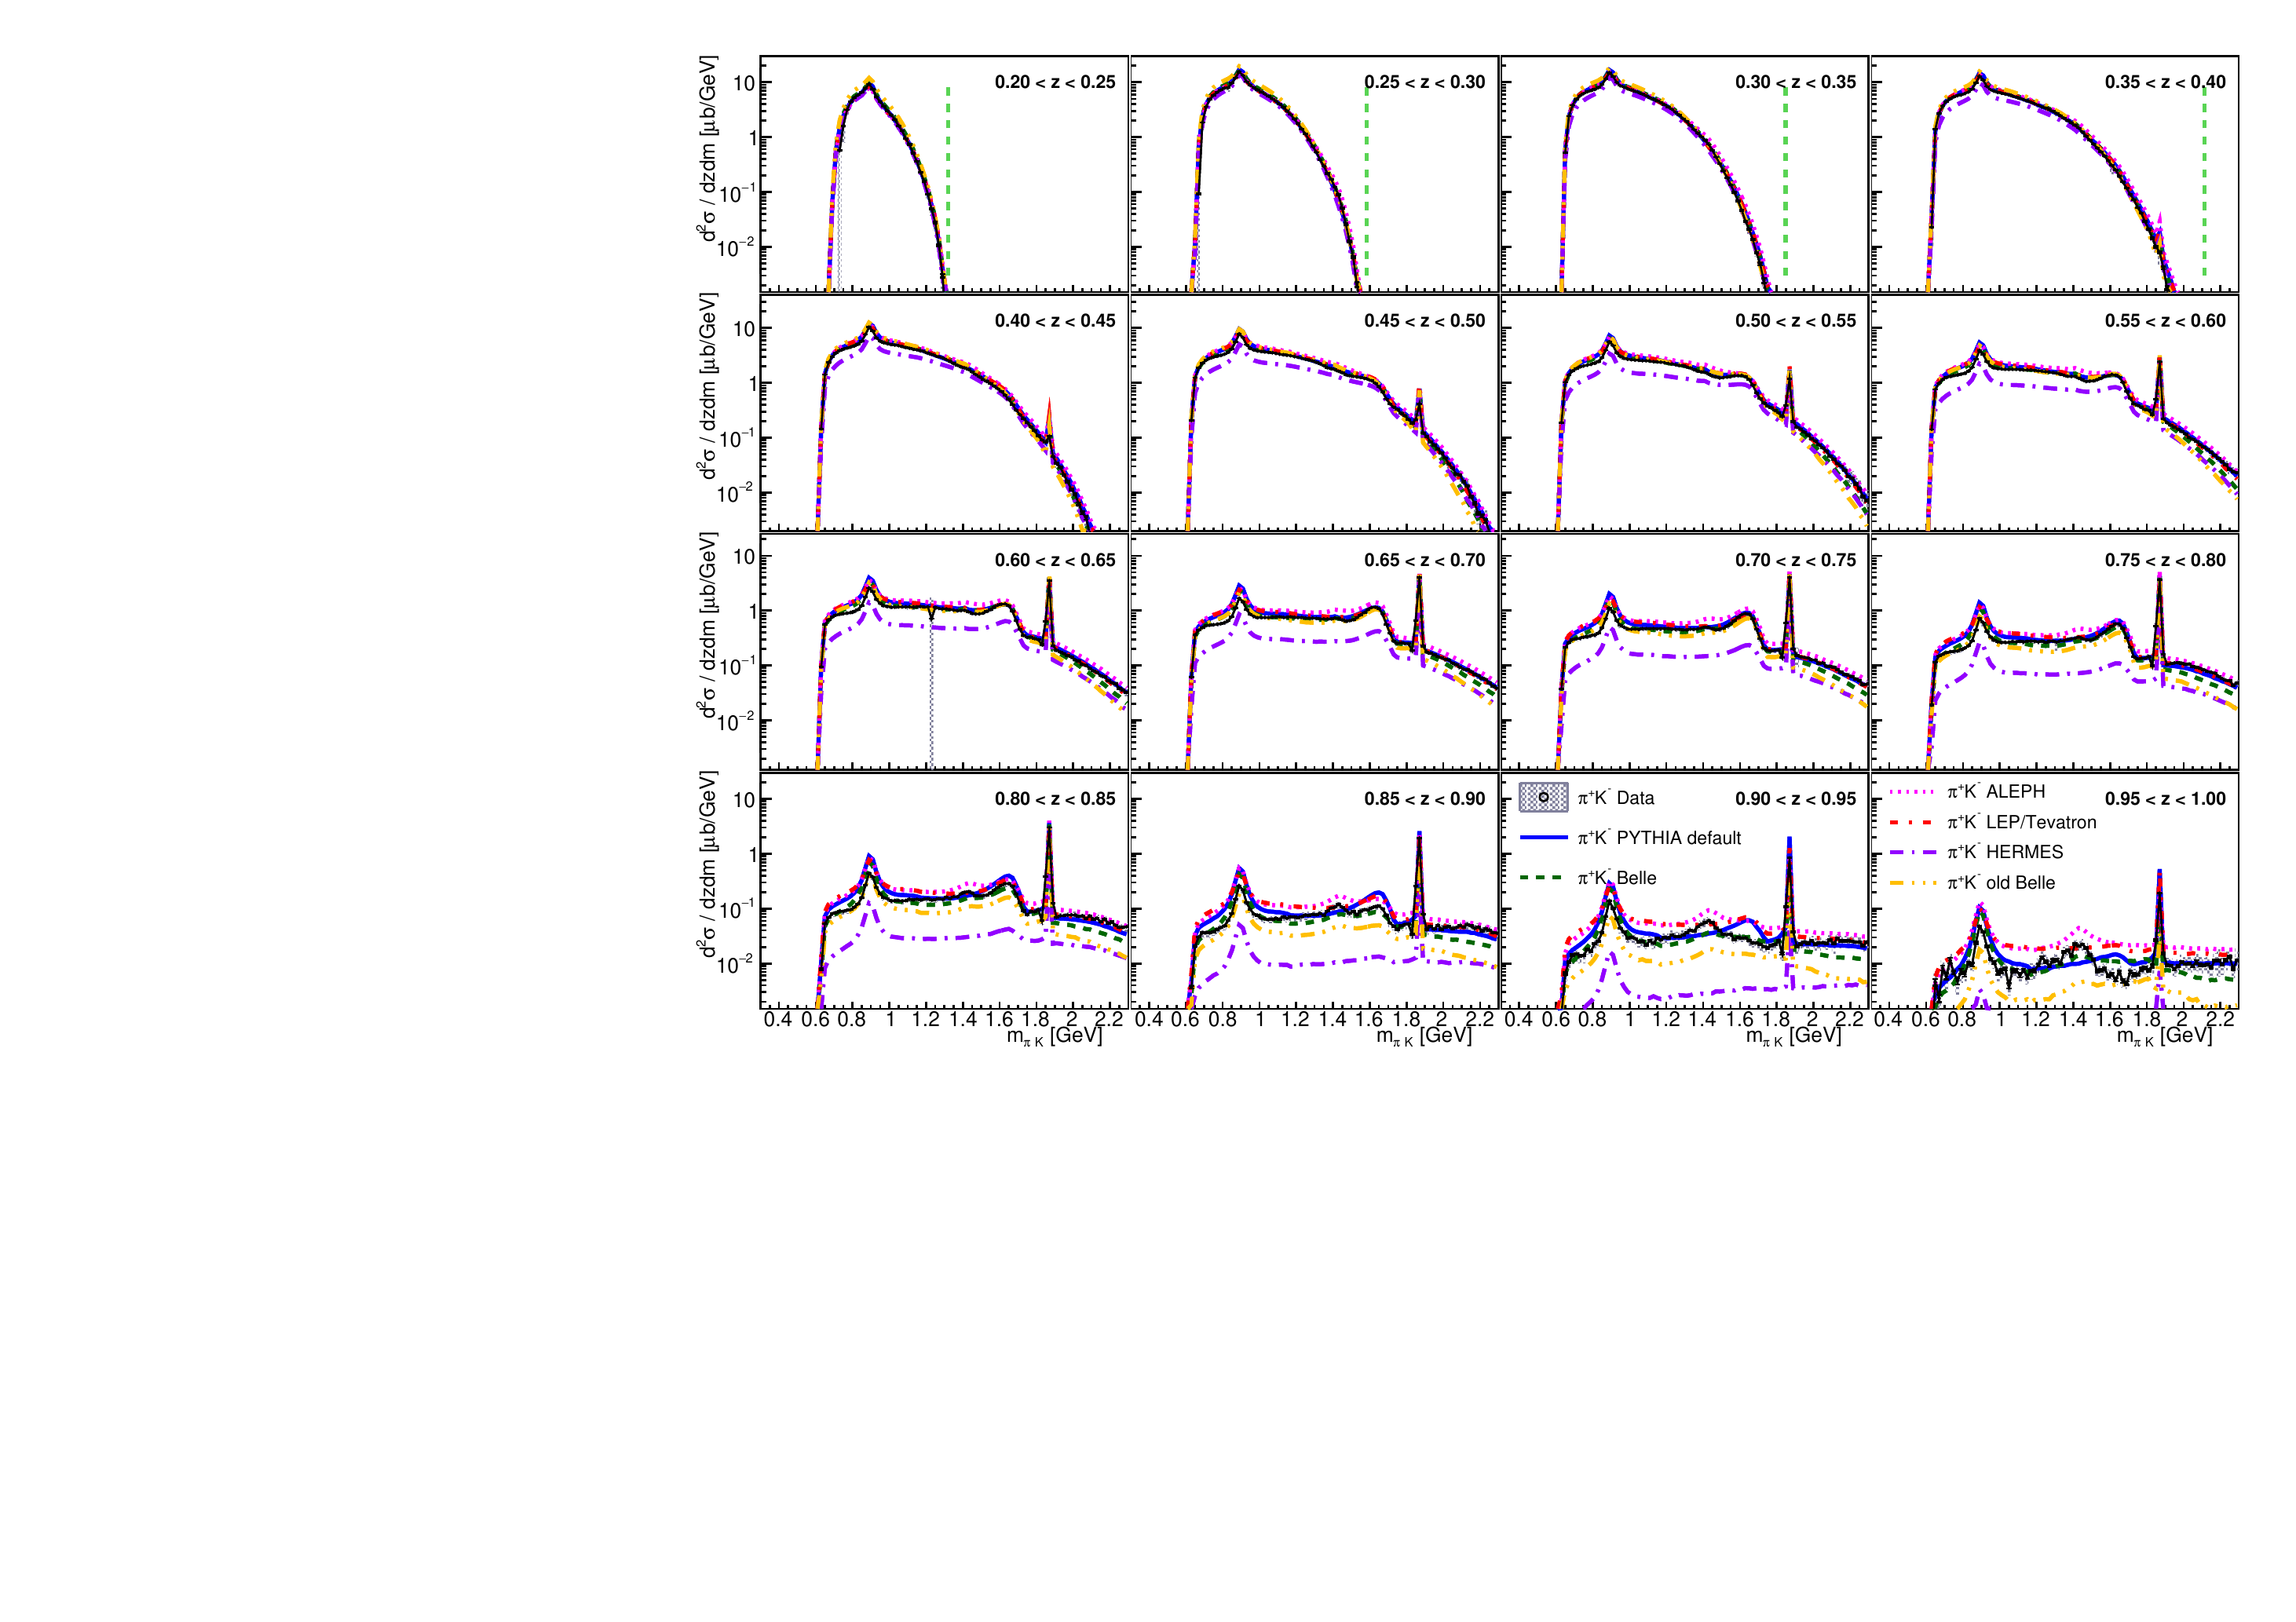}
\caption{\label{fig:allxsec_pid16_mix1_c8_32518153}Differential cross sections for $K^+\pi^-+\ c.c.$ pairs as a function of $m_{K\pi}$ in bins of $z$. Various {\sc Pythia} tunes are also displayed as described in the paper text. The vertical green dashed line corresponds to the kinematic limit. An overall 1.6\% scale uncertainty is not shown.}
\end{center}
\end{figure*}
\begin{figure*}[htb]
\begin{center}
\includegraphics[width=0.8\textwidth]{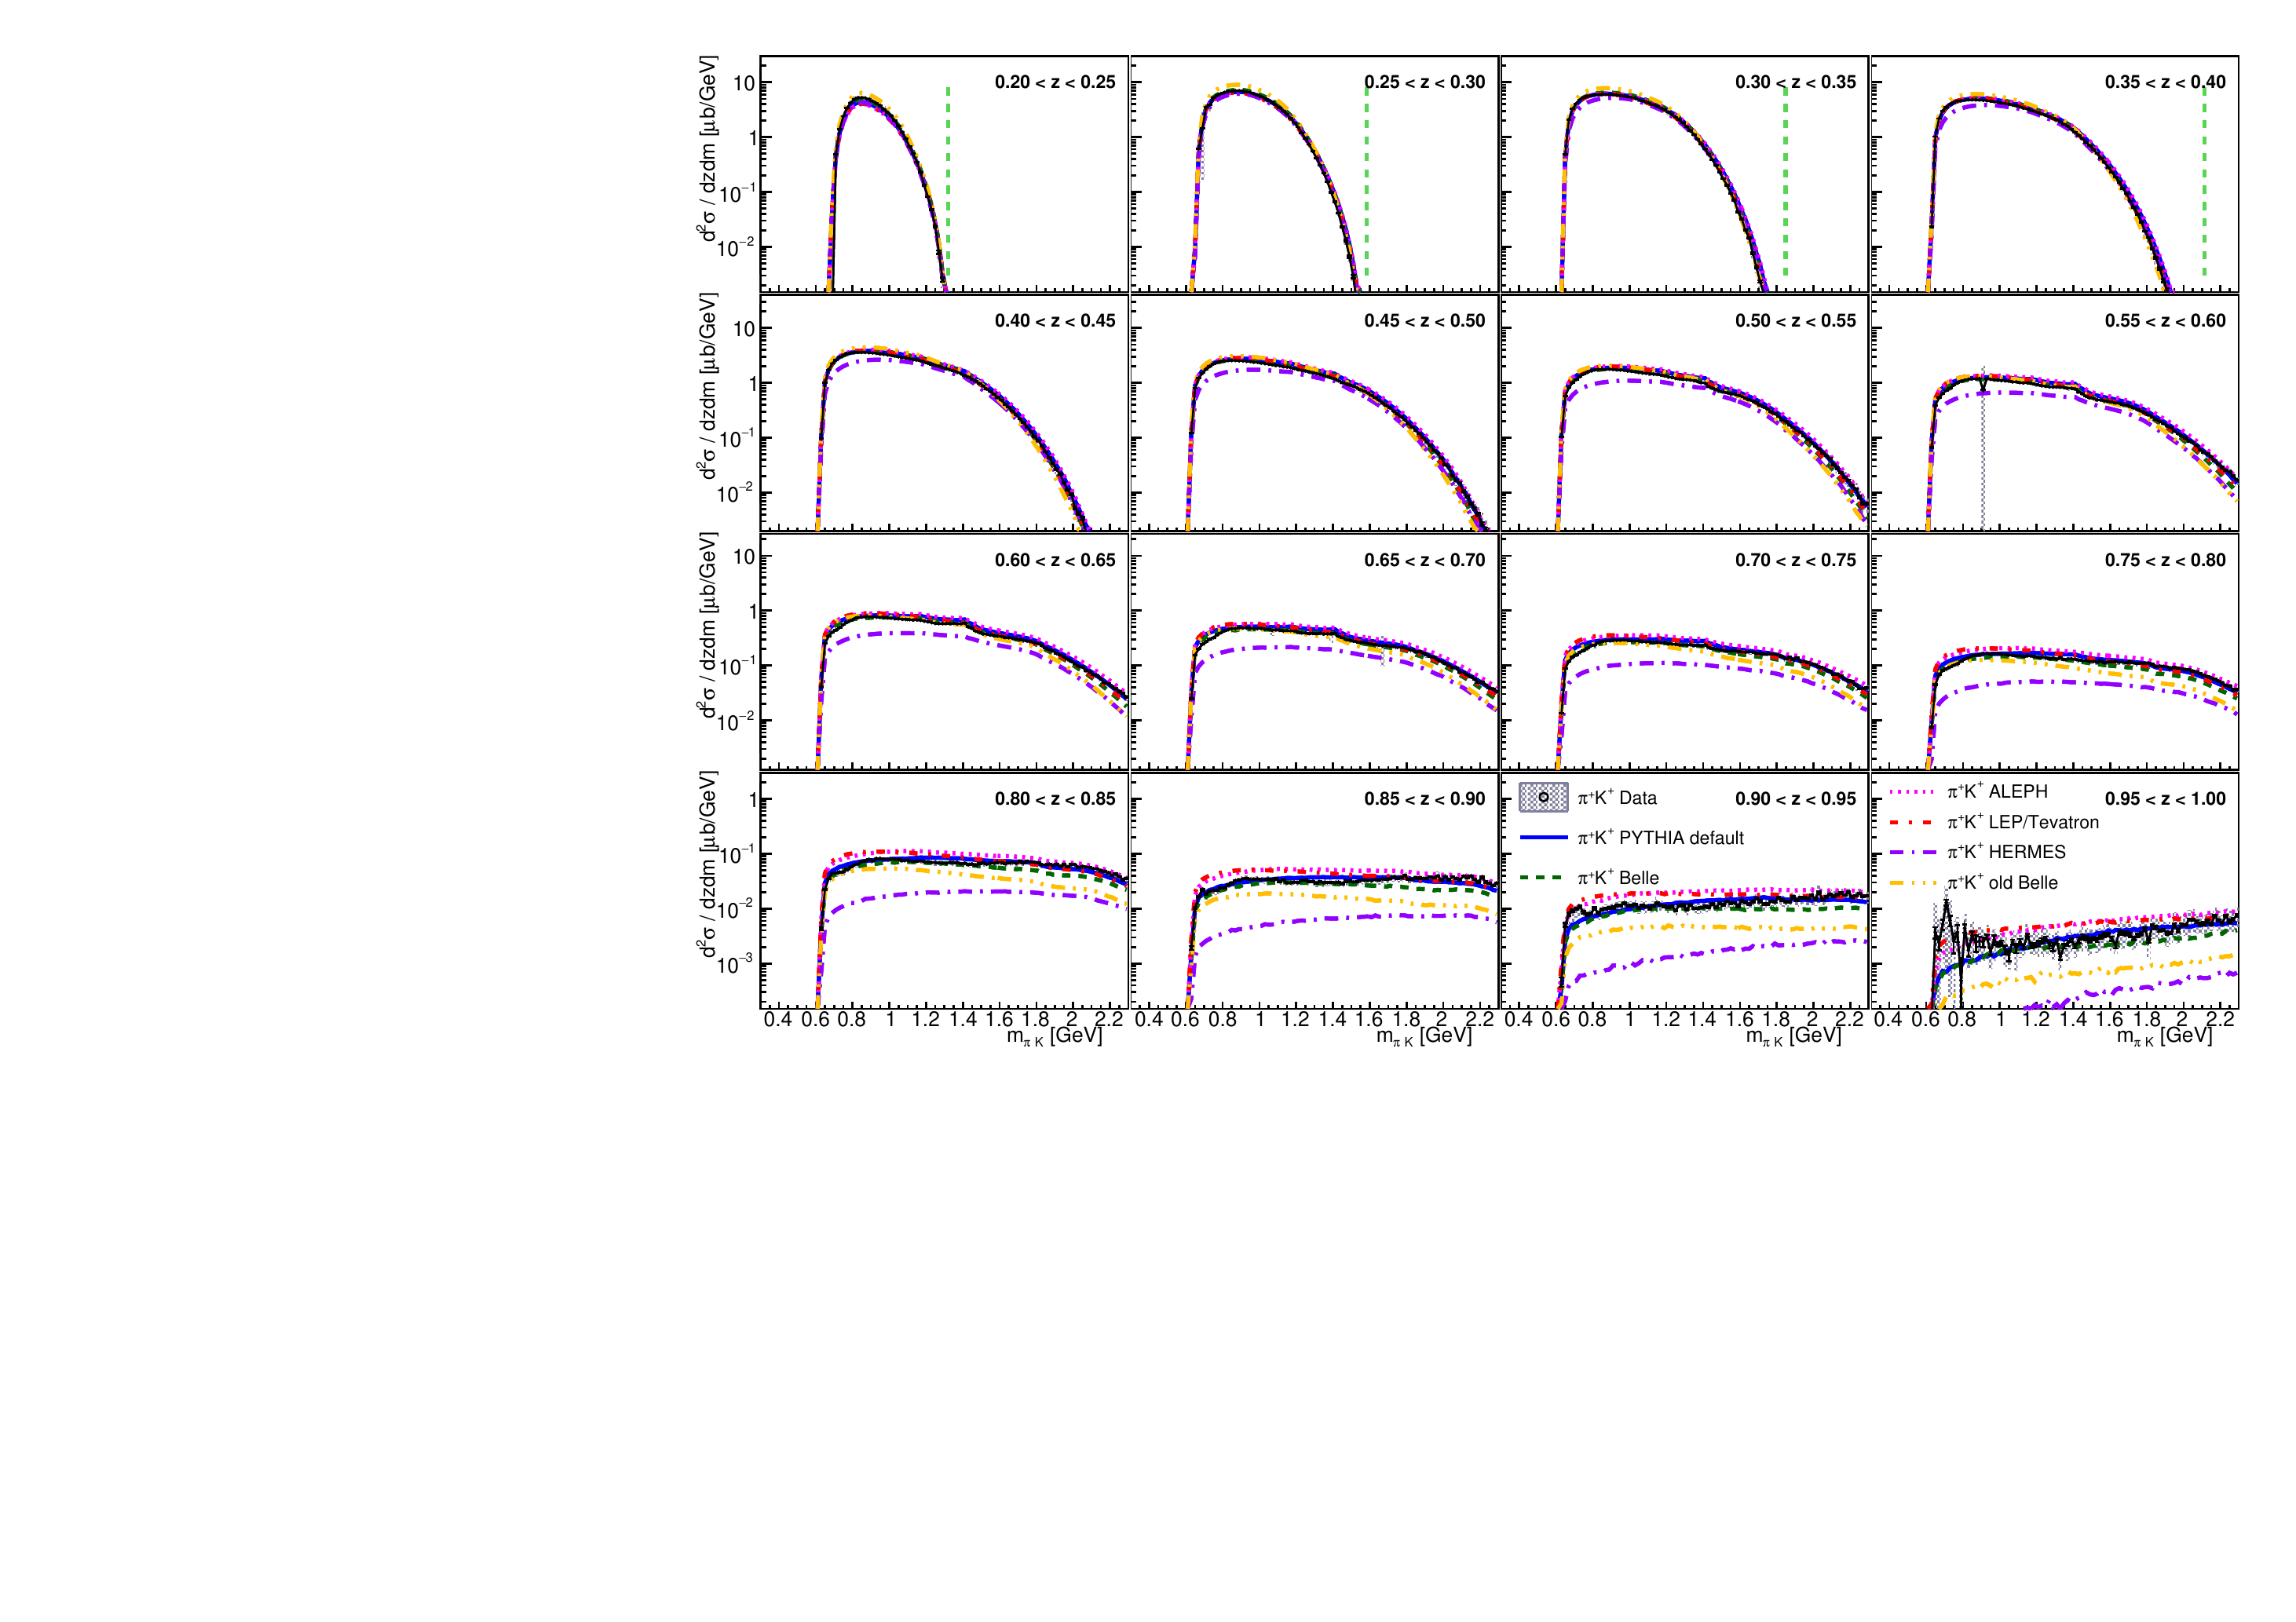}
\caption{\label{fig:allxsec_pid32_mix1_c8_32518153}Differential cross sections for $K^+\pi^++\ c.c.$ pairs as a function of $m_{K\pi}$ in bins of $z$. Various {\sc Pythia} tunes are also displayed as described in the paper text. The vertical green dashed line corresponds to the kinematic limit. An overall 1.6\% scale uncertainty is not shown.}
\end{center}
\end{figure*}

\begin{figure*}[htb]
\begin{center}
\includegraphics[width=0.8\textwidth]{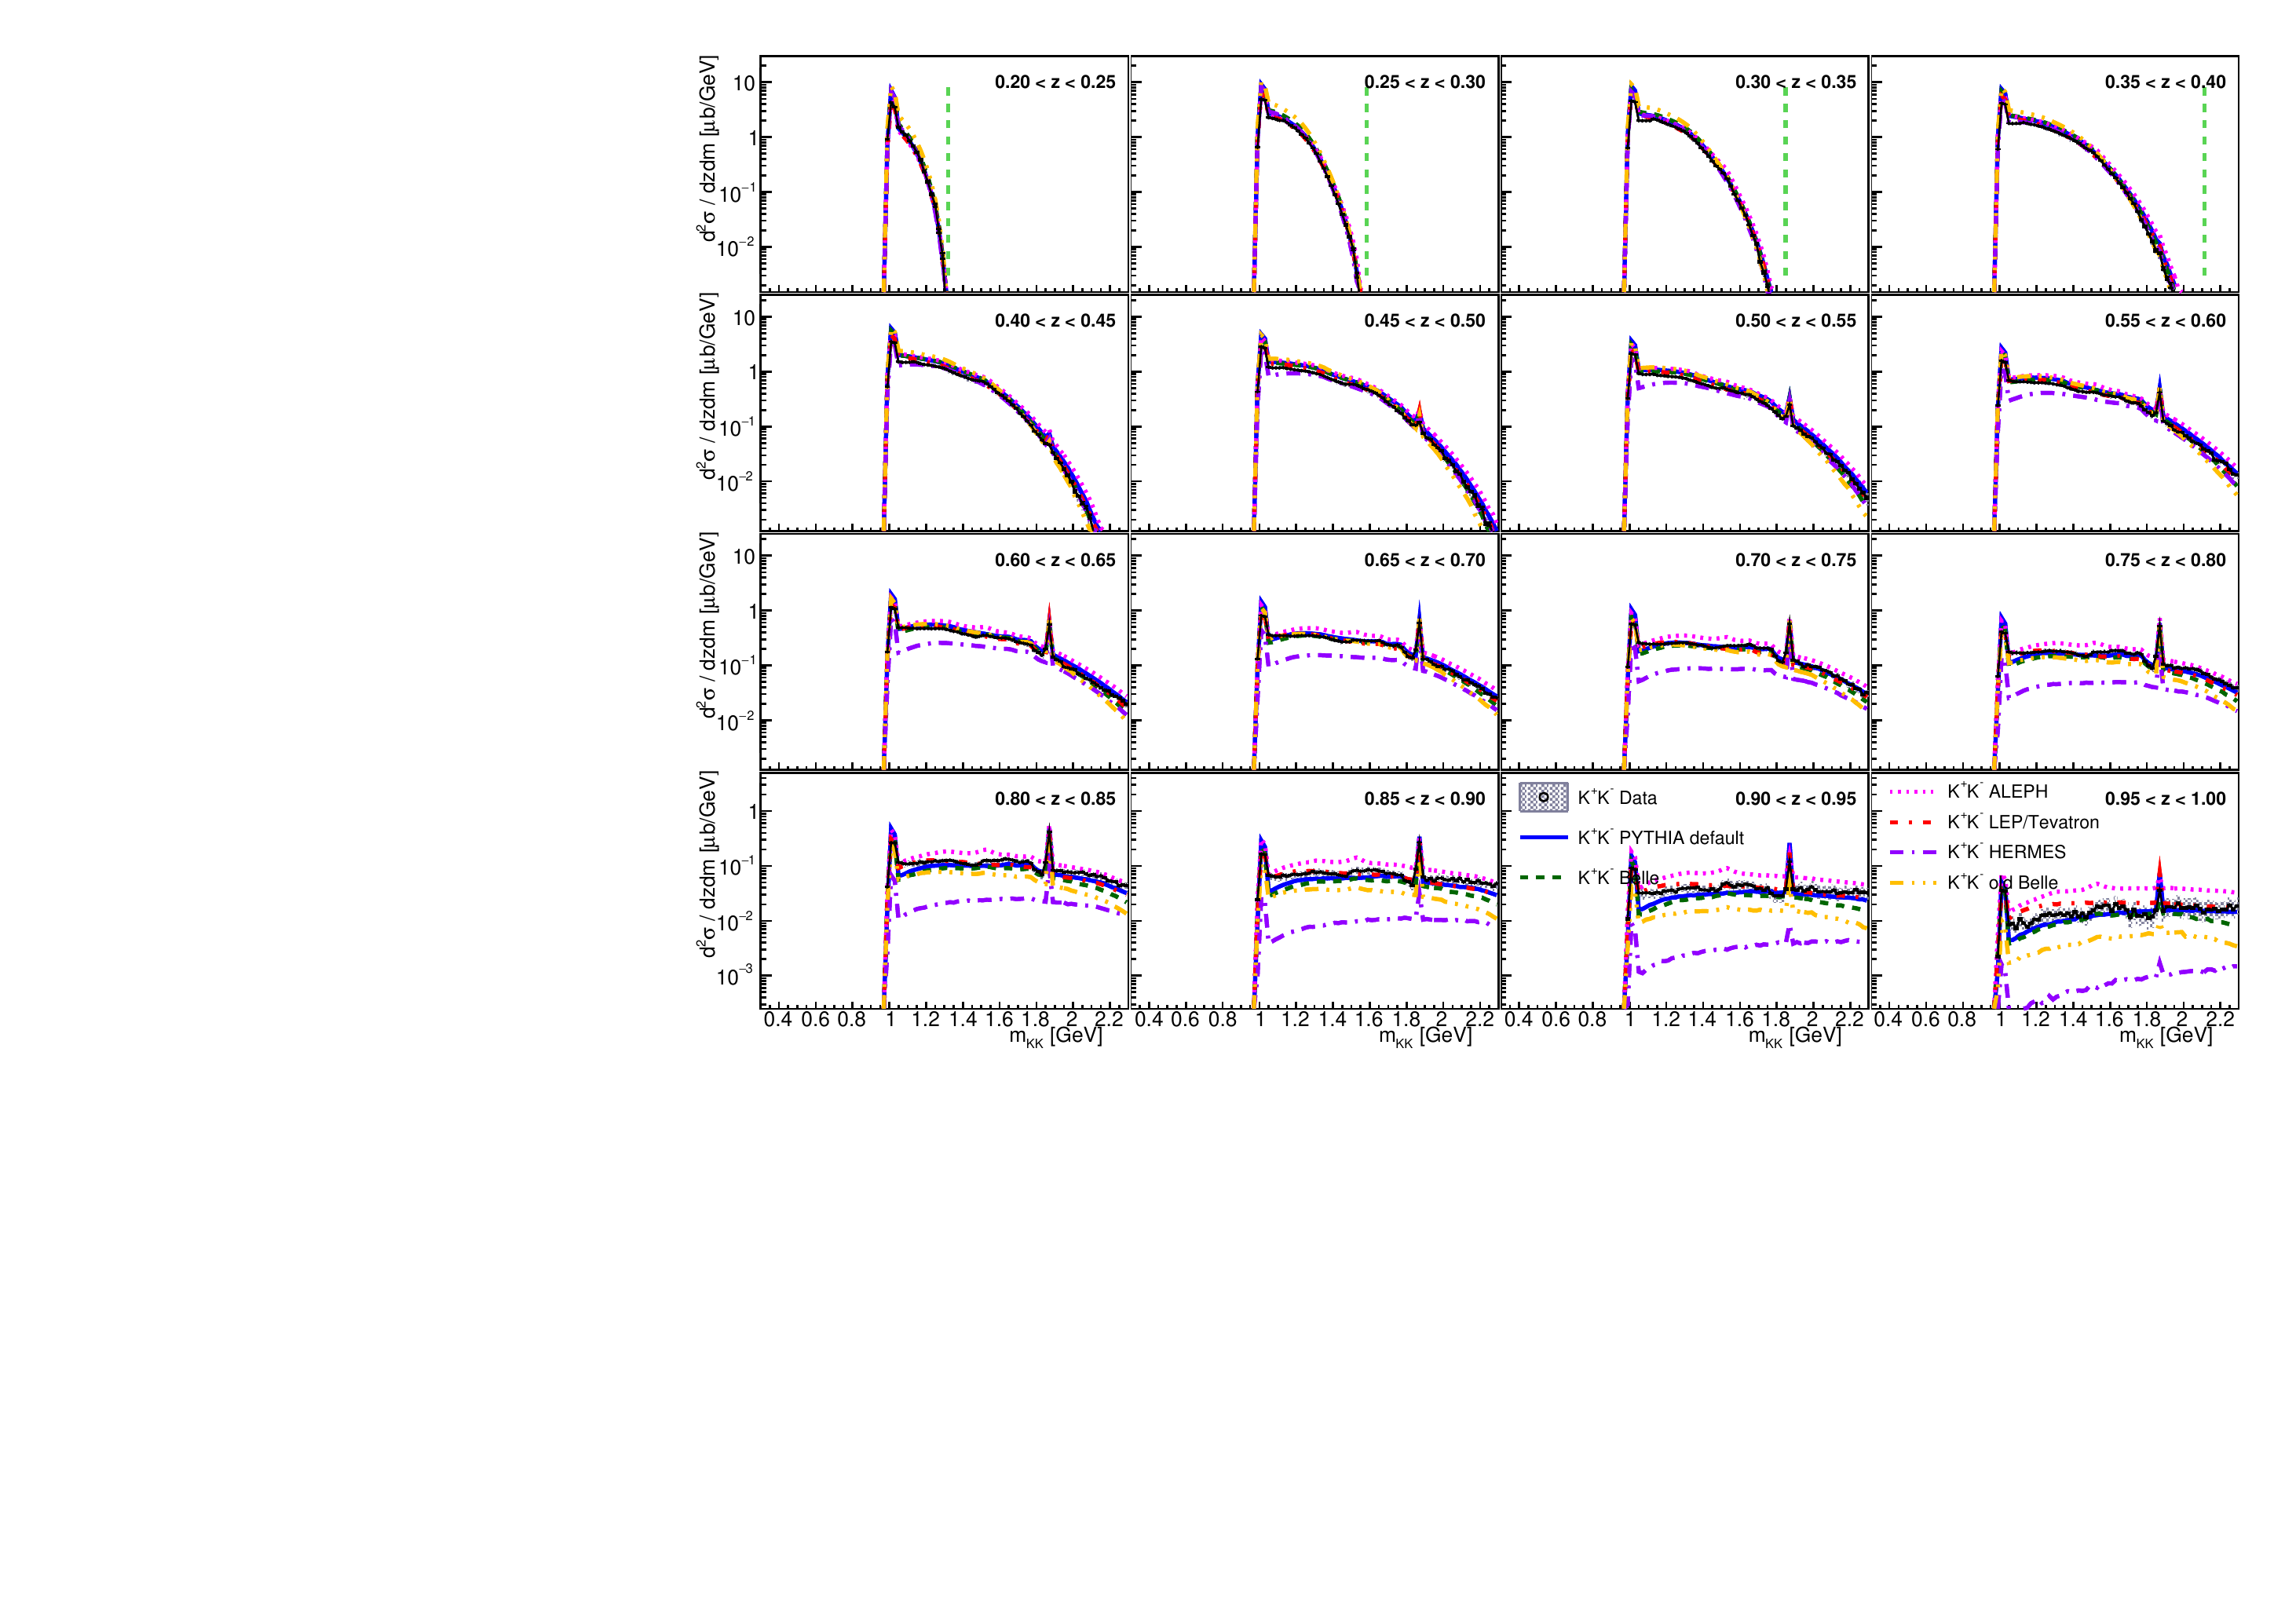}
\caption{\label{fig:allxsec_pid4096_mix1_c8_32518153}Differential cross sections for $K^+K^-$ pairs as a function of $m_{KK}$ in bins of $z$. Various {\sc Pythia} tunes are also displayed as described in the paper text. The vertical green dashed line corresponds to the kinematic limit. An overall 1.6\% scale uncertainty is not shown.}
\end{center}
\end{figure*}

\begin{figure*}[htb]
\begin{center}
\includegraphics[width=0.8\textwidth]{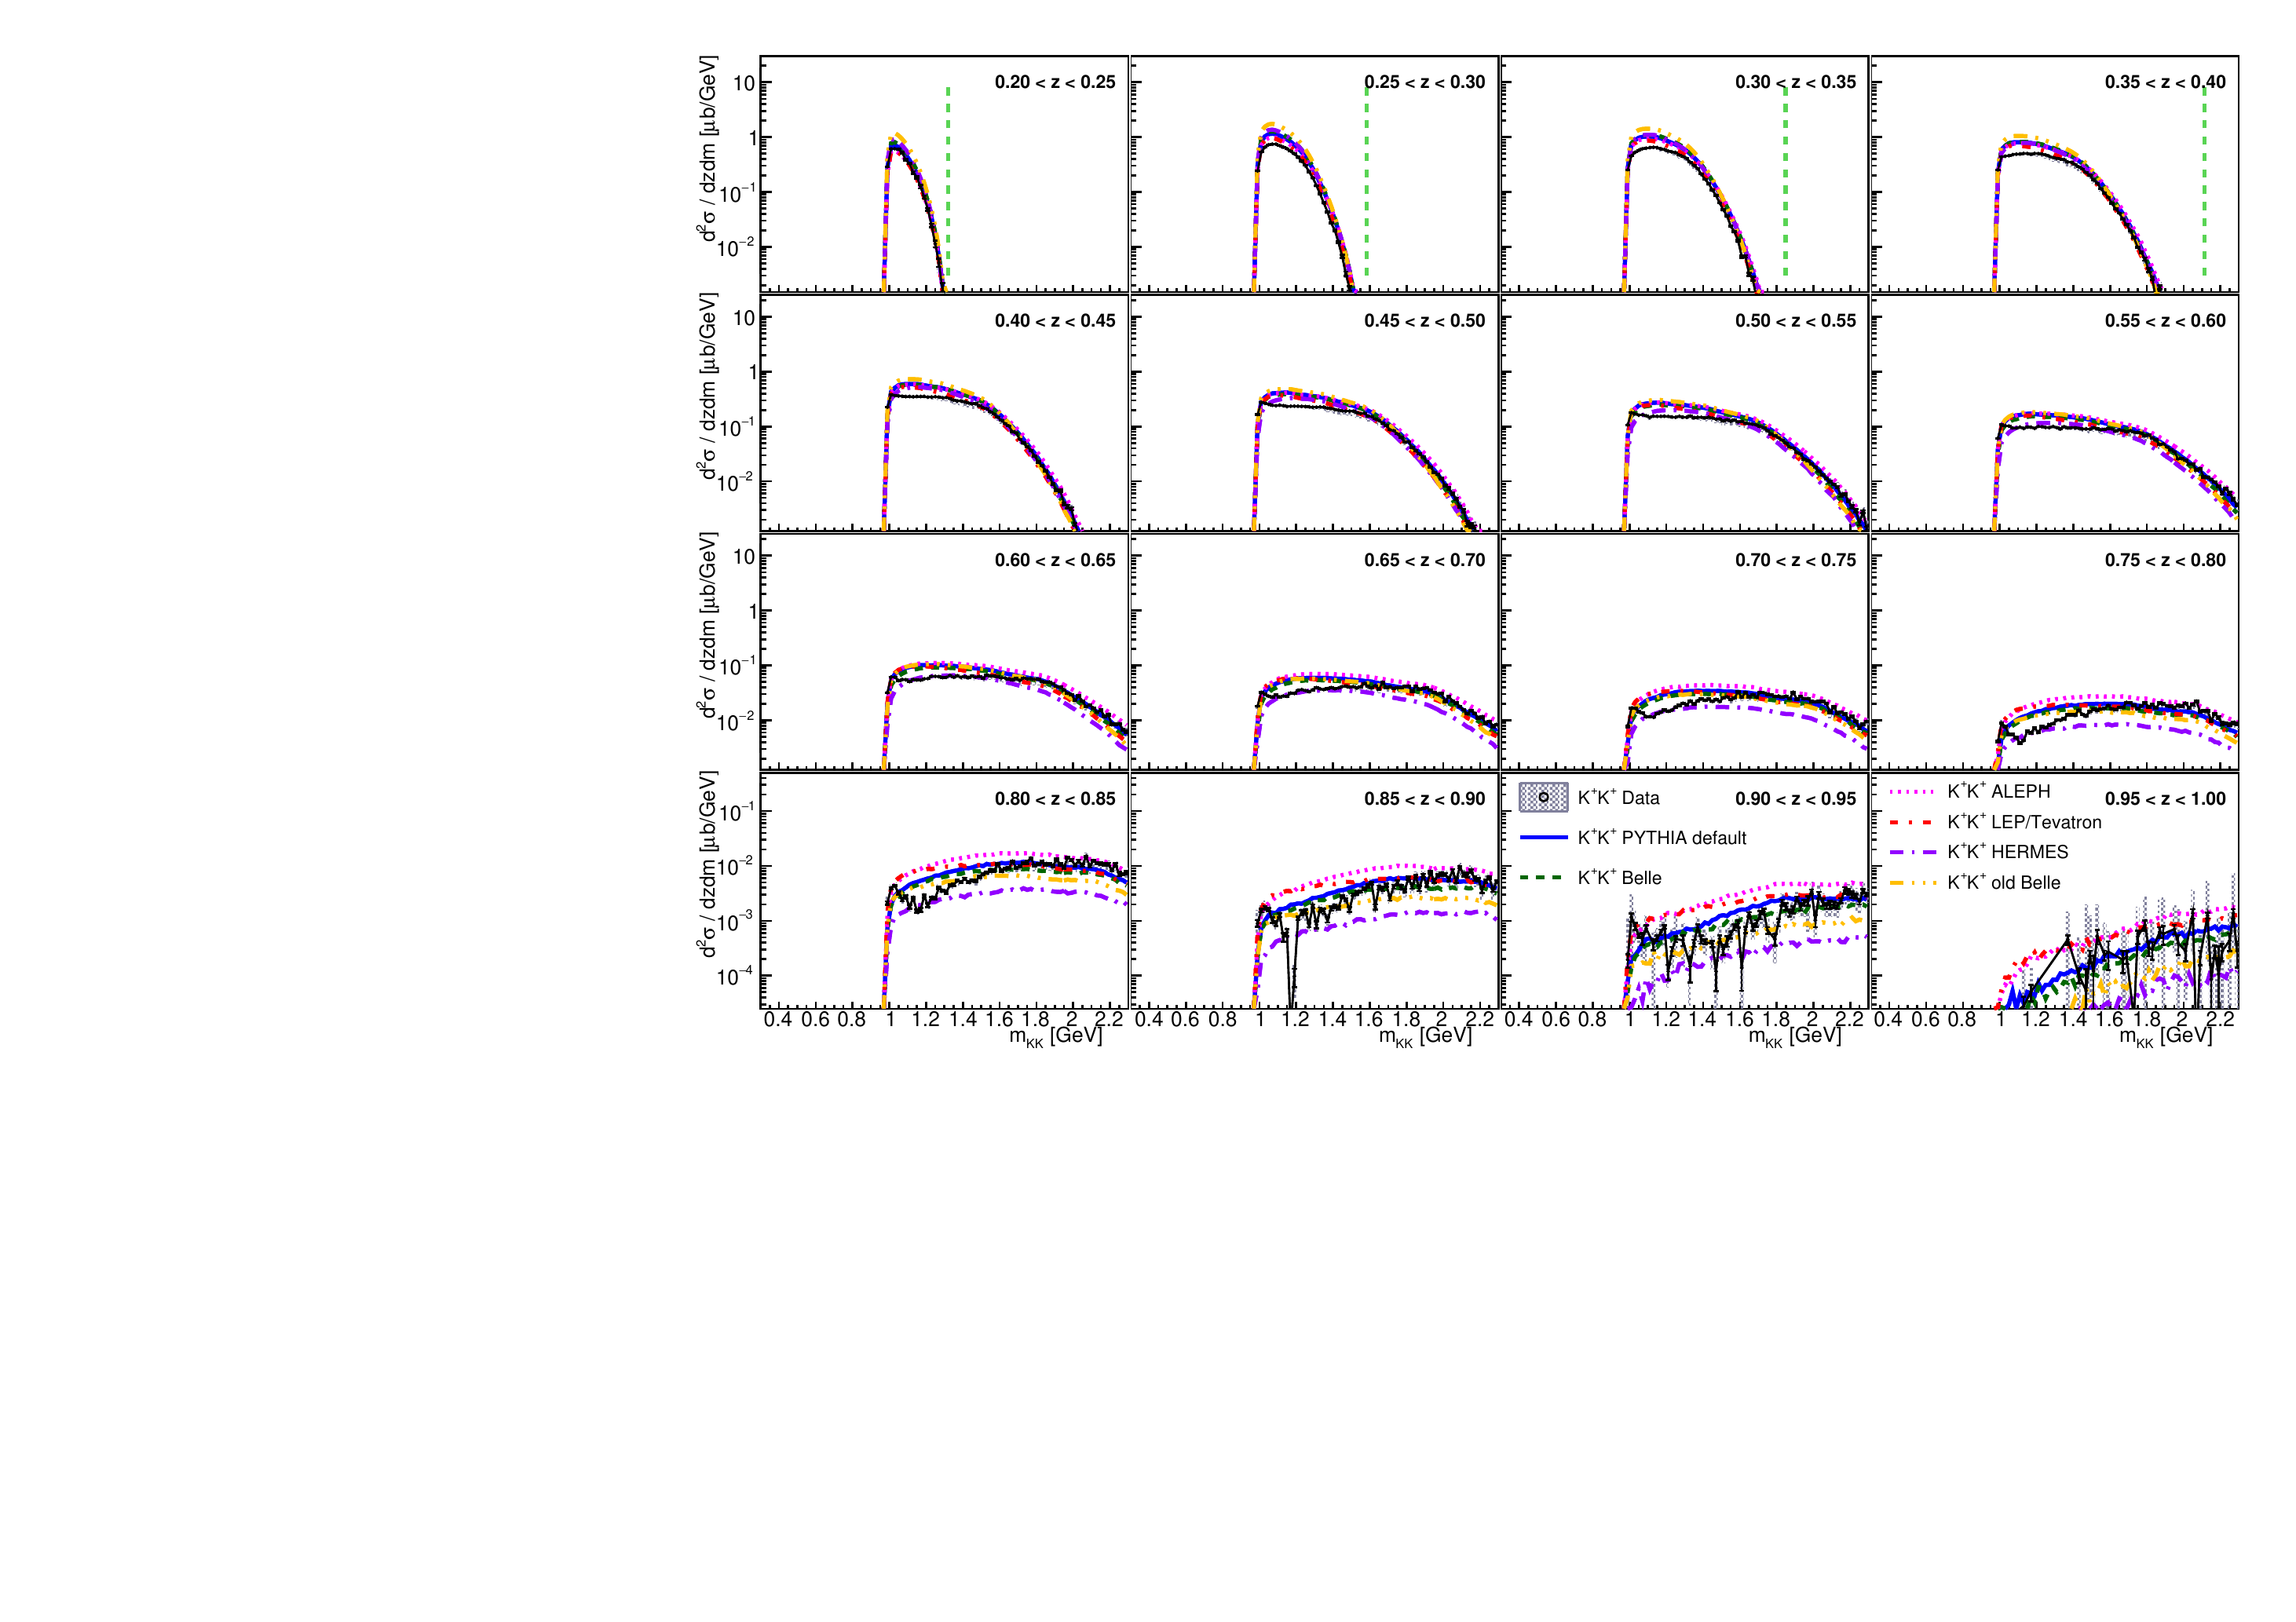}
\caption{\label{fig:allxsec_pid8192_mix1_c8_32518153}Differential cross sections for $K^+K^++\ c.c.$ pairs as a function of $m_{KK}$ in bins of $z$. Various {\sc Pythia} tunes are also displayed as described in the paper text. The vertical green dashed line corresponds to the kinematic limit. An overall 1.6\% scale uncertainty is not shown.}
\end{center}
\end{figure*}

\end{document}
